# Supplementary material for: Accurate Deep Learning-aided Density-free Strategy for Many-Body Dispersion-corrected Density Functional Theory
Source: arXiv:2203.15739 ancillary file (2022-05-06)
Supplement: Supplementary file 1 [file SI-ML_MBD2.pdf]

| Dimer nr | monomer A | Monomer B |
|---|---|---|
| 1 | -76.3881954 | -76.3881721 |
| 2 | -76.3882076 | -115.642028 |
| 3 | -76.3882076 | -95.7757617 |
| 4 | -76.3882143 | -248.341371 |
| 5 | -115.642023 | -115.642033 |
| 6 | -115.641928 | -95.7757644 |
| 7 | -115.641963 | -248.340949 |
| 8 | -115.642018 | -76.3881748 |
| 9 | -95.7757739 | -115.642046 |
| 10 | -95.7757945 | -95.7757513 |
| 11 | -95.7757494 | -248.341121 |
| 12 | -95.7757402 | -76.3882077 |
| 13 | -248.341051 | -115.642051 |
| 14 | -248.340931 | -95.7757558 |
| 15 | -248.341381 | -248.341316 |
| 16 | -248.341454 | -76.3881708 |
| 17 | -414.562122 | -414.562186 |
| 18 | -76.3882052 | -248.077581 |
| 19 | -115.641922 | -248.077578 |
| 20 | -228.945009 | -228.945011 |
| 21 | -209.074466 | -209.074468 |
| 22 | -228.944936 | -414.561914 |
| 23 | -209.074342 | -414.561895 |
| 24 | -232.038585 | -232.038582 |
| 25 | -248.077598 | -248.077598 |
| 26 | -414.562422 | -414.562422 |
| 27 | -232.038714 | -248.077599 |
| 28 | -232.038681 | -414.562783 |
| 29 | -248.077574 | -414.562704 |
| 30 | -232.03863 | -78.5079593 |
| 31 | -414.562788 | -78.5079894 |
| 32 | -414.562661 | -77.258356 |
| 33 | -248.077614 | -78.5079597 |
| 34 | -197.560184 | -197.560185 |
| 35 | -197.560187 | -197.56272 |
| 36 | -197.562688 | -197.562596 |
| 37 | -196.357712 | -197.562714 |
| 38 | -196.357589 | -196.357603 |
| 39 | -232.038709 | -196.357604 |
| 40 | -232.038715 | -197.562509 |
| 41 | -414.562885 | -197.560185 |
| 42 | -414.562896 | -196.357724 |
| 43 | -414.562812 | -197.562599 |
| 44 | -78.5079712 | -197.560171 |
| 45 | -77.2583784 | -197.560083 |
| 46 | -248.341429 | -197.560144 |
| 47 | -232.038644 | -232.038555 |
| 48 | -248.077637 | -248.077569 |

| Dimer nr | x1 |
|---|---|
| 1 | [illegible] |
| 2 | [illegible] |
| 3 | [illegible] |
| 4 | [illegible] |
| 5 | [illegible] |
| 6 | -211.428467 |
| 7 | -363.993536 |
| 8 | -192.037393 |
| 9 | -211.420787 |
| 10 | -191.555478 |
| 11 | -344.121095 |
| 12 | -172.174767 |
| 13 | -363.989231 |
| 14 | -344.125376 |
| 15 | -496.691532 |
| 16 | -324.735918 |
| 17 | -829.147045 |
| 18 | -324.476329 |
| 19 | -363.729898 |
| 20 | -457.917787 |
| 21 | -418.171132 |
| 22 | -643.534145 |
| 23 | -623.662352 |
| 24 | -464.066725 |
| 25 | -496.146586 |
| 26 | -829.121946 |
| 27 | -480.106601 |
| 28 | -646.593517 |
| 29 | -662.632499 |
| 30 | -310.54172 |
| 31 | -493.068264 |
| 32 | -491.819556 |
| 33 | -326.581644 |
| 34 | -395.116016 |
| 35 | -395.119936 |
| 36 | -395.123903 |
| 37 | -393.917025 |
| 38 | -392.712166 |
| 39 | -428.390795 |
| 40 | -429.597223 |
| 41 | -612.118112 |
| 42 | -610.915046 |
| 43 | -612.121812 |
| 44 | -276.066596 |
| 45 | -274.816454 |
| 46 | -445.898797 |
| 47 | -464.073716 |
| 48 | -496.153365 |

Total PBE PCSEG-3 energies (Hartree) f[illegible] dimes with MBD

| | | | | |
|---|---|---|---|---|
| 49 | -232.038716 | -248.077605 | 49 | -480.113418 |
| 50 | -232.038552 | -77.2583858 | 50 | -309.296533 |
| 51 | -77.2583939 | -77.2583939 | 51 | -154.518157 |
| 52 | -232.038635 | -228.946611 | 52 | -460.986918 |
| 53 | -232.038679 | -209.075078 | 53 | -441.115775 |
| 54 | -232.038714 | -76.3881322 | 54 | -308.428651 |
| 55 | -232.038701 | -115.642026 | 55 | -347.681637 |
| 56 | -232.038665 | -95.775746 | 56 | -327.813342 |
| 57 | -232.03859 | -248.341419 | 57 | -480.378237 |
| 58 | -248.07756 | -248.077559 | 58 | -496.156391 |
| 59 | -77.2583983 | -76.3881558 | 59 | -153.650336 |
| 60 | -77.2583296 | -228.946592 | 60 | -306.210644 |
| 61 | -197.56016 | -228.946634 | 61 | -426.505587 |
| 62 | -197.560153 | -209.075024 | 62 | -406.633844 |
| 63 | -232.038546 | -228.946606 | 63 | -460.982383 |
| 64 | -248.341323 | -78.5079391 | 64 | -326.849339 |
| 65 | -248.077613 | -77.2583883 | 65 | -325.34136 |
| 66 | -95.7757746 | -248.077599 | 66 | -343.854504 |

Hartree-to-kcalmol
627.5094736

for the
hout

| [illegible] | x3 | x4 | x5 | x6 | 7x | x8 |
|---|---|---|---|---|---|---|
| [illegible] | -152.784255 | -152.783944 | -152.783488 | -152.781899 | -152.779757 | -152.777749 |
| [illegible] | -192.038525 | -192.038244 | -192.037786 | -192.036107 | -192.033799 | -192.031626 |
| [illegible] | -172.175463 | -172.175 | -172.174345 | -172.172038 | -172.168855 | -172.165827 |
| [illegible] | -324.741283 | -324.740964 | -324.740423 | -324.738321 | -324.735222 | -324.731711 |
| [illegible] | -231.292246 | -231.292045 | -231.291645 | -231.290038 | -231.287722 | -231.285503 |
| -211.429239 | -211.429327 | -211.428988 | -211.428402 | -211.42615 | -211.422868 | -211.41966 |
| -363.994322 | -363.994471 | -363.99423 | -363.993743 | -363.991706 | -363.988169 | -363.98457 |
| -192.037902 | -192.037942 | -192.037697 | -192.037288 | -192.035765 | -192.03362 | -192.031583 |
| -211.421307 | -211.421459 | -211.421399 | -211.42122 | -211.420422 | -211.419303 | -211.418339 |
| -191.55628 | -191.556556 | -191.556512 | -191.556278 | -191.555196 | -191.55332 | -191.552058 |
| -344.122075 | -344.122511 | -344.122596 | -344.122435 | -344.120774 | -344.11868 | -344.117497 |
| -172.175405 | -172.175402 | -172.17501 | -172.174396 | -172.172118 | -172.16887 | -172.165787 |
| -363.990107 | -363.990448 | -363.990444 | -363.990226 | -363.989035 | -363.987038 | -363.984897 |
| -344.12633 | -344.126651 | -344.12656 | -344.126205 | -344.124446 | -344.121723 | -344.118864 |
| -496.69256 | -496.692964 | -496.692947 | -496.692653 | -496.691085 | -496.688447 | -496.685068 |
| -324.736545 | -324.73671 | -324.73659 | -324.736309 | -324.735094 | -324.733221 | -324.731294 |
| -829.148779 | -829.14913 | -829.148621 | -829.147588 | -829.143144 | -829.136317 | -829.129144 |
| -324.476817 | -324.476745 | -324.476323 | -324.475699 | -324.473475 | -324.470435 | -324.467608 |
| -363.730625 | -363.730716 | -363.730407 | -363.729854 | -363.727692 | -363.724531 | -363.721487 |
| -457.919682 | -457.919969 | -457.919195 | -457.917794 | -457.912258 | -457.903947 | -457.895452 |
| -418.17275 | -418.173028 | -418.172471 | -418.171402 | -418.167129 | -418.16068 | -418.153294 |
| -643.535976 | -643.536326 | -643.535707 | -643.534501 | -643.529416 | -643.521469 | -643.513007 |
| -623.664109 | -623.66453 | -623.664062 | -623.663032 | -623.658516 | -623.651201 | -623.64304 |
| -464.07137 | -464.07483 | -464.076357 | -464.07667 | -464.077587 | -464.077355 | -464.077243 |
| -496.150921 | -496.153728 | -496.155408 | -496.156006 | -496.1564 | -496.155925 | -496.155485 |
| -829.127078 | -829.129659 | -829.130766 | -829.130882 | -829.130036 | -829.127922 | -829.125943 |
| -480.111169 | -480.11437 | -480.116058 | -480.116399 | -480.11693 | -480.11648 | -480.116198 |
| -646.597673 | -646.600542 | -646.60244 | -646.603104 | -646.602836 | -646.601966 | -646.601465 |
| -662.6382 | -662.641314 | -662.643134 | -662.643736 | -662.643146 | -662.641869 | -662.640889 |
| -310.54377 | -310.545292 | -310.545987 | -310.546101 | -310.546573 | -310.546441 | -310.546473 |
| -493.070332 | -493.071688 | -493.072188 | -493.07231 | -493.072289 | -493.071621 | -493.071039 |
| -491.821725 | -491.822854 | -491.823292 | -491.823412 | -491.823064 | -491.822079 | -491.821294 |
| -326.583609 | -326.584863 | -326.585505 | -326.58574 | -326.585991 | -326.585748 | -326.585582 |
| -395.118625 | -395.120143 | -395.120961 | -395.121356 | -395.1215 | -395.121038 | -395.120593 |
| -395.121874 | -395.122935 | -395.123448 | -395.123669 | -395.12365 | -395.123267 | -395.12297 |
| -395.124951 | -395.125503 | -395.125772 | -395.125899 | -395.125875 | -395.125597 | -395.125386 |
| -393.919022 | -393.920141 | -393.920713 | -393.920982 | -393.921066 | -393.920741 | -393.920438 |
| -392.714075 | -392.715281 | -392.715895 | -392.716159 | -392.716166 | -392.715726 | -392.715384 |
| -428.393836 | -428.395719 | -428.396696 | -428.397031 | -428.397371 | -428.396877 | -428.396387 |
| -429.599604 | -429.601036 | -429.601615 | -429.601828 | -429.602162 | -429.601896 | -429.601571 |
| -612.121047 | -612.122869 | -612.123714 | -612.124012 | -612.124372 | -612.123606 | -612.123163 |
| -610.918191 | -610.91992 | -610.920782 | -610.921181 | -610.921482 | -610.920976 | -610.920541 |
| -612.124373 | -612.125737 | -612.126238 | -612.12647 | -612.126576 | -612.126011 | -612.125507 |
| -276.067769 | -276.068405 | -276.068715 | -276.068858 | -276.068779 | -276.068459 | -276.068196 |
| -274.817872 | -274.818643 | -274.819063 | -274.81924 | -274.819163 | -274.81883 | -274.818524 |
| -445.900899 | -445.902104 | -445.902715 | -445.902963 | -445.903106 | -445.902486 | -445.901866 |
| -464.076126 | -464.077439 | -464.078183 | -464.078481 | -464.078501 | -464.077962 | -464.07742 |
| -496.155323 | -496.156433 | -496.157039 | -496.157212 | -496.157068 | -496.15627 | -496.15556 |

| | | | | | | |
|---|---|---|---|---|---|---|
| -480.115896 | -480.117234 | -480.1179 | -480.118136 | -480.117975 | -480.117328 | -480.116641 |
| -309.298141 | -309.298848 | -309.299213 | -309.299283 | -309.298804 | -309.297929 | -309.297234 |
| -154.518604 | -154.518743 | -154.518708 | -154.518583 | -154.518066 | -154.517415 | -154.516954 |
| -460.988361 | -460.989042 | -460.989247 | -460.989196 | -460.988383 | -460.987056 | -460.985895 |
| -441.116892 | -441.11742 | -441.117573 | -441.117503 | -441.116791 | -441.115483 | -441.114159 |
| -308.429729 | -308.430222 | -308.430239 | -308.430133 | -308.429428 | -308.428385 | -308.427448 |
| -347.6831 | -347.683853 | -347.684196 | -347.68424 | -347.683495 | -347.682376 | -347.681376 |
| -327.814909 | -327.815778 | -327.816254 | -327.816367 | -327.816052 | -327.81525 | -327.814586 |
| -480.381253 | -480.382803 | -480.383555 | -480.383815 | -480.383144 | -480.381904 | -480.380763 |
| -496.158228 | -496.159161 | -496.159166 | -496.158838 | -496.157622 | -496.156326 | -496.155501 |
| -153.650738 | -153.650807 | -153.650685 | -153.650455 | -153.649564 | -153.648343 | -153.647243 |
| -306.211415 | -306.211577 | -306.211377 | -306.210983 | -306.209451 | -306.207418 | -306.20569 |
| -426.506732 | -426.507368 | -426.507656 | -426.50778 | -426.507705 | -426.50716 | -426.506767 |
| -406.635299 | -406.63607 | -406.636466 | -406.63666 | -406.636574 | -406.636007 | -406.635403 |
| -460.9848 | -460.986112 | -460.986807 | -460.98698 | -460.986945 | -460.986121 | -460.985477 |
| -326.850423 | -326.850996 | -326.851234 | -326.851268 | -326.850969 | -326.850142 | -326.849459 |
| -325.341823 | -325.341873 | -325.341678 | -325.341345 | -325.340097 | -325.338399 | -325.336878 |
| -343.855595 | -343.856189 | -343.856457 | -343.856488 | -343.855964 | -343.854914 | -343.853862 |

Dimers Interaction energies (kcal/mol) for PBE PCSEG-3 without MBD

| Dimer nr | x1 | [illegible] | x3 | x4 |
|---|---|---|---|---|
| 1 | -4.[illegible] | [illegible]19236 | -4.94954554 | -4.75446295 |
| 2 | -4.[illegible] | [illegible]01364 | -5.2019483 | -5.02565309 |
| 3 | -7.[illegible] | [illegible]3747 | -7.21217045 | -6.92159101 |
| 4 | -6[illegible] | [illegible]1351 | -7.3409416 | -7.14063888 |
| 5 | -4.[illegible] | [illegible]20276 | -5.13928401 | -5.01335817 |
| 6 | -6.76097996 | -7.24516157 | -7.30055189 | -7.08762538 |
| 7 | -6.66658968 | -7.15967909 | -7.25343026 | -7.10178845 |
| 8 | -4.51818223 | -4.83704853 | -4.86218047 | -4.70881961 |
| 9 | -1.86196782 | -2.18796489 | -2.28336698 | -2.2455136 |
| 10 | -2.46745705 | -2.97081873 | -3.1442262 | -3.11642226 |
| 11 | -2.65116791 | -3.2662613 | -3.539576 | -3.59316587 |
| 12 | -6.78911448 | -7.18910213 | -7.18769783 | -6.94137821 |
| 13 | -3.84603405 | -4.39618384 | -4.60981248 | -4.60773662 |
| 14 | -5.45229358 | -6.05097791 | -6.25244955 | -6.1954031 |
| 15 | -5.54415802 | -6.18958427 | -6.44284295 | -6.4321079 |
| 16 | -3.94889151 | -4.34242241 | -4.44592213 | -4.37087074 |
| 17 | -14.2681739 | -15.3557445 | -15.5764329 | -15.2569652 |
| 18 | -6.61528877 | -6.92181309 | -6.87633666 | -6.61178463 |
| 19 | -6.52539459 | -6.98115265 | -7.03833708 | -6.84446163 |
| 20 | -17.4237851 | -18.6124949 | -18.7928532 | -18.3072761 |
| 21 | -13.9295167 | -14.9447337 | -15.1192955 | -14.7698019 |
| 22 | -17.128136 | -18.2768614 | -18.4968302 | -18.1079705 |
| 23 | -16.3877732 | -17.4897925 | -17.7542725 | -17.4605847 |
| 24 | 6.552570201 | 3.637407107 | 1.466308541 | 0.508447583 |
| 25 | 5.402934379 | 2.682549159 | 0.920889794 | -0.13315506 |
| 26 | 1.817977463 | -1.4023155 | -3.02188363 | -3.71624765 |
| 27 | 6.094495815 | 3.228230707 | 1.219067737 | 0.160035875 |
| 28 | 4.986199627 | 2.378750802 | 0.578014413 | -0.61312313 |
| 29 | 4.881805269 | 1.304229997 | -0.65001849 | -1.79171381 |
| 30 | 3.055564761 | 1.769160238 | 0.813824315 | 0.377812222 |
| 31 | 1.577088185 | 0.279563001 | -0.571239 | -0.88499311 |
| 32 | 0.916828678 | -0.44418679 | -1.15244217 | -1.42782822 |
| 33 | 2.466118318 | 1.233129346 | 0.446214143 | 0.043200388 |
| 34 | 2.732048424 | 1.094534403 | 0.142430657 | -0.37087887 |
| 35 | 1.864209662 | 0.648486739 | -0.01751586 | -0.33924436 |
| 36 | 0.866288877 | 0.209057228 | -0.1377431 | -0.30648724 |
| 37 | 2.134810635 | 0.881571305 | 0.179061648 | -0.1794689 |
| 38 | 1.898737493 | 0.700734558 | -0.05564804 | -0.44125098 |
| 39 | 3.462417557 | 1.554211887 | 0.372643112 | -0.24067385 |
| 40 | 2.510482171 | 1.016707478 | 0.11830593 | -0.24518816 |
| 41 | 3.11178459 | 1.269561479 | 0.126521096 | -0.40350171 |
| 42 | 3.497041459 | 1.523682359 | 0.438743768 | -0.10226453 |
| 43 | 2.258041636 | 0.651275328 | -0.20458189 | -0.51941689 |
| 44 | 0.969807044 | 0.233795472 | -0.16507867 | -0.35944627 |
| 45 | 1.259754322 | 0.370377176 | -0.11368049 | -0.37726372 |
| 46 | 1.74195287 | 0.423271518 | -0.33296512 | -0.71652602 |
| 47 | 2.185371521 | 0.673424718 | -0.15075972 | -0.61771932 |
| 48 | 1.154646611 | -0.07399121 | -0.7702926 | -1.1505095 |

| | | | | |
|---|---|---|---|---|
| 49 | 1.821370406 | 0.266876014 | -0.5731942 | -0.99087731 |
| 50 | 0.254129414 | -0.75541981 | -1.19889174 | -1.42765283 |
| 51 | -0.8589777 | -1.13994808 | -1.22675943 | -1.20487517 |
| 52 | -1.04993567 | -1.95503927 | -2.38261626 | -2.51121466 |
| 53 | -1.26692148 | -1.96772193 | -2.2992552 | -2.39530664 |
| 54 | -1.13264964 | -1.80914483 | -2.11877953 | -2.12914429 |
| 55 | -0.57110735 | -1.48871753 | -1.96149873 | -2.1770601 |
| 56 | 0.67101847 | -0.31240333 | -0.85750563 | -1.15671149 |
| 57 | 1.111762864 | -0.78078249 | -1.75359242 | -2.22529913 |
| 58 | -0.79793038 | -1.95113284 | -2.53652331 | -2.53966306 |
| 59 | -2.37286376 | -2.62517603 | -2.66862002 | -2.59221729 |
| 60 | -3.59054432 | -4.0746409 | -4.1761676 | -4.0508426 |
| 61 | 0.757396593 | 0.038834114 | -0.36004423 | -0.54074368 |
| 62 | 0.836869852 | -0.07637512 | -0.55999912 | -0.80861003 |
| 63 | 1.737319277 | 0.220300065 | -0.60262057 | -1.03892765 |
| 64 | -0.04830217 | -0.72849489 | -1.0880297 | -1.23727631 |
| 65 | -3.36239964 | -3.65333449 | -3.68462494 | -3.56224798 |
| 66 | -0.7089789 | -1.39383942 | -1.76619576 | -1.9348533 |

| x5 | x6 | 7x | x8 |
|---|---|---|---|
| -4.46785879 | -3.47097798 | -2.12708963 | -0.86674294 |
| -4.73814024 | -3.68474059 | -2.2366226 | -0.87286587 |
| -6.51107714 | -5.06301896 | -3.06558816 | -1.16592622 |
| -6.80086798 | -5.4819734 | -3.53710141 | -1.33426919 |
| -4.76266431 | -3.75390129 | -2.30076794 | -0.90819835 |
| -6.72010168 | -5.30680112 | -3.24721168 | -1.23449223 |
| -6.79631201 | -5.51823284 | -3.29877143 | -1.04010034 |
| -4.45219145 | -3.49639851 | -2.15013548 | -0.87230255 |
| -2.13362483 | -1.63262861 | -0.93035778 | -0.32563274 |
| -2.96953648 | -2.29047904 | -1.11360624 | -0.32133034 |
| -3.49197896 | -2.44959474 | -1.13571703 | -0.39326395 |
| -6.55597695 | -5.12649656 | -3.0888072 | -1.1537585 |
| -4.47074992 | -3.72313249 | -2.47004025 | -1.12657322 |
| -5.97245137 | -4.86872308 | -3.1604381 | -1.36608461 |
| -6.24761277 | -5.26364428 | -3.60853 | -1.48831354 |
| -4.19458927 | -3.43200387 | -2.25655425 | -1.0472023 |
| -14.6089655 | -11.8197356 | -7.5359354 | -3.03503623 |
| -6.21993151 | -4.82427853 | -2.91705403 | -1.14270749 |
| -6.49781222 | -5.14099868 | -3.1572036 | -1.24743167 |
| -17.4277796 | -13.9543829 | -8.73882984 | -3.40847163 |
| -14.0988559 | -11.4175898 | -7.37057116 | -2.73570919 |
| -17.3510684 | -14.1606022 | -9.17362381 | -3.86371426 |
| -16.8142048 | -13.9801867 | -9.3900197 | -4.26911481 |
| 0.311774756 | -0.26371456 | -0.11783938 | -0.04753453 |
| -0.50841238 | -0.75562702 | -0.45727368 | -0.18163707 |
| -3.78946621 | -3.25868669 | -1.93202813 | -0.68976864 |
| -0.05365118 | -0.38697562 | -0.10467115 | 0.071947224 |
| -1.02970125 | -0.86162472 | -0.31528655 | -0.00111897 |
| -2.16948988 | -1.79919428 | -0.99829817 | -0.38305971 |
| 0.306601819 | 0.010043477 | 0.093354898 | 0.07327447 |
| -0.96177994 | -0.94846112 | -0.52932671 | -0.16422488 |
| -1.50309195 | -1.28450926 | -0.66626258 | -0.17354929 |
| -0.10441519 | -0.26161855 | -0.10956993 | -0.00536847 |
| -0.61902266 | -0.70912662 | -0.41961734 | -0.14030133 |
| -0.47832399 | -0.46631051 | -0.22555772 | -0.03958844 |
| -0.38571125 | -0.37087059 | -0.19621035 | -0.06371606 |
| -0.34831834 | -0.40131854 | -0.19749863 | -0.00703551 |
| -0.60697699 | -0.61093933 | -0.33480925 | -0.12033084 |
| -0.45074853 | -0.6643498 | -0.35400991 | -0.04661605 |
| -0.37892762 | -0.58869569 | -0.4215138 | -0.21780722 |
| -0.59079546 | -0.81669931 | -0.3360322 | -0.05779042 |
| -0.35242331 | -0.54104996 | -0.22378255 | 0.048935573 |
| -0.66464762 | -0.73109698 | -0.37675048 | -0.06062733 |
| -0.44967774 | -0.40013731 | -0.19887495 | -0.03376321 |
| -0.48840901 | -0.43975149 | -0.23082415 | -0.03901421 |
| -0.87217548 | -0.96160424 | -0.57304629 | -0.18398747 |
| -0.80469989 | -0.81714905 | -0.47917019 | -0.13882888 |
| -1.25940756 | -1.16886685 | -0.66839573 | -0.22246152 |

| | | | |
|---|---|---|---|
| -1.1386406 | -1.03774266 | -0.63181387 | -0.20079952 |
| -1.4719538 | -1.17097027 | -0.6222517 | -0.18587734 |
| -1.12641414 | -0.8021116 | -0.39344474 | -0.10395874 |
| -2.4788267 | -1.9686962 | -1.13601912 | -0.40760261 |
| -2.35082851 | -1.90455545 | -1.08342579 | -0.25247248 |
| -2.06297285 | -1.62042932 | -0.9656107 | -0.37774721 |
| -2.20440068 | -1.73660793 | -1.03440726 | -0.40710336 |
| -1.22762609 | -1.02989384 | -0.5262329 | -0.1099502 |
| -2.38825795 | -1.96771553 | -1.18904724 | -0.47356295 |
| -2.33383738 | -1.57054565 | -0.75702391 | -0.2396266 |
| -2.44792268 | -1.88850614 | -1.12259192 | -0.43255615 |
| -3.80350246 | -2.84244234 | -1.56631774 | -0.48226883 |
| -0.61873928 | -0.57182893 | -0.22965265 | 0.016925939 |
| -0.93031637 | -0.87626477 | -0.52041689 | -0.14121147 |
| -1.14722192 | -1.12529341 | -0.60830392 | -0.20407825 |
| -1.25867852 | -1.07115917 | -0.55217244 | -0.12334031 |
| -3.35297137 | -2.57007028 | -1.50469317 | -0.55004268 |
| -1.95390919 | -1.62528167 | -0.96642075 | -0.30638156 |

| Dimer nr | monomer A | Monomer B |
|---|---|---|
| 1 | -76.3872699 | -76.3873217 |
| 2 | -76.3872546 | -115.648047 |
| 3 | -76.3871489 | -95.7871216 |
| 4 | -76.3871836 | -248.354247 |
| 5 | -115.648068 | -115.64806 |
| 6 | -115.647863 | -95.7871148 |
| 7 | -115.647936 | -248.353957 |
| 8 | -115.648095 | -76.3873256 |
| 9 | -95.7871384 | -115.648116 |
| 10 | -95.787124 | -95.7870959 |
| 11 | -95.7870883 | -248.354115 |
| 12 | -95.7870889 | -76.3871395 |
| 13 | -248.35404 | -115.648088 |
| 14 | -248.353823 | -95.78708 |
| 15 | -248.354141 | -248.354202 |
| 16 | -248.354314 | -76.3873289 |
| 17 | -414.557593 | -414.557721 |
| 18 | -76.387156 | -248.092068 |
| 19 | -115.647866 | -248.092063 |
| 20 | -228.945248 | -228.945245 |
| 21 | -209.079951 | -209.079954 |
| 22 | -228.945172 | -414.557452 |
| 23 | -209.079854 | -414.557296 |
| 24 | -232.061117 | -232.061114 |
| 25 | -248.092018 | -248.092021 |
| 26 | -414.558134 | -414.558134 |
| 27 | -232.061202 | -248.092051 |
| 28 | -232.061147 | -414.558667 |
| 29 | -248.091935 | -414.558589 |
| 30 | -232.061181 | -78.5186559 |
| 31 | -414.55868 | -78.5186367 |
| 32 | -414.558571 | -77.2614646 |
| 33 | -248.092099 | -78.5186443 |
| 34 | -197.601676 | -197.601677 |
| 35 | -197.601676 | -197.604425 |
| 36 | -197.604399 | -197.604329 |
| 37 | -196.395698 | -197.604411 |
| 38 | -196.395601 | -196.395612 |
| 39 | -232.061189 | -196.395614 |
| 40 | -232.061208 | -197.604247 |
| 41 | -414.558707 | -197.601635 |
| 42 | -414.558711 | -196.395687 |
| 43 | -414.558664 | -197.6043 |
| 44 | -78.5186587 | -197.601667 |
| 45 | -77.2615308 | -197.601606 |
| 46 | -248.354356 | -197.601624 |
| 47 | -232.061136 | -232.061062 |
| 48 | -248.092034 | -248.091965 |

| Dimer nr | x1 |
|---|---|
| 1 | -152.782198 |
| 2 | -192.043147 |
| 3 | -172.185233 |
| 4 | -324.752906 |
| 5 | -231.303625 |
| 6 | -211.445572 |
| 7 | -364.01283 |
| 8 | -192.042681 |
| 9 | -211.438146 |
| 10 | -191.578083 |
| 11 | -344.145724 |
| 12 | -172.184969 |
| 13 | -364.008648 |
| 14 | -344.149651 |
| 15 | -496.717756 |
| 16 | -324.748206 |
| 17 | -829.139278 |
| 18 | -324.489497 |
| 19 | -363.750023 |
| 20 | -457.919917 |
| 21 | -418.18321 |
| 22 | -643.531484 |
| 23 | -623.664757 |
| 24 | -464.11215 |
| 25 | -496.175919 |
| 26 | -829.115069 |
| 27 | -480.143988 |
| 28 | -646.612968 |
| 29 | -662.643868 |
| 30 | -310.574925 |
| 31 | -493.075317 |
| 32 | -491.819137 |
| 33 | -326.60684 |
| 34 | -395.199311 |
| 35 | -395.203251 |
| 36 | -395.207196 |
| 37 | -393.996886 |
| 38 | -392.788247 |
| 39 | -428.451796 |
| 40 | -429.661907 |
| 41 | -612.156201 |
| 42 | -610.949526 |
| 43 | -612.159843 |
| 44 | -276.118829 |
| 45 | -274.861152 |
| 46 | -445.953738 |
| 47 | -464.11925 |
| 48 | -496.182741 |

| | | | | |
|---|---|---|---|---|
| 49 | -232.061181 | -248.092023 | 49 | -480.150934 |
| 50 | -232.061046 | -77.2615004 | 50 | -309.32274 |
| 51 | -77.2615305 | -77.2615305 | 51 | -154.524495 |
| 52 | -232.061076 | -228.947116 | 52 | -461.010646 |
| 53 | -232.06111 | -209.080862 | 53 | -441.14453 |
| 54 | -232.06117 | -76.3872355 | 54 | -308.450502 |
| 55 | -232.06114 | -115.648128 | 55 | -347.710528 |
| 56 | -232.061143 | -95.7871076 | 56 | -327.847515 |
| 57 | -232.061034 | -248.354328 | 57 | -480.414483 |
| 58 | -248.091918 | -248.091918 | 58 | -496.185509 |
| 59 | -77.2614878 | -76.387323 | 59 | -153.652819 |
| 60 | -77.2614084 | -228.947089 | 60 | -306.214654 |
| 61 | -197.601637 | -228.947178 | 61 | -426.547759 |
| 62 | -197.601624 | -209.080879 | 62 | -406.681403 |
| 63 | -232.061046 | -228.947105 | 63 | -461.006155 |
| 64 | -248.354296 | -78.518608 | 64 | -326.873244 |
| 65 | -248.092077 | -77.2614039 | 65 | -325.358899 |
| 66 | -95.7871145 | -248.092033 | 66 | -343.88028 |

Hartree-to-kcalmol
627.5094736

PBE0-PCSEG3

| x2 | x3 | x4 | x5 | x6 | 7x | x8 |
|---|---|---|---|---|---|---|
| -152.782542 | -152.782459 | -152.782122 | -152.781648 | -152.780046 | -152.777938 | -152.775989 |
| -192.043617 | -192.043596 | -192.04328 | -192.042799 | -192.041099 | -192.03882 | -192.036712 |
| -172.185631 | -172.185483 | -172.185005 | -172.184344 | -172.182054 | -172.17896 | -172.17608 |
| -324.753438 | -324.753396 | -324.753007 | -324.75241 | -324.750211 | -324.747069 | -324.743596 |
| -231.304223 | -231.304301 | -231.304062 | -231.303637 | -231.302006 | -231.299725 | -231.297581 |
| -211.446286 | -211.446332 | -211.445965 | -211.445368 | -211.443125 | -211.439928 | -211.436882 |
| -364.013518 | -364.013588 | -364.013279 | -364.01274 | -364.0106119 | -364.007053 | -364.003529 |
| -192.043138 | -192.043139 | -192.042866 | -192.042438 | -192.0409 | -192.038794 | -192.036821 |
| -211.438633 | -211.438765 | -211.438691 | -211.438504 | -211.4377213 | -211.436664 | -211.435768 |
| -191.578835 | -191.579075 | -191.579009 | -191.578761 | -191.577677 | -191.575889 | -191.57472 |
| -344.146617 | -344.146973 | -344.146988 | -344.146781 | -344.145027 | -344.142964 | -344.141829 |
| -172.185549 | -172.185507 | -172.185086 | -172.184453 | -172.182165 | -172.178989 | -172.176036 |
| -364.009449 | -364.009722 | -364.009659 | -364.009392 | -364.008108 | -364.006083 | -364.003966 |
| -344.150543 | -344.150809 | -344.150674 | -344.150288 | -344.148498 | -344.145806 | -344.143049 |
| -496.718685 | -496.719 | -496.718907 | -496.718549 | -496.716849 | -496.714135 | -496.710773 |
| -324.748778 | -324.748895 | -324.748735 | -324.748421 | -324.747153 | -324.745276 | -324.743372 |
| -829.140785 | -829.140952 | -829.140285 | -829.139118 | -829.13439 | -829.127401 | -829.120207 |
| -324.489967 | -324.489883 | -324.489457 | -324.488837 | -324.486651 | -324.483713 | -324.481012 |
| -363.750731 | -363.750805 | -363.75049 | -363.749937 | -363.747804 | -363.744749 | -363.741858 |
| -457.921435 | -457.921426 | -457.920426 | -457.918851 | -457.912985 | -457.904465 | -457.895941 |
| -418.184603 | -418.184706 | -418.184009 | -418.182832 | -418.178337 | -418.17174 | -418.164362 |
| -643.533017 | -643.533123 | -643.532307 | -643.530937 | -643.525531 | -643.517387 | -643.508874 |
| -623.666264 | -623.666478 | -623.665842 | -623.664671 | -623.65986 | -623.652351 | -623.644129 |
| -464.116651 | -464.119856 | -464.121278 | -464.121583 | -464.122394 | -464.122271 | -464.122263 |
| -496.180161 | -496.18278 | -496.184297 | -496.184824 | -496.185101 | -496.184677 | -496.184293 |
| -829.119812 | -829.121885 | -829.122769 | -829.122722 | -829.121561 | -829.119366 | -829.117419 |
| -480.148432 | -480.151422 | -480.152959 | -480.153266 | -480.153713 | -480.153349 | -480.153152 |
| -646.616863 | -646.619395 | -646.621068 | -646.62159 | -646.621174 | -646.620286 | -646.6198 |
| -662.649306 | -662.652017 | -662.653709 | -662.654145 | -662.653409 | -662.652129 | -662.651146 |
| -310.576935 | -310.578368 | -310.579012 | -310.579129 | -310.579609 | -310.579585 | -310.579697 |
| -493.077221 | -493.078415 | -493.07883 | -493.078891 | -493.078768 | -493.078114 | -493.077581 |
| -491.821141 | -491.822142 | -491.822483 | -491.822517 | -491.822042 | -491.821064 | -491.820319 |
| -326.608723 | -326.6099 | -326.610489 | -326.610692 | -326.610944 | -326.610787 | -326.610712 |
| -395.201695 | -395.203054 | -395.203735 | -395.204081 | -395.204164 | -395.203809 | -395.203504 |
| -395.205071 | -395.206041 | -395.206487 | -395.206686 | -395.206659 | -395.206357 | -395.206149 |
| -395.208196 | -395.208755 | -395.208993 | -395.209114 | -395.209141 | -395.208938 | -395.208801 |
| -393.998748 | -393.999768 | -394.000236 | -394.000499 | -394.000563 | -394.000311 | -394.000101 |
| -392.790021 | -392.791129 | -392.791678 | -392.791906 | -392.791933 | -392.791598 | -392.791368 |
| -428.454665 | -428.456367 | -428.457216 | -428.457501 | -428.457721 | -428.45727 | -428.45687 |
| -429.664139 | -429.665414 | -429.66594 | -429.666122 | -429.666338 | -429.666005 | -429.665723 |
| -612.158849 | -612.160403 | -612.161101 | -612.161353 | -612.161482 | -612.160811 | -612.160435 |
| -610.952402 | -610.953919 | -610.954645 | -610.954962 | -610.955151 | -610.954703 | -610.954342 |
| -612.162329 | -612.163494 | -612.163912 | -612.164082 | -612.164046 | -612.16352 | -612.163097 |
| -276.119921 | -276.120481 | -276.120737 | -276.12087 | -276.12079 | -276.120542 | -276.120359 |
| -274.862502 | -274.863214 | -274.863588 | -274.86375 | -274.863684 | -274.863419 | -274.863187 |
| -445.955585 | -445.956608 | -445.9571 | -445.957289 | -445.95732 | -445.956734 | -445.956228 |
| -464.121499 | -464.122672 | -464.123296 | -464.12352 | -464.123432 | -464.1229 | -464.122406 |
| -496.184573 | -496.185514 | -496.186016 | -496.186131 | -496.185854 | -496.185055 | -496.184361 |

| | | | | | | |
|---|---|---|---|---|---|---|
| -480.15325 | -480.154435 | -480.154989 | -480.155155 | -480.154864 | -480.154198 | -480.15355 |
| -309.324225 | -309.324834 | -309.325091 | -309.325079 | -309.32448 | -309.323586 | -309.322867 |
| -154.524925 | -154.525047 | -154.524999 | -154.524866 | -154.524344 | -154.523708 | -154.523257 |
| -461.011963 | -461.012525 | -461.01263 | -461.012492 | -461.011519 | -461.010089 | -461.008882 |
| -441.145579 | -441.146037 | -441.146119 | -441.145983 | -441.145157 | -441.143763 | -441.142439 |
| -308.4515 | -308.45198 | -308.451893 | -308.451821 | -308.451046 | -308.449977 | -308.449036 |
| -347.711926 | -347.712617 | -347.712889 | -347.712877 | -347.712104 | -347.710963 | -347.709955 |
| -327.84899 | -327.849776 | -327.850174 | -327.850236 | -327.84986 | -327.849086 | -327.848462 |
| -480.41727 | -480.418658 | -480.419255 | -480.419392 | -480.418612 | -480.417319 | -480.416163 |
| -496.18723 | -496.188038 | -496.187962 | -496.187576 | -496.186293 | -496.185011 | -496.184209 |
| -153.653174 | -153.653203 | -153.653048 | -153.652794 | -153.651861 | -153.650631 | -153.649533 |
| -306.215348 | -306.215437 | -306.21517 | -306.214721 | -306.213083 | -306.210998 | -306.209284 |
| -426.548792 | -426.549352 | -426.549598 | -426.549699 | -426.549581 | -426.549115 | -426.548803 |
| -406.682717 | -406.68339 | -406.683723 | -406.683866 | -406.683717 | -406.683189 | -406.682701 |
| -461.008364 | -461.009495 | -461.010069 | -461.01016 | -461.009932 | -461.009109 | -461.008483 |
| -326.874231 | -326.874725 | -326.874901 | -326.874894 | -326.874533 | -326.873735 | -326.873103 |
| -325.359337 | -325.359364 | -325.359152 | -325.358804 | -325.357546 | -325.355858 | -325.354368 |
| -343.881353 | -343.881922 | -343.88216 | -343.882164 | -343.88163 | -343.880617 | -343.87963 |

PBE0-PCSEG3

| Dimer nr | x1 | x2 | x3 | x4 |
|---|---|---|---|---|
| 1 | -4.77310896 | -4.98920326 | -4.93683867 | -4.72524373 |
| 2 | -4.9226242 | -5.21754129 | -5.20466084 | -5.00650847 |
| 3 | -6.87934174 | -7.12857006 | -7.03564256 | -6.73573915 |
| 4 | -7.20087779 | -7.53489669 | -7.50841974 | -7.26400317 |
| 5 | -4.7045971 | -5.07978576 | -5.12874775 | -4.97884754 |
| 6 | -6.64773634 | -7.0955869 | -7.12435677 | -6.89437511 |
| 7 | -6.86305379 | -7.29527002 | -7.33900279 | -7.14528371 |
| 8 | -4.55632991 | -4.84299462 | -4.84380988 | -4.67247583 |
| 9 | -1.81415474 | -2.11985533 | -2.20287263 | -2.15610448 |
| 10 | -2.42408064 | -2.89627933 | -3.04673828 | -3.00534719 |
| 11 | -2.83726011 | -3.39714892 | -3.62052773 | -3.6299634 |
| 12 | -6.73976933 | -7.10379956 | -7.07718048 | -6.81318179 |
| 13 | -4.09187162 | -4.59457824 | -4.76562804 | -4.72614816 |
| 14 | -5.48928401 | -6.04870168 | -6.21571395 | -6.131363 |
| 15 | -5.90673927 | -6.48962554 | -6.68698976 | -6.62855626 |
| 16 | -4.11822539 | -4.47686475 | -4.55040032 | -4.44991089 |
| 17 | -15.0375578 | -15.9833121 | -16.0878917 | -15.6693353 |
| 18 | -6.44624882 | -6.74118054 | -6.68879303 | -6.42128982 |
| 19 | -6.33420694 | -6.77827626 | -6.82514356 | -6.62703255 |
| 20 | -18.463611 | -19.4161347 | -19.4108879 | -18.7832657 |
| 21 | -14.6243767 | -15.4982264 | -15.5630032 | -15.1257537 |
| 22 | -18.1100559 | -19.0720734 | -19.1388936 | -18.6267674 |
| 23 | -17.3240282 | -18.269358 | -18.4036414 | -18.0045628 |
| 24 | 6.325930847 | 3.501820069 | 1.490760075 | 0.598195871 |
| 25 | 5.09519978 | 2.43339395 | 0.789770058 | -0.16198712 |
| 26 | 0.752450061 | -2.22383999 | -3.52473879 | -4.07911184 |
| 27 | 5.813959673 | 3.025167324 | 1.149330413 | 0.184799971 |
| 28 | 4.295740097 | 1.851251403 | 0.262326194 | -0.78708482 |
| 29 | 4.177024467 | 0.764444654 | -0.93663739 | -1.99791267 |
| 30 | 3.082186286 | 1.820676067 | 0.921792089 | 0.517280783 |
| 31 | 1.254971507 | 0.060433429 | -0.68871844 | -0.94913807 |
| 32 | 0.564242713 | -0.69335793 | -1.32125828 | -1.53566478 |
| 33 | 2.44952816 | 1.267657427 | 0.528805998 | 0.159678131 |
| 34 | 2.536269798 | 1.040124312 | 0.187466447 | -0.23989449 |
| 35 | 1.788817976 | 0.646571203 | 0.037691294 | -0.24179277 |
| 36 | 0.961490849 | 0.333636935 | -0.01688804 | -0.16629428 |
| 37 | 2.022343493 | 0.853928822 | 0.214304776 | -0.07970123 |
| 38 | 1.861612777 | 0.748332658 | 0.052728805 | -0.29145456 |
| 39 | 3.142283558 | 1.342125859 | 0.273976974 | -0.2588678 |
| 40 | 2.225983306 | 0.825557739 | 0.025664322 | -0.30464788 |
| 41 | 2.598885078 | 0.937065105 | -0.03791996 | -0.47618425 |
| 42 | 3.057184112 | 1.252457955 | 0.300352954 | -0.15514852 |
| 43 | 1.958288769 | 0.398506982 | -0.33272893 | -0.59458298 |
| 44 | 0.939632435 | 0.254532212 | -0.09692172 | -0.25782557 |
| 45 | 1.245562819 | 0.398634492 | -0.04846595 | -0.28287349 |
| 46 | 1.406126554 | 0.24710614 | -0.39469737 | -0.70357209 |
| 47 | 1.849487913 | 0.438068254 | -0.29777138 | -0.68967728 |
| 48 | 0.788995836 | -0.36070399 | -0.9513363 | -1.26590398 |

| | | | | |
|---|---|---|---|---|
| 49 | 1.424240745 | -0.02872192 | -0.77229266 | -1.12033935 |
| 50 | -0.12130172 | -1.05348405 | -1.43552914 | -1.59701538 |
| 51 | -0.89964289 | -1.16978986 | -1.24598243 | -1.2161485 |
| 52 | -1.54010365 | -2.36606036 | -2.71869189 | -2.78514288 |
| 53 | -1.60509462 | -2.26275599 | -2.55017547 | -2.60200311 |
| 54 | -1.31566033 | -1.94145903 | -2.24272714 | -2.18815591 |
| 55 | -0.79050763 | -1.66800966 | -2.10169928 | -2.27198948 |
| 56 | 0.461415058 | -0.46392804 | -0.95767722 | -1.20715296 |
| 57 | 0.550934869 | -1.1980244 | -2.06887928 | -2.44341364 |
| 58 | -1.04913667 | -2.12919781 | -2.63633842 | -2.58879473 |
| 59 | -2.51525495 | -2.7377747 | -2.75585645 | -2.65913622 |
| 60 | -3.86327795 | -4.29914339 | -4.35507388 | -4.18722426 |
| 61 | 0.662347231 | 0.014243085 | -0.33690444 | -0.49184513 |
| 62 | 0.689776046 | -0.13424749 | -0.55687538 | -0.76547063 |
| 63 | 1.25224705 | -0.13394127 | -0.84311583 | -1.20325387 |
| 64 | -0.21373989 | -0.8329348 | -1.1427137 | -1.25345651 |
| 65 | -3.39994604 | -3.67435204 | -3.691784 | -3.55864394 |
| 66 | -0.71090197 | -1.38424837 | -1.74104091 | -1.8904405 |

| x5 | x6 | 7x | x8 |
|---|---|---|---|
| -4.42787263 | -3.42297363 | -2.10011444 | -0.87656673 |
| -4.70464905 | -3.63800544 | -2.20779833 | -0.88506365 |
| -6.32100264 | -4.88412479 | -2.94279277 | -1.13563527 |
| -6.88975658 | -5.50984536 | -3.53823934 | -1.35855468 |
| -4.7123688 | -3.68873431 | -2.25744651 | -0.91204398 |
| -6.51967377 | -5.11247756 | -3.10595873 | -1.19461194 |
| -6.80663385 | -5.47143287 | -3.237883 | -1.02655461 |
| -4.40392681 | -3.43853731 | -2.11708343 | -0.87919901 |
| -2.03882453 | -1.54776046 | -0.88414723 | -0.32182495 |
| -2.84937243 | -2.16933457 | -1.04718568 | -0.31356956 |
| -3.50030827 | -2.3997831 | -1.1054392 | -0.39297668 |
| -6.416131 | -4.98044129 | -2.98714012 | -1.13448868 |
| -4.55818872 | -3.75257863 | -2.48177198 | -1.15341569 |
| -5.8887999 | -4.765556 | -3.0764698 | -1.34621816 |
| -6.40412662 | -5.33728729 | -3.63400312 | -1.5246961 |
| -4.25331939 | -3.45721676 | -2.27973953 | -1.08479357 |
| -14.9371659 | -11.9703622 | -7.58493586 | -3.07018962 |
| -6.03195025 | -4.66038215 | -2.81716124 | -1.12219201 |
| -6.28020762 | -4.94181287 | -3.02493402 | -1.21073636 |
| -17.7949409 | -14.1135275 | -8.76749773 | -3.41867142 |
| -14.3867545 | -11.5660083 | -7.42674831 | -2.79694276 |
| -17.7666672 | -14.3746068 | -9.26388565 | -3.92208506 |
| -17.2700437 | -14.2511274 | -9.53904115 | -4.37995488 |
| 0.406552909 | -0.10187629 | -0.02511506 | -0.02003111 |
| -0.49270431 | -0.66669054 | -0.40046073 | -0.1592806 |
| -4.04958727 | -3.32135142 | -1.94356075 | -0.72208883 |
| -0.00776763 | -0.28855157 | -0.05994454 | 0.063716496 |
| -1.11508659 | -0.8539676 | -0.29686877 | 0.008500745 |
| -2.27199312 | -1.80992451 | -1.00655475 | -0.38972342 |
| 0.444366692 | 0.142648779 | 0.157912383 | 0.087435288 |
| -0.98784116 | -0.91065838 | -0.50027766 | -0.16586845 |
| -1.55703618 | -1.25849453 | -0.64524076 | -0.17745842 |
| 0.032053937 | -0.12609062 | -0.02733036 | 0.019601702 |
| -0.45682476 | -0.50864293 | -0.28615781 | -0.09468704 |
| -0.36664036 | -0.34996693 | -0.16021497 | -0.03010891 |
| -0.24258192 | -0.25949983 | -0.13206175 | -0.046073 |
| -0.24430193 | -0.28489652 | -0.12661252 | 0.005161077 |
| -0.43487241 | -0.45177375 | -0.24158807 | -0.09675048 |
| -0.43771628 | -0.57602333 | -0.29255602 | -0.04166732 |
| -0.41910636 | -0.55413027 | -0.34519817 | -0.16829653 |
| -0.63415549 | -0.71509455 | -0.29393723 | -0.05836208 |
| -0.35411922 | -0.47273671 | -0.1914938 | 0.035286364 |
| -0.70152566 | -0.67881233 | -0.34861195 | -0.08343554 |
| -0.34099586 | -0.29086865 | -0.13553194 | -0.02052929 |
| -0.38464668 | -0.34303289 | -0.17696508 | -0.03118521 |
| -0.82216492 | -0.84160215 | -0.47356289 | -0.15633407 |
| -0.83002103 | -0.77459895 | -0.44105532 | -0.13097566 |
| -1.3382936 | -1.1646493 | -0.66305475 | -0.22774421 |

| | | | |
|---|---|---|---|
| -1.22402795 | -1.04183973 | -0.62408208 | -0.21740455 |
| -1.58922227 | -1.21343245 | -0.65214311 | -0.20099687 |
| -1.13272356 | -0.80497675 | -0.40587275 | -0.12272899 |
| -2.69860267 | -2.08786803 | -1.19031607 | -0.43306933 |
| -2.51684261 | -1.99830461 | -1.12345343 | -0.29286972 |
| -2.14313756 | -1.65648338 | -0.98623963 | -0.3951963 |
| -2.26437296 | -1.77955493 | -1.0632294 | -0.43076561 |
| -1.2462313 | -1.01003341 | -0.52419305 | -0.13318945 |
| -2.52912868 | -2.0395921 | -1.22824061 | -0.50278933 |
| -2.34631032 | -1.54135052 | -0.73682238 | -0.23339098 |
| -2.49921731 | -1.91407332 | -1.14211023 | -0.45316143 |
| -3.90572338 | -2.87769595 | -1.56958443 | -0.49386797 |
| -0.55494246 | -0.48074618 | -0.18819047 | 0.007393442 |
| -0.85566966 | -0.76202705 | -0.43094188 | -0.1245083 |
| -1.26087487 | -1.11738196 | -0.60125787 | -0.20859413 |
| -1.24917257 | -1.02240476 | -0.52157075 | -0.12529111 |
| -3.33993957 | -2.55052681 | -1.49168904 | -0.55636477 |
| -1.89313785 | -1.55789574 | -0.92228117 | -0.30330074 |

DNN-MBD (different beta values)

REFERENCE CCSD(T)

CCSD(T) CBS REFERENCE INTER. ENERGIES kcal/mol

| Dimer nr | x1 | [illegible] | x3 | x4 | x5 | x6 |
|---|---|---|---|---|---|---|
| 1 | [illegible] | [illegible]4.884 | -4.894 | -4.723 | -4.451 | -3.457 |
| 2 | [illegible] | -5.55 | -5.569 | -5.381 | -5.076 | -3.944 |
| 3 | [illegible] | -6.87 | -6.875 | -6.648 | -6.284 | -4.919 |
| 4 | [illegible] | [illegible]8.055 | -8.075 | -7.843 | -7.462 | -5.994 |
| 5 | -5.279 | -5.691 | -5.745 | -5.578 | -5.283 | -4.141 |
| 6 | -6.972 | -7.472 | -7.54 | -7.335 | -6.967 | -5.503 |
| 7 | -7.629 | -8.14 | -8.22 | -8.024 | -7.66 | -6.182 |
| 8 | -4.587 | -4.952 | -4.997 | -4.847 | -4.586 | -3.589 |
| 9 | -2.814 | -3.041 | -3.035 | -2.896 | -2.687 | -1.976 |
| 10 | -3.696 | -4.093 | -4.152 | -4.008 | -3.752 | -2.793 |
| 11 | -4.949 | -5.356 | -5.406 | -5.236 | -4.939 | -3.209 |
| 12 | -6.747 | -7.203 | -7.245 | -7.029 | -6.657 | -5.222 |
| 13 | -5.673 | -6.107 | -6.18 | -6.027 | -5.741 | -4.604 |
| 14 | -6.812 | -7.341 | -7.451 | -7.291 | -6.966 | -5.611 |
| 15 | -8.015 | -8.531 | -8.624 | -8.445 | -8.098 | -6.657 |
| 16 | -4.695 | -5.061 | -5.118 | -4.983 | -4.74 | -3.793 |
| 17 | -15.7 | -16.898 | -17.182 | -16.864 | -16.169 | -13.15 |
| 18 | -6.392 | -6.804 | -6.834 | -6.624 | -6.273 | -4.931 |
| 19 | -6.783 | -7.307 | -7.404 | -7.226 | -6.882 | -5.479 |
| 20 | -17.449 | -18.787 | -19.09 | -18.724 | -17.938 | -14.558 |
| 21 | -14.926 | -16.026 | -16.26 | -15.935 | -15.262 | -12.418 |
| 22 | -17.902 | -19.185 | -19.491 | -19.152 | -18.406 | -15.137 |
| 23 | -17.697 | -18.889 | -19.19 | -18.898 | -18.224 | -15.208 |
| 24 | -0.225 | -2.069 | -2.736 | -2.799 | -2.578 | -1.538 |
| 25 | -1.321 | -3.168 | -3.825 | -3.855 | -3.58 | -2.356 |
| 26 | -7.855 | -9.498 | -9.821 | -9.429 | -8.685 | -6.072 |
| 27 | -0.725 | -2.69 | -3.369 | -3.398 | -3.128 | -1.97 |
| 28 | -3.531 | -5.216 | -5.705 | -5.549 | -5.077 | -3.292 |
| 29 | -3.74 | -6.173 | -6.814 | -6.581 | -5.971 | -3.866 |
| 30 | -0.259 | -1.125 | -1.412 | -1.401 | -1.256 | -0.689 |
| 31 | -2.567 | -3.237 | -3.378 | -3.237 | -2.959 | -1.99 |
| 32 | -2.793 | -3.563 | -3.737 | -3.591 | -3.291 | -2.225 |
| 33 | -0.885 | -1.622 | -1.861 | -1.83 | -1.668 | -1.027 |
| 34 | -2.856 | -3.62 | -3.774 | -3.613 | -3.304 | -2.235 |
| 35 | -1.852 | -2.492 | -2.611 | -2.484 | -2.254 | -1.496 |
| 36 | -1.454 | -1.735 | -1.772 | -1.684 | -1.537 | -1.048 |
| 37 | -1.607 | -2.25 | -2.405 | -2.325 | -2.138 | -1.467 |
| 38 | -2.237 | -2.842 | -2.997 | -2.86 | -2.595 | -1.713 |
| 39 | -2.156 | -3.239 | -3.569 | -3.47 | -3.167 | -2.065 |
| 40 | -1.863 | -2.675 | -2.894 | -2.804 | -2.568 | -1.703 |
| 41 | -3.827 | -4.692 | -4.839 | -4.6 | -4.079 | -2.443 |
| 42 | -3.049 | -3.968 | -4.132 | -3.919 | -3.539 | -2.294 |
| 43 | -2.868 | -3.599 | -3.7 | -3.489 | -3.145 | -2.045 |
| 44 | -1.656 | -1.971 | -1.989 | -1.862 | -1.674 | -1.09 |
| 45 | -1.134 | -1.631 | -1.749 | -1.676 | -1.519 | -0.977 |
| 46 | -3.751 | -4.205 | -4.244 | -4.048 | -3.73 | -2.628 |

| | | | | | | |
|---|---|---|---|---|---|---|
| 47 | -1.643 | -2.578 | -2.866 | -2.816 | -2.604 | -1.767 |
| 48 | -2.526 | -3.307 | -3.533 | -3.453 | -3.218 | -2.292 |
| 49 | -2.087 | -3.041 | -3.324 | -3.257 | -3.02 | -2.098 |
| 50 | -1.869 | -2.646 | -2.864 | -2.791 | -2.58 | -1.785 |
| 51 | -1.207 | -1.47 | -1.523 | -1.462 | -1.346 | -0.933 |
| 52 | -3.968 | -4.58 | -4.704 | -4.55 | -4.25 | -3.126 |
| 53 | -3.787 | -4.265 | -4.358 | -4.225 | -3.967 | -2.973 |
| 54 | -2.804 | -3.213 | -3.268 | -3.132 | -2.901 | -2.102 |
| 55 | -3.453 | -4.047 | -4.187 | -4.065 | -3.804 | -2.8 |
| 56 | -2.512 | -3.087 | -3.231 | -3.119 | -2.863 | -1.95 |
| 57 | -3.746 | -4.955 | -5.28 | -5.144 | -4.782 | -3.414 |
| 58 | -2.804 | -3.819 | -4.146 | -3.885 | -3.446 | -2.181 |
| 59 | -2.515 | -2.797 | -2.847 | -2.759 | -2.596 | -1.981 |
| 60 | -4.284 | -4.781 | -4.86 | -4.693 | -4.39 | -3.255 |
| 61 | -2.7 | -2.901 | -2.879 | -2.73 | -2.515 | -1.788 |
| 62 | -3.152 | -3.501 | -3.505 | -3.321 | -3.043 | -2.116 |
| 63 | -2.734 | -3.6 | -3.801 | -3.652 | -3.338 | -2.236 |
| 64 | -2.6 | -2.949 | -2.988 | -2.854 | -2.631 | -1.856 |
| 65 | -3.535 | -3.91 | -3.99 | -3.887 | -3.679 | -2.843 |
| 66 | -3.445 | -3.875 | -3.966 | -3.85 | -3.618 | -2.713 |

| **Beta=0.70** | | | | | | |
|---|---|---|---|---|---|---|
| 1 | 0.00196898 | 0.000680071 | 0.00157067 | 0.00383416 | 0.00856103 | 0.0425532 |
| 2 | 0.556436 | 0.574009 | 0.590823 | 0.610738 | 0.635682 | 0.735889 |
| 3 | 0.797311 | 0.823476 | 0.848517 | 0.874186 | 0.90026 | 0.973946 |
| 4 | 2.54982 | 2.57744 | 2.60883 | 2.64232 | 2.67812 | 2.80849 |
| 5 | 1.1288 | 1.17329 | 1.22038 | 1.26975 | 1.31936 | 1.465 |
| 6 | 1.06403 | 1.1405 | 1.21151 | 1.27867 | 1.34377 | 1.53273 |
| 7 | 2.87788 | 2.95022 | 3.0275 | 3.10873 | 3.18788 | 3.40994 |
| 8 | 0.69833 | 0.708437 | 0.722302 | 0.73954 | 0.75801 | 0.823792 |
| 9 | 1.14669 | 1.23512 | 1.32187 | 1.40574 | 1.48591 | 1.70356 |
| 10 | 1.07634 | 1.16735 | 1.25674 | 1.34541 | 1.43584 | 1.69423 |
| 11 | 2.48802 | 2.62736 | 2.75932 | 2.88908 | 3.01744 | 3.56633 |
| 12 | 0.67632 | 0.692522 | 0.710905 | 0.733228 | 0.760741 | 0.85864 |
| 13 | 2.76605 | 2.86647 | 2.96748 | 3.06897 | 3.1652 | 3.43165 |
| 14 | 2.70002 | 2.8313 | 2.95436 | 3.06937 | 3.17679 | 3.4914 |
| 15 | 4.33845 | 4.48806 | 4.63231 | 4.77266 | 4.9121 | 5.31532 |
| 16 | 2.78626 | 2.81664 | 2.85039 | 2.88503 | 2.91895 | 3.02213 |
| 17 | 8.06606 | 8.19858 | 8.33717 | 8.47098 | 8.59088 | 8.91454 |
| 18 | 4.66619 | 4.70315 | 4.73955 | 4.78184 | 4.83082 | 4.98354 |
| 19 | 5.01418 | 5.10743 | 5.18698 | 5.2603 | 5.33612 | 5.58662 |
| 20 | 1.71208 | 1.77478 | 1.84376 | 1.91558 | 1.98914 | 2.20943 |
| 21 | 1.84681 | 1.92836 | 2.0086 | 2.09045 | 2.17194 | 2.41455 |
| 22 | 4.94726 | 5.04227 | 5.14172 | 5.23869 | 5.33036 | 5.58453 |
| 23 | 4.95138 | 5.05205 | 5.15131 | 5.24877 | 5.3423 | 5.61655 |

| | | | | | | |
|---|---|---|---|---|---|---|
| 24 | 5.90646 | 6.73702 | 7.54401 | 8.28209 | 8.90366 | 10.201 |
| 25 | 4.77874 | 5.54242 | 6.26629 | 6.9304 | 7.53198 | 8.85665 |
| 26 | 3.14783 | 3.90731 | 4.65015 | 5.32936 | 5.93938 | 7.4576 |
| 27 | 5.29542 | 6.11214 | 6.87888 | 7.59678 | 8.23237 | 9.5363 |
| 28 | 4.4196 | 5.17134 | 5.90958 | 6.61856 | 7.25614 | 8.72679 |
| 29 | 3.75635 | 4.62522 | 5.43795 | 6.189 | 6.85699 | 8.39132 |
| 30 | 3.86111 | 4.26804 | 4.65 | 5.00425 | 5.32688 | 6.03691 |
| 31 | 2.94445 | 3.30192 | 3.65234 | 3.98642 | 4.2916 | 5.02329 |
| 32 | 2.84203 | 3.1488 | 3.44961 | 3.73345 | 3.9973 | 4.6467 |
| 33 | 3.32887 | 3.69994 | 4.05041 | 4.36165 | 4.65298 | 5.35529 |
| 34 | 5.46993 | 6.17216 | 6.78464 | 7.34238 | 7.82546 | 8.89978 |
| 35 | 7.26181 | 7.80812 | 8.31092 | 8.73217 | 9.07927 | 9.78313 |
| 36 | 8.63163 | 9.0272 | 9.37395 | 9.65623 | 9.88762 | 10.3554 |
| 37 | 8.12248 | 8.71419 | 9.21239 | 9.61782 | 9.94921 | 10.6145 |
| 38 | 8.10335 | 8.67959 | 9.25707 | 9.7621 | 10.1714 | 10.9999 |
| 39 | 7.14057 | 7.83727 | 8.46575 | 9.0309 | 9.51466 | 10.5614 |
| 40 | 7.74531 | 8.29807 | 8.75959 | 9.18458 | 9.54617 | 10.3083 |
| 41 | 4.7976 | 5.46483 | 6.08965 | 6.67132 | 7.30233 | 8.67485 |
| 42 | 6.0061 | 6.70515 | 7.35645 | 7.94527 | 8.45615 | 9.59931 |
| 43 | 6.62599 | 7.16176 | 7.66834 | 8.12421 | 8.50898 | 9.35513 |
| 44 | 3.89034 | 4.21522 | 4.51554 | 4.78495 | 5.0377 | 5.57142 |
| 45 | 3.66242 | 3.95896 | 4.23633 | 4.4803 | 4.69777 | 5.19685 |
| 46 | 4.09784 | 4.5627 | 5.00912 | 5.42145 | 5.80406 | 6.76508 |
| 47 | 8.38161 | 8.86999 | 9.30325 | 9.66948 | 9.99762 | 10.6789 |
| 48 | 7.37449 | 7.75893 | 8.1161 | 8.44252 | 8.74775 | 9.39818 |
| 49 | 7.76685 | 8.24583 | 8.67093 | 9.04078 | 9.37163 | 10.0758 |
| 50 | 4.27676 | 4.53823 | 4.79267 | 5.03951 | 5.2736 | 5.74222 |
| 51 | 0.297134 | 0.383187 | 0.468763 | 0.551218 | 0.627107 | 0.787394 |
| 52 | 5.03951 | 5.31632 | 5.56394 | 5.79003 | 5.99097 | 6.52139 |
| 53 | 5.44144 | 5.63838 | 5.8358 | 6.02735 | 6.20294 | 6.64412 |
| 54 | 4.67939 | 4.84361 | 4.98898 | 5.11034 | 5.2225 | 5.52133 |
| 55 | 4.29916 | 4.5944 | 4.86979 | 5.12559 | 5.34349 | 5.88874 |
| 56 | 4.38254 | 4.69688 | 4.99632 | 5.27836 | 5.53034 | 6.12629 |
| 57 | 5.07509 | 5.61923 | 6.11038 | 6.53103 | 6.87193 | 7.75718 |
| 58 | 8.60814 | 8.78964 | 9.06059 | 9.30776 | 9.51502 | 9.97214 |
| 59 | 0.264338 | 0.279607 | 0.298487 | 0.319363 | 0.341054 | 0.411119 |
| 60 | 0.907094 | 0.998409 | 1.09874 | 1.2003 | 1.29951 | 1.56559 |
| 61 | 3.92477 | 4.24317 | 4.53754 | 4.82088 | 5.08083 | 5.72248 |
| 62 | 3.63326 | 4.00272 | 4.35351 | 4.68119 | 4.9701 | 5.68914 |
| 63 | 3.97361 | 4.38301 | 4.79431 | 5.17883 | 5.52131 | 6.30484 |
| 64 | 2.09176 | 2.3084 | 2.51972 | 2.72416 | 2.90855 | 3.3842 |
| 65 | 4.8569 | 4.93974 | 5.01671 | 5.09336 | 5.16755 | 5.36769 |
| 66 | 4.05146 | 4.26754 | 4.47959 | 4.68523 | 4.88185 | 5.37218 |

| 7x | x8 |
|---|---|
| -2.108 | -0.871 |
| -2.385 | -0.951 |
| -2.977 | -1.14 |
| -3.832 | -1.436 |
| -2.524 | -1.009 |
| -3.349 | -1.274 |
| -3.648 | -1.096 |
| -2.199 | -0.907 |
| -1.1 | -0.393 |
| -1.307 | -0.387 |
| -1.401 | -0.455 |
| -3.153 | -1.195 |
| -2.946 | -1.303 |
| -3.553 | -1.489 |
| -4.415 | -1.774 |
| -2.449 | -1.133 |
| -8.354 | -3.333 |
| -3.011 | -1.186 |
| -3.381 | -1.331 |
| -9.207 | -3.592 |
| -7.997 | -2.999 |
| -9.859 | -4.146 |
| -10.229 | -4.653 |
| -0.487 | -0.063 |
| -0.96 | -0.236 |
| -3.096 | -0.992 |
| -0.721 | -0.145 |
| -1.364 | -0.251 |
| -1.776 | -0.532 |
| -0.174 | 0.009 |
| -0.932 | -0.254 |
| -1.042 | -0.273 |
| -0.366 | -0.046 |
| -1.05 | -0.27 |
| -0.698 | -0.184 |
| -0.504 | -0.135 |
| -0.706 | -0.188 |
| -0.791 | -0.204 |
| -0.895 | -0.189 |
| -0.765 | -0.187 |
| -0.976 | -0.213 |
| -1.017 | -0.247 |
| -0.92 | -0.229 |
| -0.492 | -0.12 |
| -0.421 | -0.097 |
| -1.188 | -0.286 |

| | |
|---|---|
| -0.828 | -0.224 |
| -1.178 | -0.371 |
| -1.049 | -0.333 |
| -0.889 | -0.271 |
| -0.461 | -0.135 |
| -1.699 | -0.554 |
| -1.645 | -0.481 |
| -1.156 | -0.416 |
| -1.528 | -0.517 |
| -0.94 | -0.261 |
| -1.803 | -0.618 |
| -1.01 | -0.275 |
| -1.169 | -0.458 |
| -1.772 | -0.557 |
| -0.784 | -0.168 |
| -1.043 | -0.273 |
| -1.02 | -0.262 |
| -0.877 | -0.189 |
| -1.67 | -0.616 |
| -1.503 | -0.494 |

| | | **Beta=0.72** | | | | |
|---|---|---|---|---|---|---|
| 0.120958 | 0.200593 | 1 | -0.404131 | -0.40013 | -0.387787 | -0.370593 |
| 0.891835 | 1.03702 | 2 | -0.849771 | -0.802631 | -0.75625 | -0.704914 |
| 1.09917 | 1.23846 | 3 | -0.762892 | -0.720575 | -0.676462 | -0.62739 |
| 3.03969 | 3.32853 | 4 | -1.32316 | -1.2606 | -1.19 | -1.11579 |
| 1.69192 | 1.89337 | 5 | -1.19789 | -1.11074 | -1.01979 | -0.927038 |
| 1.79752 | 2.06489 | 6 | -1.55081 | -1.42127 | -1.30182 | -1.18975 |
| 3.78527 | 4.18217 | 7 | -1.90251 | -1.77204 | -1.636 | -1.49811 |
| 0.949355 | 1.06797 | 8 | -0.663478 | -0.632072 | -0.592231 | -0.546651 |
| 1.92817 | 2.11451 | 9 | -1.34022 | -1.1878 | -1.0458 | -0.916921 |
| 2.06684 | 2.30261 | 10 | -1.81097 | -1.63642 | -1.47135 | -1.31553 |
| 4.10686 | 4.38603 | 11 | -2.61118 | -2.3649 | -2.14019 | -1.93004 |
| 1.01466 | 1.20903 | 12 | -0.981435 | -0.942458 | -0.896545 | -0.841471 |
| 3.77395 | 4.10255 | 13 | -1.92202 | -1.75656 | -1.59248 | -1.43289 |
| 3.89268 | 4.27141 | 14 | -2.30125 | -2.08879 | -1.89209 | -1.71254 |
| 5.81328 | 6.37803 | 15 | -2.84844 | -2.61895 | -2.4014 | -2.19293 |
| 3.19042 | 3.35913 | 16 | -0.897594 | -0.837906 | -0.771942 | -0.705147 |
| 9.4266 | 10.0092 | 17 | -2.96326 | -2.77067 | -2.56438 | -2.36553 |
| 5.16479 | 5.33354 | 18 | -1.03011 | -0.969292 | -0.909617 | -0.838968 |
| 5.89276 | 6.16348 | 19 | -1.64349 | -1.50206 | -1.38425 | -1.27721 |
| 2.57219 | 3.05489 | 20 | -2.21883 | -2.12269 | -2.01488 | -1.89951 |
| 2.78554 | 3.2706 | 21 | -2.26767 | -2.13281 | -1.99641 | -1.8548 |
| 6.00107 | 6.5365 | 22 | -2.52348 | -2.38268 | -2.23332 | -2.08711 |
| 6.05626 | 6.59661 | 23 | -2.63023 | -2.47716 | -2.32313 | -2.16998 |

| | | | | | | |
|---|---|---|---|---|---|---|
| 11.2249 | 11.6739 | 24 | -7.02281 | -5.78903 | -4.68627 | -3.75643 |
| 9.94682 | 10.4619 | 25 | -7.06708 | -5.90741 | -4.8943 | -4.02543 |
| 8.98772 | 9.99408 | 26 | -9.06248 | -7.81314 | -6.66951 | -5.6944 |
| 10.5931 | 11.07 | 27 | -7.11921 | -5.88927 | -4.83013 | -3.90467 |
| 10.0799 | 10.8328 | 28 | -8.20454 | -7.00679 | -5.91758 | -4.93987 |
| 9.6358 | 10.2855 | 29 | -8.47024 | -7.02945 | -5.80417 | -4.76126 |
| 6.57134 | 6.84261 | 30 | -3.86615 | -3.1869 | -2.6075 | -2.11585 |
| 5.67353 | 6.0717 | 31 | -4.15292 | -3.54819 | -3.0032 | -2.52062 |
| 5.22973 | 5.57853 | 32 | -3.70726 | -3.16786 | -2.67944 | -2.25167 |
| 5.91374 | 6.22911 | 33 | -3.81254 | -3.18801 | -2.64652 | -2.20799 |
| 9.89358 | 10.5209 | 34 | -6.23355 | -5.21503 | -4.3963 | -3.7184 |
| 10.415 | 10.8081 | 35 | -4.168 | -3.46091 | -2.85319 | -2.35943 |
| 10.778 | 11.0534 | 36 | -2.72958 | -2.27124 | -1.87817 | -1.56925 |
| 11.2002 | 11.5703 | 37 | -3.9487 | -3.22406 | -2.64629 | -2.188 |
| 11.7041 | 12.1302 | 38 | -4.61373 | -3.89932 | -3.21805 | -2.65204 |
| 11.3935 | 11.8993 | 39 | -5.56593 | -4.61049 | -3.81318 | -3.14657 |
| 10.944 | 11.3399 | 40 | -4.16487 | -3.42604 | -2.85962 | -2.37458 |
| 9.75063 | 10.368 | 41 | -6.86952 | -5.86729 | -4.99617 | -4.24173 |
| 10.5143 | 11.1132 | 42 | -6.20831 | -5.20751 | -4.33765 | -3.59882 |
| 10.1052 | 10.5809 | 43 | -4.89868 | -4.12815 | -3.43928 | -2.85633 |
| 6.02832 | 6.30585 | 44 | -2.9866 | -2.51112 | -2.10396 | -1.76451 |
| 5.60265 | 5.83235 | 45 | -2.71712 | -2.2555 | -1.86262 | -1.54461 |
| 7.79939 | 8.47072 | 46 | -5.57718 | -4.84723 | -4.19573 | -3.63033 |
| 11.3058 | 11.6557 | 47 | -3.9708 | -3.26821 | -2.69259 | -2.23809 |
| 10.0451 | 10.4397 | 48 | -3.82296 | -3.25407 | -2.763 | -2.34103 |
| 10.7055 | 11.0601 | 49 | -4.02869 | -3.32597 | -2.75624 | -2.29668 |
| 6.11888 | 6.32954 | 50 | -2.63193 | -2.2066 | -1.83235 | -1.49838 |
| 0.91841 | 0.992536 | 51 | -0.915275 | -0.765445 | -0.633549 | -0.518211 |
| 7.06164 | 7.4099 | 52 | -3.0387 | -2.60139 | -2.23846 | -1.93492 |
| 7.11278 | 7.48263 | 53 | -2.69353 | -2.37835 | -2.07763 | -1.80397 |
| 5.78426 | 5.9543 | 54 | -1.68286 | -1.39917 | -1.1762 | -1.01038 |
| 6.42018 | 6.76314 | 55 | -3.12678 | -2.65866 | -2.25526 | -1.90989 |
| 6.66575 | 6.98676 | 56 | -3.29146 | -2.79891 | -2.36524 | -1.98862 |
| 8.53457 | 9.02325 | 57 | -4.97834 | -4.14576 | -3.44892 | -2.89649 |
| 10.3188 | 10.5065 | 58 | -2.51516 | -2.21979 | -1.80402 | -1.45434 |
| 0.515177 | 0.595427 | 59 | -0.565991 | -0.523714 | -0.47391 | -0.423017 |
| 1.86708 | 2.08807 | 60 | -1.74099 | -1.54896 | -1.35808 | -1.18216 |
| 6.43447 | 6.89953 | 61 | -3.69409 | -3.2219 | -2.81169 | -2.4398 |
| 6.40108 | 6.91703 | 62 | -4.19954 | -3.62428 | -3.11847 | -2.67898 |
| 7.01701 | 7.43387 | 63 | -4.4325 | -3.77738 | -3.16736 | -2.63691 |
| 3.90622 | 4.23959 | 64 | -2.7854 | -2.42279 | -2.09656 | -1.8039 |
| 5.57828 | 5.73441 | 65 | -1.21389 | -1.08463 | -0.965505 | -0.85083 |
| 5.90942 | 6.31732 | 66 | -3.05573 | -2.70893 | -2.38674 | -2.08818 |

| | | | | | | |
|---|---|---|---|---|---|---|
| | | | **Beta=0.74** | | | |
| -0.348415 | -0.257958 | -0.126896 | -0.0370505 | 1 | -0.35051 | -0.35001 |
| -0.646788 | -0.45583 | -0.232458 | -0.0734693 | 2 | -0.763879 | -0.727285 |
| -0.574345 | -0.428675 | -0.234656 | -0.0713397 | 3 | -0.6866 | -0.650204 |
| -1.03942 | -0.79694 | -0.451883 | -0.108607 | 4 | -1.19982 | -1.14917 |
| -0.837722 | -0.606953 | -0.315823 | -0.104444 | 5 | -1.1091 | -1.03548 |
| -1.08137 | -0.779548 | -0.428596 | -0.138204 | 6 | -1.4379 | -1.32467 |
| -1.36718 | -1.02794 | -0.547678 | -0.122229 | 7 | -1.77822 | -1.6654 |
| -0.501178 | -0.368122 | -0.184444 | -0.0558651 | 8 | -0.594253 | -0.570854 |
| -0.800689 | -0.512479 | -0.269307 | -0.0750804 | 9 | -1.26748 | -1.13334 |
| -1.16499 | -0.780637 | -0.324293 | -0.0782531 | 10 | -1.67671 | -1.52777 |
| -1.73348 | -0.994252 | -0.382213 | -0.101851 | 11 | -2.45834 | -2.24303 |
| -0.776272 | -0.571985 | -0.327284 | -0.0960972 | 12 | -0.876235 | -0.845773 |
| -1.28683 | -0.920121 | -0.51553 | -0.174508 | 13 | -1.81946 | -1.67292 |
| -1.54823 | -1.10084 | -0.605967 | -0.209123 | 14 | -2.16627 | -1.9774 |
| -1.99129 | -1.44558 | -0.85377 | -0.257056 | 15 | -2.71391 | -2.50698 |
| -0.6419 | -0.473929 | -0.258293 | -0.0809958 | 16 | -0.831608 | -0.781565 |
| -2.19179 | -1.73467 | -1.03677 | -0.373655 | 17 | -2.78261 | -2.60787 |
| -0.756046 | -0.506953 | -0.267896 | -0.0897858 | 18 | -0.951158 | -0.898093 |
| -1.16602 | -0.805324 | -0.428496 | -0.150582 | 19 | -1.55039 | -1.42356 |
| -1.77827 | -1.40858 | -0.856719 | -0.279719 | 20 | -2.0512 | -1.96469 |
| -1.71238 | -1.30467 | -0.778263 | -0.220746 | 21 | -2.08883 | -1.97115 |
| -1.94866 | -1.56274 | -0.960328 | -0.323329 | 22 | -2.35234 | -2.22497 |
| -2.0233 | -1.60393 | -0.979786 | -0.345873 | 23 | -2.44928 | -2.31219 |

| | | | | | | |
|---|---|---|---|---|---|---|
| -3.01624 | -1.59982 | -0.543139 | -0.106889 | 24 | -6.76444 | -5.6307 |
| -3.27639 | -1.76425 | -0.628792 | -0.125548 | 25 | -6.78155 | -5.71946 |
| -4.87591 | -3.01566 | -1.33979 | -0.346858 | 26 | -8.61255 | -7.49607 |
| -3.12798 | -1.67139 | -0.578447 | -0.113018 | 27 | -6.84441 | -5.71583 |
| -4.11609 | -2.39142 | -0.951555 | -0.221555 | 28 | -7.84245 | -6.75944 |
| -3.89765 | -2.11414 | -0.809622 | -0.178049 | 29 | -8.05246 | -6.7637 |
| -1.7013 | -0.882054 | -0.331081 | -0.0660082 | 30 | -3.67305 | -3.06617 |
| -2.10792 | -1.21451 | -0.510537 | -0.114852 | 31 | -3.9351 | -3.39554 |
| -1.88482 | -1.0742 | -0.449611 | -0.103647 | 32 | -3.49657 | -3.01991 |
| -1.82416 | -0.981341 | -0.398528 | -0.0822763 | 33 | -3.61469 | -3.05849 |
| -3.13943 | -1.92177 | -0.866372 | -0.260844 | 34 | -6.04325 | -5.10012 |
| -1.96658 | -1.22348 | -0.555357 | -0.170678 | 35 | -4.07977 | -3.40664 |
| -1.32258 | -0.841371 | -0.395296 | -0.120703 | 36 | -2.69494 | -2.24854 |
| -1.82935 | -1.14772 | -0.538299 | -0.173891 | 37 | -3.88917 | -3.19071 |
| -2.20413 | -1.3409 | -0.60712 | -0.184587 | 38 | -4.53875 | -3.84997 |
| -2.60217 | -1.48012 | -0.644869 | -0.140055 | 39 | -5.43496 | -4.53963 |
| -1.96626 | -1.16449 | -0.529627 | -0.133743 | 40 | -4.08136 | -3.38486 |
| -3.46734 | -1.90945 | -0.806227 | -0.191316 | 41 | -6.62796 | -5.70832 |
| -2.99718 | -1.72043 | -0.796079 | -0.203829 | 42 | -6.01643 | -5.08771 |
| -2.38816 | -1.42457 | -0.638652 | -0.171112 | 43 | -4.71891 | -4.00859 |
| -1.46387 | -0.861614 | -0.374514 | -0.105116 | 44 | -2.89002 | -2.44925 |
| -1.2796 | -0.715845 | -0.29727 | -0.0721971 | 45 | -2.61571 | -2.19449 |
| -3.1399 | -2.00013 | -0.890517 | -0.231053 | 46 | -5.36825 | -4.70474 |
| -1.84933 | -1.12458 | -0.470147 | -0.122265 | 47 | -3.84207 | -3.19715 |
| -1.96642 | -1.23799 | -0.544993 | -0.146217 | 48 | -3.68499 | -3.16144 |
| -1.90661 | -1.13776 | -0.476935 | -0.122395 | 49 | -3.89434 | -3.24565 |
| -1.20141 | -0.666687 | -0.278839 | -0.0667974 | 50 | -2.51501 | -2.12995 |
| -0.420103 | -0.234076 | -0.0972738 | -0.0248677 | 51 | -0.870461 | -0.7366 |
| -1.68712 | -1.07287 | -0.478885 | -0.139854 | 52 | -2.92219 | -2.5259 |
| -1.56915 | -1.03102 | -0.513939 | -0.13696 | 53 | -2.57133 | -2.28757 |
| -0.871362 | -0.505201 | -0.224504 | -0.0537539 | 54 | -1.6018 | -1.34926 |
| -1.63957 | -1.01354 | -0.454942 | -0.123391 | 55 | -3.01212 | -2.58721 |
| -1.6785 | -0.986171 | -0.417501 | -0.0937975 | 56 | -3.16062 | -2.71276 |
| -2.48165 | -1.47034 | -0.657912 | -0.173328 | 57 | -4.78812 | -4.02822 |
| -1.18664 | -0.6457 | -0.275042 | -0.087082 | 58 | -2.37949 | -2.11587 |
| -0.37538 | -0.252466 | -0.115748 | -0.0310845 | 59 | -0.506872 | -0.474271 |
| -1.02501 | -0.662256 | -0.314065 | -0.0842759 | 60 | -1.61917 | -1.45712 |
| -2.11101 | -1.36289 | -0.613183 | -0.158448 | 61 | -3.5797 | -3.14428 |
| -2.3144 | -1.47673 | -0.710342 | -0.209573 | 62 | -4.05077 | -3.52646 |
| -2.194 | -1.27408 | -0.536787 | -0.123024 | 63 | -4.23926 | -3.64689 |
| -1.55919 | -0.987198 | -0.412362 | -0.0830932 | 64 | -2.66027 | -2.33509 |
| -0.74354 | -0.475949 | -0.235933 | -0.0739059 | 65 | -1.14215 | -1.02725 |
| -1.81382 | -1.1918 | -0.585419 | -0.174088 | 66 | -2.90294 | -2.59181 |

| | | | | | | Beta=0.75 |
|---|---|---|---|---|---|---|
| -0.342792 | -0.331594 | -0.315762 | -0.242808 | -0.125089 | -0.0368822 | 1 |
| -0.69115 | -0.650169 | -0.602411 | -0.437012 | -0.229583 | -0.0727728 | 2 |
| -0.613085 | -0.572336 | -0.528525 | -0.405182 | -0.228709 | -0.0704773 | 3 |
| -1.09173 | -1.03086 | -0.967354 | -0.757415 | -0.440806 | -0.109358 | 4 |
| -0.95808 | -0.878309 | -0.800396 | -0.591748 | -0.314843 | -0.104359 | 5 |
| -1.22 | -1.12146 | -1.0259 | -0.755532 | -0.424252 | -0.137405 | 6 |
| -1.54683 | -1.42537 | -1.30946 | -1.00066 | -0.543797 | -0.123146 | 7 |
| -0.540195 | -0.50408 | -0.467149 | -0.353219 | -0.183471 | -0.0561453 | 8 |
| -1.0064 | -0.889112 | -0.781637 | -0.509626 | -0.267963 | -0.0752429 | 9 |
| -1.38507 | -1.24824 | -1.11401 | -0.761062 | -0.322586 | -0.0782018 | 10 |
| -2.04409 | -1.85542 | -1.67636 | -0.981091 | -0.383041 | -0.102039 | 11 |
| -0.809774 | -0.766018 | -0.713315 | -0.541273 | -0.318736 | -0.0952508 | 12 |
| -1.52688 | -1.38336 | -1.25053 | -0.907737 | -0.515343 | -0.175464 | 13 |
| -1.80192 | -1.64057 | -1.49187 | -1.07834 | -0.603602 | -0.208813 | 14 |
| -2.30993 | -2.12007 | -1.93486 | -1.42387 | -0.851287 | -0.259435 | 15 |
| -0.725879 | -0.668955 | -0.61428 | -0.463381 | -0.258005 | -0.0813578 | 16 |
| -2.42251 | -2.24411 | -2.08728 | -1.66899 | -1.01938 | -0.374091 | 17 |
| -0.84584 | -0.783946 | -0.711252 | -0.4901 | -0.265225 | -0.0880034 | 18 |
| -1.31706 | -1.2196 | -1.11823 | -0.787768 | -0.427639 | -0.149471 | 19 |
| -1.86872 | -1.76712 | -1.6612 | -1.33844 | -0.837972 | -0.281534 | 20 |
| -1.8533 | -1.73137 | -1.60856 | -1.25024 | -0.763289 | -0.221081 | 21 |
| -2.09094 | -1.96031 | -1.83686 | -1.49156 | -0.938834 | -0.324941 | 22 |
| -2.17548 | -2.04056 | -1.9109 | -1.53511 | -0.959657 | -0.346623 | 23 |

| | | | | | | |
|---|---|---|---|---|---|---|
| -4.59612 | -3.70934 | -2.99302 | -1.59552 | -0.547458 | -0.107773 | 24 |
| -4.77446 | -3.95011 | -3.23289 | -1.75878 | -0.633081 | -0.12673 | 25 |
| -6.45606 | -5.55321 | -4.78242 | -2.99438 | -1.34876 | -0.350476 | 26 |
| -4.72078 | -3.84165 | -3.09609 | -1.66775 | -0.583019 | -0.114567 | 27 |
| -5.75651 | -4.84165 | -4.05861 | -2.38278 | -0.961752 | -0.224167 | 28 |
| -5.64031 | -4.66611 | -3.8451 | -2.11003 | -0.817548 | -0.180269 | 29 |
| -2.53666 | -2.07593 | -1.68104 | -0.882518 | -0.33357 | -0.066612 | 30 |
| -2.90009 | -2.45307 | -2.06488 | -1.20591 | -0.512873 | -0.115803 | 31 |
| -2.5799 | -2.18761 | -1.84458 | -1.06928 | -0.451798 | -0.104414 | 32 |
| -2.56543 | -2.15531 | -1.79175 | -0.978871 | -0.399152 | -0.0831695 | 33 |
| -4.32621 | -3.67106 | -3.11018 | -1.91862 | -0.874673 | -0.262594 | 34 |
| -2.81995 | -2.34075 | -1.9564 | -1.21813 | -0.558547 | -0.171409 | 35 |
| -1.86451 | -1.56031 | -1.31592 | -0.83591 | -0.396157 | -0.121143 | 36 |
| -2.62755 | -2.17919 | -1.82477 | -1.1424 | -0.53861 | -0.172604 | 37 |
| -3.18955 | -2.63357 | -2.19228 | -1.33326 | -0.606905 | -0.1837 | 38 |
| -3.77645 | -3.1279 | -2.5931 | -1.48311 | -0.645691 | -0.141425 | 39 |
| -2.83897 | -2.36359 | -1.96388 | -1.16777 | -0.530089 | -0.134769 | 40 |
| -4.89401 | -4.1764 | -3.43076 | -1.90892 | -0.808129 | -0.193411 | 41 |
| -4.26721 | -3.56031 | -2.97621 | -1.72583 | -0.799765 | -0.205608 | 42 |
| -3.3647 | -2.81137 | -2.36151 | -1.42409 | -0.644295 | -0.174155 | 43 |
| -2.06524 | -1.73974 | -1.44815 | -0.858642 | -0.377785 | -0.105865 | 44 |
| -1.82775 | -1.52492 | -1.26881 | -0.716304 | -0.299173 | -0.0726107 | 45 |
| -4.10168 | -3.57015 | -3.10165 | -1.99501 | -0.897372 | -0.233235 | 46 |
| -2.65294 | -2.21549 | -1.83744 | -1.11847 | -0.470907 | -0.122898 | 47 |
| -2.70138 | -2.30012 | -1.94033 | -1.22478 | -0.54387 | -0.147121 | 48 |
| -2.70797 | -2.26656 | -1.88889 | -1.13011 | -0.477673 | -0.123545 | 49 |
| -1.7837 | -1.46924 | -1.18621 | -0.665007 | -0.278368 | -0.0670033 | 50 |
| -0.615887 | -0.508028 | -0.414826 | -0.233874 | -0.0979183 | -0.0248755 | 51 |
| -2.19063 | -1.90367 | -1.66392 | -1.0639 | -0.484446 | -0.14112 | 52 |
| -2.01362 | -1.76038 | -1.53916 | -1.02085 | -0.513618 | -0.13771 | 53 |
| -1.14477 | -0.98783 | -0.852785 | -0.50232 | -0.224969 | -0.0540663 | 54 |
| -2.21398 | -1.88801 | -1.62689 | -1.01449 | -0.460595 | -0.12424 | 55 |
| -2.3108 | -1.95425 | -1.65377 | -0.981111 | -0.418012 | -0.0951778 | 56 |
| -3.38025 | -2.85667 | -2.45534 | -1.4675 | -0.660613 | -0.17484 | 57 |
| -1.7389 | -1.41468 | -1.16071 | -0.639175 | -0.274379 | -0.0862286 | 58 |
| -0.434888 | -0.393499 | -0.353542 | -0.24444 | -0.114998 | -0.0309842 | 59 |
| -1.29171 | -1.13556 | -0.992941 | -0.651976 | -0.312909 | -0.0846562 | 60 |
| -2.76019 | -2.40721 | -2.09264 | -1.36363 | -0.618289 | -0.159535 | 61 |
| -3.05673 | -2.64137 | -2.29173 | -1.47482 | -0.71744 | -0.211059 | 62 |
| -3.08541 | -2.58889 | -2.1682 | -1.27545 | -0.539364 | -0.124601 | 63 |
| -2.03671 | -1.7643 | -1.53249 | -0.979293 | -0.414856 | -0.0837228 | 64 |
| -0.920476 | -0.816539 | -0.718126 | -0.467702 | -0.233917 | -0.0732214 | 65 |
| -2.29865 | -2.02355 | -1.76875 | -1.17599 | -0.583656 | -0.173211 | 66 |

| | | | | | | |
|---|---|---|---|---|---|---|
| -0.326867 | -0.327077 | -0.321711 | -0.312852 | -0.299657 | -0.234698 | -0.12379 |
| -0.72391 | -0.691823 | -0.659941 | -0.623428 | -0.580299 | -0.427005 | -0.227876 |
| -0.652015 | -0.617936 | -0.583611 | -0.546331 | -0.506449 | -0.393246 | -0.225731 |
| -1.14192 | -1.09625 | -1.04439 | -0.98932 | -0.931513 | -0.736839 | -0.434693 |
| -1.06768 | -0.999928 | -0.928551 | -0.854701 | -0.782138 | -0.584526 | -0.315384 |
| -1.38701 | -1.28098 | -1.18271 | -1.09016 | -1.0004 | -0.744951 | -0.424105 |
| -1.72043 | -1.61558 | -1.50499 | -1.39116 | -1.28169 | -0.988007 | -0.543719 |
| -0.565221 | -0.545001 | -0.518136 | -0.486114 | -0.452986 | -0.348065 | -0.185498 |
| -1.22851 | -1.10305 | -0.983468 | -0.872081 | -0.769202 | -0.505961 | -0.266095 |
| -1.61101 | -1.47366 | -1.34134 | -1.21359 | -1.08734 | -0.749747 | -0.32133 |
| -2.37656 | -2.1759 | -1.98948 | -1.8115 | -1.64136 | -0.970481 | -0.380792 |
| -0.827571 | -0.80051 | -0.768577 | -0.729602 | -0.682294 | -0.525123 | -0.314019 |
| -1.76701 | -1.62929 | -1.49174 | -1.35596 | -1.22963 | -0.899355 | -0.514024 |
| -2.10006 | -1.92219 | -1.75667 | -1.60398 | -1.46283 | -1.06447 | -0.600872 |
| -2.64495 | -2.44869 | -2.26142 | -2.08055 | -1.90345 | -1.41036 | -0.848577 |
| -0.799901 | -0.753996 | -0.702827 | -0.650356 | -0.599668 | -0.457183 | -0.25738 |
| -2.69827 | -2.53139 | -2.35511 | -2.18554 | -2.03601 | -1.63549 | -1.0097 |
| -0.915323 | -0.865526 | -0.816364 | -0.758519 | -0.690284 | -0.481865 | -0.263874 |
| -1.50591 | -1.38598 | -1.28494 | -1.1922 | -1.09569 | -0.780078 | -0.428327 |
| -1.97316 | -1.89096 | -1.79971 | -1.70408 | -1.60477 | -1.30276 | -0.827049 |
| -2.00787 | -1.89762 | -1.78771 | -1.67368 | -1.55953 | -1.22405 | -0.757036 |
| -2.27155 | -2.15017 | -2.02281 | -1.89886 | -1.78182 | -1.45453 | -0.926067 |
| -2.36483 | -2.23466 | -2.10617 | -1.97851 | -1.85614 | -1.49994 | -0.948308 |

| | | | | | | |
|---|---|---|---|---|---|---|
| -6.62016 | -5.53925 | -4.54081 | -3.67739 | -2.97446 | -1.58908 | -0.544887 |
| -6.62898 | -5.61764 | -4.70412 | -3.9081 | -3.20846 | -1.75617 | -0.63535 |
| -8.38156 | -7.32991 | -6.34173 | -5.47614 | -4.73081 | -2.98285 | -1.35343 |
| -6.702 | -5.62278 | -4.66405 | -3.80763 | -3.07678 | -1.66279 | -0.582479 |
| -7.64564 | -6.62094 | -5.66326 | -4.78273 | -4.02169 | -2.37423 | -0.962812 |
| -7.83089 | -6.61799 | -5.54718 | -4.60807 | -3.80982 | -2.10405 | -0.818072 |
| -3.56553 | -2.99485 | -2.48977 | -2.04688 | -1.663 | -0.876906 | -0.329678 |
| -3.82291 | -3.31574 | -2.84437 | -2.41577 | -2.0406 | -1.2004 | -0.513285 |
| -3.38895 | -2.94302 | -2.52723 | -2.15308 | -1.82262 | -1.06632 | -0.45324 |
| -3.50584 | -2.98352 | -2.5142 | -2.12054 | -1.76848 | -0.975317 | -0.397855 |
| -5.94004 | -5.03643 | -4.2872 | -3.64562 | -3.09542 | -1.91932 | -0.881986 |
| -4.03086 | -3.3765 | -2.80167 | -2.33076 | -1.95151 | -1.21449 | -0.559263 |
| -2.67258 | -2.23449 | -1.85566 | -1.55433 | -1.31148 | -0.83257 | -0.395927 |
| -3.83927 | -3.15587 | -2.60138 | -2.15883 | -1.80715 | -1.1256 | -0.524754 |
| -4.50644 | -3.81881 | -3.16771 | -2.61796 | -2.18079 | -1.32515 | -0.614268 |
| -5.34632 | -4.48222 | -3.73901 | -3.10128 | -2.57266 | -1.47009 | -0.632476 |
| -4.03326 | -3.35912 | -2.82498 | -2.35542 | -1.96095 | -1.16842 | -0.530171 |
| -6.49327 | -5.61654 | -4.83295 | -4.13591 | -3.4071 | -1.90576 | -0.807052 |
| -5.90202 | -5.01107 | -4.21703 | -3.52918 | -2.9552 | -1.71458 | -0.793135 |
| -4.62178 | -3.94279 | -3.32264 | -2.78529 | -2.34573 | -1.4224 | -0.645987 |
| -2.83652 | -2.41427 | -2.04297 | -1.72548 | -1.43877 | -0.856824 | -0.379337 |
| -2.56363 | -2.16307 | -1.81034 | -1.51607 | -1.26521 | -0.719522 | -0.303425 |
| -5.2537 | -4.62415 | -4.04663 | -3.53359 | -3.0776 | -1.99072 | -0.900766 |
| -3.77466 | -3.1514 | -2.62465 | -2.19725 | -1.83053 | -1.11603 | -0.471468 |
| -3.60824 | -3.10688 | -2.66252 | -2.27183 | -1.92004 | -1.21917 | -0.543749 |
| -3.81775 | -3.19626 | -2.67534 | -2.2476 | -1.87512 | -1.12507 | -0.475137 |
| -2.45312 | -2.08845 | -1.75686 | -1.45281 | -1.17717 | -0.663313 | -0.277554 |
| -0.845954 | -0.720968 | -0.60605 | -0.50217 | -0.411615 | -0.233541 | -0.0981479 |
| -2.85515 | -2.47948 | -2.15866 | -1.88099 | -1.64642 | -1.05564 | -0.482772 |
| -2.50951 | -2.24123 | -1.98064 | -1.73781 | -1.52384 | -1.01676 | -0.515029 |
| -1.55974 | -1.32255 | -1.12764 | -0.97574 | -0.843529 | -0.500883 | -0.225283 |
| -2.95141 | -2.54452 | -2.18706 | -1.87177 | -1.61646 | -1.01261 | -0.46158 |
| -3.08595 | -2.66084 | -2.27554 | -1.93027 | -1.63638 | -0.974783 | -0.414788 |
| -4.67638 | -3.963 | -3.34009 | -2.82244 | -2.42937 | -1.45564 | -0.65257 |
| -2.31505 | -2.06629 | -1.70783 | -1.39602 | -1.14913 | -0.637166 | -0.274789 |
| -0.48006 | -0.451346 | -0.416328 | -0.379079 | -0.342598 | -0.240165 | -0.114522 |
| -1.55758 | -1.4095 | -1.25632 | -1.10996 | -0.974756 | -0.645566 | -0.311902 |
| -3.51694 | -3.10074 | -2.73072 | -2.38821 | -2.08162 | -1.36417 | -0.622146 |
| -3.97024 | -3.4721 | -3.02148 | -2.61942 | -2.27842 | -1.47436 | -0.722576 |
| -4.13232 | -3.57169 | -3.03524 | -2.55665 | -2.14798 | -1.27078 | -0.536777 |
| -2.59474 | -2.2883 | -2.00429 | -1.74264 | -1.51791 | -0.975469 | -0.416852 |
| -1.10536 | -0.99592 | -0.894934 | -0.796125 | -0.702062 | -0.46006 | -0.229374 |
| -2.8206 | -2.52769 | -2.24963 | -1.98708 | -1.74169 | -1.16548 | -0.581288 |

| | | | | | | |
|---|---|---|---|---|---|---|
| | **Beta=0.76** | | | | | |
| -0.0366977 | 1 | -0.305173 | -0.306266 | -0.302358 | -0.295442 | -0.284528 |
| -0.0724588 | 2 | -0.685601 | -0.657152 | -0.629141 | -0.596747 | -0.557965 |
| -0.0704077 | 3 | -0.619703 | -0.587611 | -0.555673 | -0.521361 | -0.484939 |
| -0.109684 | 4 | -1.08663 | -1.04542 | -0.998602 | -0.948779 | -0.896208 |
| -0.105864 | 5 | -1.0242 | -0.962025 | -0.896353 | -0.828131 | -0.7607 |
| -0.139659 | 6 | -1.33116 | -1.23198 | -1.14013 | -1.05347 | -0.969346 |
| -0.12602 | 7 | -1.65768 | -1.56033 | -1.45728 | -1.35071 | -1.24789 |
| -0.0590585 | 8 | -0.531693 | -0.514234 | -0.490762 | -0.462437 | -0.432841 |
| -0.0743704 | 9 | -1.19293 | -1.07564 | -0.963084 | -0.857333 | -0.758952 |
| -0.078157 | 10 | -1.54662 | -1.42001 | -1.29739 | -1.17824 | -1.05964 |
| -0.0998299 | 11 | -2.30378 | -2.11673 | -1.94204 | -1.77418 | -1.61257 |
| -0.094972 | 12 | -0.782427 | -0.758245 | -0.729818 | -0.695035 | -0.652603 |
| -0.175227 | 13 | -1.71632 | -1.58683 | -1.45731 | -1.32892 | -1.20893 |
| -0.207757 | 14 | -2.03391 | -1.86628 | -1.71005 | -1.56552 | -1.43158 |
| -0.259934 | 15 | -2.5781 | -2.39106 | -2.2131 | -2.04089 | -1.87168 |
| -0.081431 | 16 | -0.769187 | -0.727028 | -0.680003 | -0.631688 | -0.584792 |
| -0.373834 | 17 | -2.61505 | -2.4558 | -2.28814 | -2.12687 | -1.98424 |
| -0.08708 | 18 | -0.879051 | -0.832274 | -0.78623 | -0.731903 | -0.668243 |
| -0.150365 | 19 | -1.46145 | -1.34728 | -1.25084 | -1.16221 | -1.07009 |
| -0.281564 | 20 | -1.89826 | -1.82021 | -1.73424 | -1.64402 | -1.55072 |
| -0.223261 | 21 | -1.92687 | -1.8232 | -1.72029 | -1.61437 | -1.50793 |
| -0.324999 | 22 | -2.19501 | -2.07937 | -1.9583 | -1.84058 | -1.72973 |
| -0.34641 | 23 | -2.2843 | -2.16073 | -2.03835 | -1.9178 | -1.80226 |

| | | | | | | |
|---|---|---|---|---|---|---|
| -0.10352 | 24 | -6.48368 | -5.45972 | -4.49104 | -3.65213 | -2.96358 |
| -0.127592 | 25 | -6.47512 | -5.51384 | -4.63966 | -3.86566 | -3.18375 |
| -0.352676 | 26 | -8.15049 | -7.16021 | -6.2235 | -5.39457 | -4.67515 |
| -0.112555 | 27 | -6.54469 | -5.5192 | -4.59852 | -3.76925 | -3.05654 |
| -0.221652 | 28 | -7.45696 | -6.48809 | -5.57312 | -4.72583 | -3.98802 |
| -0.177979 | 29 | -7.6152 | -6.47444 | -5.45584 | -4.55369 | -3.77959 |
| -0.0619902 | 30 | -3.47127 | -2.93464 | -2.45428 | -2.02835 | -1.65557 |
| -0.11566 | 31 | -3.70914 | -3.23368 | -2.7868 | -2.37677 | -2.01511 |
| -0.10527 | 32 | -3.27962 | -2.86379 | -2.47184 | -2.11588 | -1.7983 |
| -0.0821185 | 33 | -3.40856 | -2.91832 | -2.47395 | -2.09629 | -1.75453 |
| -0.266811 | 34 | -5.82484 | -4.96111 | -4.23749 | -3.61054 | -3.07158 |
| -0.171276 | 35 | -3.97524 | -3.34095 | -2.77908 | -2.31685 | -1.94285 |
| -0.120847 | 36 | -2.65272 | -2.22081 | -1.84749 | -1.54926 | -1.30816 |
| -0.158032 | 37 | -3.81476 | -3.14711 | -2.60218 | -2.16587 | -1.81732 |
| -0.190426 | 38 | -4.44571 | -3.79076 | -3.1524 | -2.6114 | -2.17861 |
| -0.128235 | 39 | -5.27949 | -4.44836 | -3.72623 | -3.10087 | -2.57887 |
| -0.134976 | 40 | -3.98096 | -3.33019 | -2.80898 | -2.34798 | -1.95889 |
| -0.192092 | 41 | -6.36138 | -5.52656 | -4.77352 | -4.09771 | -3.38625 |
| -0.197643 | 42 | -5.80185 | -4.94874 | -4.18191 | -3.51123 | -2.94837 |
| -0.174547 | 43 | -4.52891 | -3.8786 | -3.28141 | -2.75946 | -2.32977 |
| -0.106301 | 44 | -2.77922 | -2.37596 | -2.01796 | -1.70903 | -1.42851 |
| -0.0761701 | 45 | -2.50115 | -2.1218 | -1.78364 | -1.49855 | -1.2535 |
| -0.234655 | 46 | -5.13416 | -4.53837 | -3.98671 | -3.49276 | -3.05003 |
| -0.123167 | 47 | -3.70499 | -3.11104 | -2.60458 | -2.18716 | -1.82868 |
| -0.147817 | 48 | -3.53632 | -3.05944 | -2.63263 | -2.25443 | -1.91126 |
| -0.12128 | 49 | -3.74637 | -3.15386 | -2.65283 | -2.23243 | -1.86732 |
| -0.0663507 | 50 | -2.38959 | -2.04613 | -1.72961 | -1.4364 | -1.16852 |
| -0.0248386 | 51 | -0.821916 | -0.704743 | -0.595702 | -0.495929 | -0.408136 |
| -0.137967 | 52 | -2.79339 | -2.43822 | -2.13193 | -1.86387 | -1.63498 |
| -0.139823 | 53 | -2.44365 | -2.19049 | -1.94301 | -1.71054 | -1.50399 |
| -0.0542611 | 54 | -1.51493 | -1.29313 | -1.1081 | -0.961847 | -0.832894 |
| -0.123533 | 55 | -2.88277 | -2.50181 | -2.1605 | -1.85632 | -1.60734 |
| -0.0924294 | 56 | -3.01637 | -2.6139 | -2.24546 | -1.91187 | -1.62515 |
| -0.165759 | 57 | -4.58027 | -3.89402 | -3.29725 | -2.80575 | -2.4216 |
| -0.0863174 | 58 | -2.24443 | -2.01064 | -1.67124 | -1.37284 | -1.13375 |
| -0.0309218 | 59 | -0.453123 | -0.428023 | -0.397147 | -0.363919 | -0.330907 |
| -0.0846724 | 60 | -1.4982 | -1.36305 | -1.2215 | -1.08462 | -0.95675 |
| -0.161692 | 61 | -3.44699 | -3.05025 | -2.69475 | -2.36324 | -2.06512 |
| -0.213746 | 62 | -3.88172 | -3.40977 | -2.97869 | -2.59056 | -2.25883 |
| -0.121627 | 63 | -4.03182 | -3.50167 | -2.99036 | -2.53004 | -2.13376 |
| -0.0849708 | 64 | -2.52485 | -2.23713 | -1.96762 | -1.71706 | -1.49983 |
| -0.0691062 | 65 | -1.07396 | -0.971444 | -0.875887 | -0.78198 | -0.692242 |
| -0.169629 | 66 | -2.7479 | -2.47059 | -2.20566 | -1.95432 | -1.71912 |

| | | | | | | | |
|---|---|---|---|---|---|---|---|
| | | | **Beta=0.77** | | | | |
| -0.226905 | -0.122636 | -0.0366849 | **Beta=0.77** | | | | |
| -0.416486 | -0.225892 | -0.0720854 | | 1 | -0.28521 | -0.28643 | -0.283633 |
| -0.381023 | -0.222178 | -0.0696622 | | 2 | -0.649456 | -0.624309 | -0.599658 |
| -0.715989 | -0.428258 | -0.109984 | | 3 | -0.589438 | -0.55909 | -0.529238 |
| -0.573963 | -0.312709 | -0.104177 | | 4 | -1.03376 | -0.99651 | -0.954179 |
| -0.728479 | -0.418519 | -0.136705 | | 5 | -0.984955 | -0.927697 | -0.867175 |
| -0.969187 | -0.537955 | -0.123652 | | 6 | -1.28316 | -1.19021 | -1.10408 |
| -0.336709 | -0.181519 | -0.0562875 | | 7 | -1.60118 | -1.51083 | -1.41484 |
| -0.504342 | -0.266365 | -0.0754144 | | 8 | -0.50575 | -0.490609 | -0.470054 |
| -0.738713 | -0.32034 | -0.078162 | | 9 | -1.15384 | -1.04442 | -0.938774 |
| -0.964974 | -0.383533 | -0.102449 | | 10 | -1.48375 | -1.36712 | -1.25369 |
| -0.509086 | -0.309138 | -0.0944272 | | 11 | -2.22272 | -2.04886 | -1.88576 |
| -0.891255 | -0.513496 | -0.176011 | | 12 | -0.739258 | -0.717572 | -0.692228 |
| -1.05187 | -0.599772 | -0.208593 | | 13 | -1.66435 | -1.54279 | -1.42099 |
| -1.39649 | -0.846245 | -0.261289 | | 14 | -1.96928 | -1.81155 | -1.66436 |
| -0.450636 | -0.256722 | -0.0816976 | | 15 | -2.50786 | -2.33151 | -2.16257 |
| -1.60141 | -0.999393 | -0.373516 | | 16 | -0.739346 | -0.70057 | -0.657325 |
| -0.47242 | -0.261992 | -0.0864657 | | 17 | -2.53827 | -2.38596 | -2.22608 |
| -0.768269 | -0.425592 | -0.148579 | | 18 | -0.845685 | -0.801676 | -0.75823 |
| -1.26782 | -0.816447 | -0.282747 | | 19 | -1.41857 | -1.31051 | -1.21899 |
| -1.19352 | -0.746157 | -0.221199 | | 20 | -1.82716 | -1.75307 | -1.67161 |
| -1.41954 | -0.914906 | -0.325771 | | 21 | -1.85388 | -1.75634 | -1.65985 |
| -1.46503 | -0.936853 | -0.346488 | | 22 | -2.12159 | -2.01132 | -1.89602 |

| | | | | | | |
|---|---|---|---|---|---|---|
| -1.59214 | -0.551709 | -0.108695 | 23 | -2.2064 | -2.0889 | -1.97279 |
| -1.75275 | -0.637307 | -0.127841 | 24 | -6.33123 | -5.35156 | -4.42849 |
| -2.9685 | -1.35626 | -0.353752 | 25 | -6.31077 | -5.40238 | -4.56322 |
| -1.66288 | -0.586819 | -0.115368 | 26 | -7.91332 | -6.98531 | -6.09866 |
| -2.37167 | -0.9706 | -0.226617 | 27 | -6.39165 | -5.41758 | -4.53341 |
| -2.10226 | -0.824271 | -0.181775 | 28 | -7.25367 | -6.3395 | -5.46991 |
| -0.882101 | -0.336327 | -0.0676491 | 29 | -7.38701 | -6.319 | -5.35309 |
| -1.19547 | -0.514775 | -0.116763 | 30 | -3.35976 | -2.85791 | -2.40299 |
| -1.06187 | -0.453512 | -0.105126 | 31 | -3.59376 | -3.14921 | -2.72719 |
| -0.974555 | -0.399688 | -0.0839171 | 32 | -3.1704 | -2.78359 | -2.41531 |
| -1.91284 | -0.882651 | -0.264521 | 33 | -3.29889 | -2.83939 | -2.41944 |
| -1.21255 | -0.561688 | -0.172239 | 34 | -5.70774 | -4.8846 | -4.1879 |
| -0.830686 | -0.396861 | -0.12155 | 35 | -3.91794 | -3.3044 | -2.75611 |
| -1.13731 | -0.539226 | -0.171681 | 36 | -2.62779 | -2.20405 | -1.83677 |
| -1.32651 | -0.607343 | -0.183215 | 37 | -3.75872 | -3.10899 | -2.57453 |
| -1.48512 | -0.647257 | -0.142815 | 38 | -4.39061 | -3.75347 | -3.12853 |
| -1.17079 | -0.531999 | -0.136725 | 39 | -5.18203 | -4.38408 | -3.68371 |
| -1.90632 | -0.810527 | -0.194796 | 40 | -3.92543 | -3.29847 | -2.79097 |
| -1.72861 | -0.803253 | -0.207223 | 41 | -6.21778 | -5.42628 | -4.70543 |
| -1.41933 | -0.647427 | -0.174977 | 42 | -5.67655 | -4.86401 | -4.12543 |
| -0.854606 | -0.380721 | -0.106527 | 43 | -4.42816 | -3.80856 | -3.23456 |
| -0.715524 | -0.300853 | -0.0729894 | 44 | -2.71907 | -2.33526 | -1.99115 |
| -1.98464 | -0.903217 | -0.235351 | 45 | -2.44256 | -2.08424 | -1.76098 |
| -1.11301 | -0.471976 | -0.123451 | 46 | -5.00841 | -4.44638 | -3.92114 |
| -1.21363 | -0.543886 | -0.147904 | 47 | -3.62706 | -3.05874 | -2.56803 |
| -1.1232 | -0.47827 | -0.124176 | 48 | -3.45739 | -3.00321 | -2.59269 |
| -0.662623 | -0.278175 | -0.0671747 | 49 | -3.6643 | -3.09963 | -2.61538 |
| -0.233161 | -0.0984233 | -0.024879 | 50 | -2.32377 | -2.00121 | -1.70003 |
| -1.05435 | -0.487705 | -0.14155 | 51 | -0.796513 | -0.687784 | -0.58467 |
| -1.00883 | -0.512757 | -0.13832 | 52 | -2.72141 | -2.3865 | -2.095 |
| -0.498682 | -0.225263 | -0.0544115 | 53 | -2.37994 | -2.14159 | -1.90713 |
| -1.01301 | -0.464827 | -0.125069 | 54 | -1.47048 | -1.26359 | -1.08842 |
| -0.974943 | -0.417968 | -0.0957596 | 55 | -2.81216 | -2.45301 | -2.12804 |
| -1.46255 | -0.663029 | -0.176047 | 56 | -2.93695 | -2.5571 | -2.2059 |
| -0.632539 | -0.273539 | -0.0853814 | 57 | -4.46435 | -3.81368 | -3.24294 |
| -0.235456 | -0.113965 | -0.0308861 | 58 | -2.17862 | -1.96041 | -1.63882 |
| -0.639521 | -0.31131 | -0.0849987 | 59 | -0.428946 | -0.406796 | -0.379407 |
| -1.36045 | -0.622642 | -0.160725 | 60 | -1.43802 | -1.31524 | -1.1849 |
| -1.4689 | -0.723428 | -0.212503 | 61 | -3.37541 | -2.9984 | -2.65789 |
| -1.27288 | -0.541409 | -0.125671 | 62 | -3.79191 | -3.34618 | -2.93507 |
| -0.969123 | -0.416842 | -0.0843294 | 63 | -3.91849 | -3.42063 | -2.93466 |
| -0.458872 | -0.232091 | -0.0727633 | 64 | -2.45493 | -2.18557 | -1.93079 |
| -1.15907 | -0.582778 | -0.170823 | 65 | -1.03952 | -0.942315 | -0.850927 |
| | | | 66 | -2.66444 | -2.40447 | -2.15429 |

| | | | | | | |
|---|---|---|---|---|---|---|
| | | | | | **Beta=0.78** | |
| | | | | | 1 | -0.266919 |
| -0.27831 | -0.269366 | -0.218566 | -0.121021 | -0.03649 | 2 | -0.614847 |
| -0.570968 | -0.536114 | -0.405737 | -0.223709 | -0.0717374 | 3 | -0.560984 |
| -0.497549 | -0.46423 | -0.369008 | -0.218943 | -0.0696277 | 4 | -0.983652 |
| -0.909083 | -0.861297 | -0.694777 | -0.421471 | -0.110262 | 5 | -0.943795 |
| -0.804143 | -0.741543 | -0.565494 | -0.312585 | -0.105543 | 6 | -1.23056 |
| -1.02278 | -0.943364 | -0.71629 | -0.418211 | -0.139582 | 7 | -1.54065 |
| -1.31516 | -1.21868 | -0.954665 | -0.536946 | -0.12638 | 8 | -0.475723 |
| -0.444996 | -0.418605 | -0.330738 | -0.182819 | -0.0588862 | 9 | -1.1179 |
| -0.838745 | -0.745016 | -0.499609 | -0.26444 | -0.0746356 | 10 | -1.42219 |
| -1.14283 | -1.03175 | -0.726971 | -0.318784 | -0.0781277 | 11 | -2.15043 |
| -1.72808 | -1.5752 | -0.952568 | -0.380827 | -0.100114 | 12 | -0.699118 |
| -0.661195 | -0.623171 | -0.492548 | -0.303979 | -0.0941839 | 13 | -1.61382 |
| -1.29979 | -1.18604 | -0.881206 | -0.511623 | -0.175877 | 14 | -1.90474 |
| -1.5278 | -1.40092 | -1.03802 | -0.598071 | -0.209336 | 15 | -2.4405 |
| -1.99881 | -1.83738 | -1.38034 | -0.842326 | -0.261639 | 16 | -0.710398 |
| -0.612847 | -0.569512 | -0.443445 | -0.25563 | -0.0818143 | 17 | -2.46122 |
| -2.07228 | -1.93583 | -1.56842 | -0.989541 | -0.373847 | 18 | -0.812505 |
| -0.707512 | -0.647769 | -0.463488 | -0.260184 | -0.0857461 | 19 | -1.37675 |
| -1.13476 | -1.04723 | -0.75948 | -0.425637 | -0.149509 | 20 | -1.75722 |
| -1.58642 | -1.4986 | -1.23299 | -0.804968 | -0.283247 | 21 | -1.77947 |
| -1.56081 | -1.46148 | -1.16638 | -0.738706 | -0.223133 | 22 | -2.05109 |
| -1.78392 | -1.67817 | -1.38323 | -0.901642 | -0.325506 | 23 | -2.13281 |

| | | | | | | |
|---|---|---|---|---|---|---|
| -1.85861 | -1.74917 | -1.42894 | -0.923901 | -0.345554 | 24 | -6.18881 |
| -3.61514 | -2.94195 | -1.58628 | -0.54965 | -0.105039 | 25 | -6.14943 |
| -3.81363 | -3.15512 | -1.74925 | -0.639241 | -0.128456 | 26 | -7.67912 |
| -5.30802 | -4.61553 | -2.95401 | -1.36059 | -0.356282 | 27 | -6.22538 |
| -3.72956 | -3.03418 | -1.65942 | -0.586295 | -0.113453 | 28 | -7.05412 |
| -4.65658 | -3.943 | -2.3616 | -0.97118 | -0.224229 | 29 | -7.16609 |
| -4.4883 | -3.73948 | -2.09495 | -0.82361 | -0.179046 | 30 | -3.26232 |
| -1.99498 | -1.63436 | -0.87561 | -0.332361 | -0.0631052 | 31 | -3.47806 |
| -2.33627 | -1.98841 | -1.18884 | -0.51492 | -0.116621 | 32 | -3.06049 |
| -2.07764 | -1.77327 | -1.05752 | -0.454558 | -0.105841 | 33 | -3.19791 |
| -2.05814 | -1.7291 | -0.967043 | -0.398453 | -0.0828693 | 34 | -5.58182 |
| -3.57701 | -3.05105 | -1.91078 | -0.888552 | -0.267721 | 35 | -3.85481 |
| -2.30119 | -1.93305 | -1.20838 | -0.561836 | -0.17144 | 36 | -2.60254 |
| -1.54207 | -1.30303 | -0.827381 | -0.396516 | -0.121209 | 37 | -3.72425 |
| -2.14516 | -1.80025 | -1.12273 | -0.527691 | -0.159506 | 38 | -4.33742 |
| -2.59395 | -2.1663 | -1.31912 | -0.603676 | -0.179151 | 39 | -5.1033 |
| -3.07162 | -2.55821 | -1.47424 | -0.637157 | -0.13251 | 40 | -3.86512 |
| -2.33656 | -1.95375 | -1.17075 | -0.532271 | -0.136943 | 41 | -6.07335 |
| -4.0524 | -3.35992 | -1.90539 | -0.812765 | -0.196658 | 42 | -5.56777 |
| -3.47417 | -2.92317 | -1.72122 | -0.796133 | -0.198985 | 43 | -4.33276 |
| -2.72936 | -2.31089 | -1.41641 | -0.648837 | -0.175226 | 44 | -2.65597 |
| -1.69141 | -1.41722 | -0.852318 | -0.38223 | -0.10707 | 45 | -2.37615 |
| -1.48556 | -1.24675 | -0.717255 | -0.304217 | -0.0757739 | 46 | -4.88023 |
| -3.44711 | -3.01857 | -1.97684 | -0.905433 | -0.236186 | 47 | -3.55602 |
| -2.16211 | -1.80883 | -1.11065 | -0.472685 | -0.123745 | 48 | -3.37831 |
| -2.22626 | -1.89129 | -1.20777 | -0.543488 | -0.148297 | 49 | -3.58655 |
| -2.20666 | -1.85039 | -1.11802 | -0.475755 | -0.121829 | 50 | -2.25722 |
| -1.41801 | -1.15814 | -0.660654 | -0.277619 | -0.0666803 | 51 | -0.771628 |
| -0.489124 | -0.404208 | -0.232571 | -0.0985976 | -0.0248572 | 52 | -2.65612 |
| -1.83711 | -1.61461 | -1.04525 | -0.485103 | -0.138116 | 53 | -2.31277 |
| -1.68508 | -1.48617 | -1.00371 | -0.513922 | -0.140432 | 54 | -1.42376 |
| -0.947947 | -0.822714 | -0.496756 | -0.225474 | -0.0546178 | 55 | -2.74122 |
| -1.83551 | -1.59361 | -1.01005 | -0.465481 | -0.124668 | 56 | -2.86221 |
| -1.88473 | -1.60598 | -0.968356 | -0.415292 | -0.0935002 | 57 | -4.35853 |
| -2.7684 | -2.39412 | -1.45182 | -0.657141 | -0.16977 | 58 | -2.11168 |
| -1.35285 | -1.12135 | -0.630285 | -0.273723 | -0.0852814 | 59 | -0.404806 |
| -0.349655 | -0.319718 | -0.230721 | -0.113314 | -0.0307949 | 60 | -1.38011 |
| -1.05728 | -0.936788 | -0.632167 | -0.310149 | -0.0851163 | 61 | -3.29858 |
| -2.33791 | -2.04878 | -1.35819 | -0.625425 | -0.162299 | 62 | -3.69607 |
| -2.56148 | -2.23972 | -1.46562 | -0.727295 | -0.214543 | 63 | -3.81255 |
| -2.49309 | -2.1098 | -1.26682 | -0.5392 | -0.123172 | 64 | -2.38133 |
| -1.69155 | -1.48212 | -0.963947 | -0.418436 | -0.0854605 | 65 | -1.00851 |
| -0.76174 | -0.6761 | -0.451188 | -0.227909 | -0.069011 | 66 | -2.59232 |
| -1.91544 | -1.69054 | -1.14747 | -0.580501 | -0.169563 | | |

| | | | | | | |
|---|---|---|---|---|---|---|
| -0.268403 | -0.26655 | -0.262507 | -0.255228 | -0.210592 | -0.119535 | -0.0364507 |
| -0.5926 | -0.570929 | -0.545491 | -0.514288 | -0.394632 | -0.22133 | -0.0714088 |
| -0.532173 | -0.504122 | -0.474698 | -0.44409 | -0.356703 | -0.21508 | -0.0688933 |
| -0.949971 | -0.911693 | -0.870917 | -0.827063 | -0.6734 | -0.414325 | -0.110451 |
| -0.891246 | -0.835616 | -0.777508 | -0.719522 | -0.553935 | -0.309458 | -0.10394 |
| -1.14354 | -1.06283 | -0.986558 | -0.912556 | -0.698885 | -0.411286 | -0.135987 |
| -1.45687 | -1.36752 | -1.27435 | -1.18396 | -0.934341 | -0.530474 | -0.124091 |
| -0.46257 | -0.444594 | -0.42249 | -0.399023 | -0.31903 | -0.178687 | -0.0563512 |
| -1.01586 | -0.916749 | -0.822211 | -0.732639 | -0.496638 | -0.264063 | -0.0752192 |
| -1.31479 | -1.20993 | -1.10687 | -1.00294 | -0.713766 | -0.317482 | -0.078153 |
| -1.98879 | -1.83648 | -1.68835 | -1.54375 | -0.94517 | -0.382962 | -0.102469 |
| -0.67954 | -0.656845 | -0.629082 | -0.594952 | -0.476118 | -0.298531 | -0.0935581 |
| -1.49966 | -1.38512 | -1.27076 | -1.16302 | -0.870976 | -0.510022 | -0.17627 |
| -1.75625 | -1.61747 | -1.48836 | -1.36819 | -1.02163 | -0.594204 | -0.208342 |
| -2.27354 | -2.11314 | -1.95743 | -1.80358 | -1.36379 | -0.838607 | -0.262674 |
| -0.674692 | -0.634905 | -0.593986 | -0.55401 | -0.435865 | -0.254409 | -0.0820315 |
| -2.31584 | -2.16399 | -2.01735 | -1.88683 | -1.53492 | -0.978971 | -0.374014 |
| -0.771053 | -0.730053 | -0.682229 | -0.626471 | -0.453594 | -0.257716 | -0.0852171 |
| -1.27366 | -1.18613 | -1.10554 | -1.02196 | -0.746826 | -0.42221 | -0.147708 |
| -1.68701 | -1.60989 | -1.52942 | -1.44672 | -1.19761 | -0.792308 | -0.283301 |
| -1.68761 | -1.59697 | -1.50418 | -1.41134 | -1.13539 | -0.726914 | -0.221062 |
| -1.9461 | -1.83635 | -1.72963 | -1.62894 | -1.34867 | -0.889617 | -0.326721 |
| -2.0212 | -1.91108 | -1.80291 | -1.69923 | -1.39544 | -0.91289 | -0.346818 |

| | | | | | | |
|---|---|---|---|---|---|---|
| -5.25941 | -4.37015 | -3.58331 | -2.92644 | -1.58838 | -0.555703 | -0.109552 |
| -5.28871 | -4.48924 | -3.7697 | -3.12629 | -1.74509 | -0.641209 | -0.128797 |
| -6.80927 | -5.97103 | -5.21758 | -4.5521 | -2.93643 | -1.36293 | -0.357614 |
| -5.30481 | -4.46059 | -3.68552 | -3.0102 | -1.65788 | -0.590352 | -0.115961 |
| -6.19686 | -5.37125 | -4.59225 | -3.90294 | -2.35669 | -0.977811 | -0.228705 |
| -6.16622 | -5.25296 | -4.42552 | -3.70263 | -2.09279 | -0.829611 | -0.183169 |
| -2.79253 | -2.36203 | -1.97161 | -1.62311 | -0.879215 | -0.338213 | -0.0680887 |
| -3.06377 | -2.6658 | -2.2939 | -1.96018 | -1.18204 | -0.515337 | -0.116989 |
| -2.70136 | -2.35615 | -2.03646 | -1.74622 | -1.05189 | -0.454703 | -0.105817 |
| -2.76975 | -2.37306 | -2.02821 | -1.71137 | -0.96872 | -0.400835 | -0.0852163 |
| -4.79916 | -4.12989 | -3.53557 | -3.02304 | -1.90311 | -0.889501 | -0.266195 |
| -3.26317 | -2.72956 | -2.2867 | -1.925 | -1.20611 | -0.564389 | -0.172919 |
| -2.18649 | -1.82673 | -1.53579 | -1.29794 | -0.824512 | -0.396396 | -0.120958 |
| -3.09289 | -2.56968 | -2.1472 | -1.80632 | -1.13198 | -0.539818 | -0.170922 |
| -3.71819 | -3.1085 | -2.58421 | -2.16203 | -1.32002 | -0.608126 | -0.182982 |
| -4.33743 | -3.66036 | -3.063 | -2.55864 | -1.48552 | -0.649204 | -0.144153 |
| -3.26263 | -2.76979 | -2.32466 | -1.94828 | -1.17134 | -0.533207 | -0.137678 |
| -5.32335 | -4.634 | -4.00392 | -3.33086 | -1.90154 | -0.813922 | -0.197361 |
| -4.79185 | -4.08186 | -3.45072 | -2.91235 | -1.72839 | -0.806758 | -0.208965 |
| -3.74088 | -3.18893 | -2.69968 | -2.29185 | -1.41231 | -0.650246 | -0.175884 |
| -2.29178 | -1.96196 | -1.67188 | -1.40461 | -0.849289 | -0.383321 | -0.107219 |
| -2.03877 | -1.7307 | -1.46544 | -1.23337 | -0.713244 | -0.302284 | -0.0733596 |
| -4.35127 | -3.85236 | -3.39855 | -2.98473 | -1.9682 | -0.907758 | -0.237402 |
| -3.01499 | -2.54449 | -2.15238 | -1.80756 | -1.10749 | -0.473212 | -0.123971 |
| -2.94792 | -2.55646 | -2.20318 | -1.87828 | -1.20236 | -0.54373 | -0.148423 |
| -3.05202 | -2.58774 | -2.19168 | -1.84257 | -1.11649 | -0.478695 | -0.124363 |
| -1.95508 | -1.66979 | -1.39927 | -1.14774 | -0.659307 | -0.278148 | -0.0673418 |
| -0.670736 | -0.573456 | -0.481916 | -0.399974 | -0.231896 | -0.09879 | -0.0248861 |
| -2.34108 | -2.06427 | -1.81672 | -1.60096 | -1.04368 | -0.489859 | -0.142112 |
| -2.08871 | -1.8669 | -1.65512 | -1.46391 | -0.994671 | -0.511398 | -0.138947 |
| -1.23161 | -1.06646 | -0.932237 | -0.811059 | -0.494 | -0.225328 | -0.0547539 |
| -2.40382 | -2.09542 | -1.81483 | -1.58044 | -1.00859 | -0.46774 | -0.12582 |
| -2.50461 | -2.17064 | -1.86215 | -1.5918 | -0.96714 | -0.417961 | -0.0962955 |
| -3.74473 | -3.20085 | -2.74398 | -2.38018 | -1.45539 | -0.665544 | -0.177518 |
| -1.90537 | -1.60156 | -1.32863 | -1.1052 | -0.625475 | -0.272456 | -0.0844455 |
| -0.385368 | -0.361252 | -0.334837 | -0.30793 | -0.225597 | -0.112617 | -0.0307858 |
| -1.26855 | -1.14877 | -1.03021 | -0.916929 | -0.624861 | -0.309209 | -0.0853012 |
| -2.94124 | -2.61596 | -2.30788 | -2.02812 | -1.35274 | -0.625973 | -0.161908 |
| -3.27622 | -2.8852 | -2.5266 | -2.21551 | -1.4584 | -0.728018 | -0.213839 |
| -3.34521 | -2.88433 | -2.46087 | -2.09084 | -1.2665 | -0.54318 | -0.126685 |
| -2.13009 | -1.88998 | -1.66228 | -1.461 | -0.956265 | -0.418085 | -0.0848001 |
| -0.916957 | -0.831159 | -0.746298 | -0.664561 | -0.44792 | -0.229927 | -0.0720639 |
| -2.34672 | -2.10892 | -1.88082 | -1.66508 | -1.13944 | -0.581402 | -0.171067 |

**Beta=0.80**

| | | | | | | |
|---|---|---|---|---|---|---|
| 1 | -0.2348 | -0.236089 | -0.235198 | -0.232935 | -0.228208 | -0.194216 |
| 2 | -0.551314 | -0.533741 | -0.516927 | -0.497012 | -0.472068 | -0.371861 |
| 3 | -0.509259 | -0.483095 | -0.458053 | -0.432384 | -0.406309 | -0.332624 |
| 4 | -0.889417 | -0.861798 | -0.830406 | -0.796919 | -0.761118 | -0.630755 |
| 5 | -0.86823 | -0.823745 | -0.776646 | -0.727285 | -0.677666 | -0.532034 |
| 6 | -1.13612 | -1.05965 | -0.988639 | -0.921476 | -0.856383 | -0.667417 |
| 7 | -1.42879 | -1.35645 | -1.27917 | -1.19794 | -1.11879 | -0.89673 |
| 8 | -0.42599 | -0.415883 | -0.402018 | -0.38478 | -0.36631 | -0.300528 |
| 9 | -1.04323 | -0.954804 | -0.868052 | -0.784176 | -0.704006 | -0.486357 |
| 10 | -1.30442 | -1.21341 | -1.12402 | -1.03535 | -0.944925 | -0.686527 |
| 11 | -2.0005 | -1.86116 | -1.7292 | -1.59944 | -1.47108 | -0.922192 |
| 12 | -0.62534 | -0.609138 | -0.590755 | -0.568432 | -0.540919 | -0.443021 |
| 13 | -1.51316 | -1.41274 | -1.31173 | -1.21024 | -1.11401 | -0.84756 |
| 14 | -1.77933 | -1.64805 | -1.52499 | -1.40998 | -1.30256 | -0.987947 |
| 15 | -2.30419 | -2.15458 | -2.01033 | -1.86998 | -1.73054 | -1.32732 |
| 16 | -0.654972 | -0.62459 | -0.590838 | -0.556204 | -0.522284 | -0.419102 |
| 17 | -2.31624 | -2.18372 | -2.04513 | -1.91132 | -1.79142 | -1.46776 |
| 18 | -0.751222 | -0.714257 | -0.677863 | -0.635574 | -0.586593 | -0.433874 |
| 19 | -1.29597 | -1.20272 | -1.12317 | -1.04985 | -0.974025 | -0.723527 |
| 20 | -1.62596 | -1.56326 | -1.49428 | -1.42246 | -1.3489 | -1.12861 |
| 21 | -1.64441 | -1.56286 | -1.48262 | -1.40077 | -1.31928 | -1.07667 |
| 22 | -1.91574 | -1.82073 | -1.72128 | -1.62431 | -1.53264 | -1.27847 |
| 23 | -1.99079 | -1.89012 | -1.79086 | -1.6934 | -1.59987 | -1.32562 |

| | | | | | | |
|---|---|---|---|---|---|---|
| 24 | -5.87784 | -5.04728 | -4.24029 | -3.50221 | -2.88064 | -1.58326 |
| 25 | -5.81299 | -5.04931 | -4.32544 | -3.66133 | -3.05975 | -1.73508 |
| 26 | -7.20787 | -6.44839 | -5.70555 | -5.02634 | -4.41632 | -2.8981 |
| 27 | -5.89148 | -5.07476 | -4.30802 | -3.59012 | -2.95453 | -1.6506 |
| 28 | -6.6432 | -5.89146 | -5.15322 | -4.44424 | -3.80666 | -2.33601 |
| 29 | -6.71415 | -5.84528 | -5.03255 | -4.2815 | -3.61351 | -2.07918 |
| 30 | -3.05002 | -2.64309 | -2.26113 | -1.90688 | -1.58425 | -0.874218 |
| 31 | -3.24582 | -2.88835 | -2.53793 | -2.20385 | -1.89867 | -1.16698 |
| 32 | -2.84294 | -2.53617 | -2.23536 | -1.95152 | -1.68767 | -1.03827 |
| 33 | -2.98593 | -2.61486 | -2.26439 | -1.95315 | -1.66182 | -0.959511 |
| 34 | -5.31917 | -4.61694 | -4.00446 | -3.44672 | -2.96364 | -1.88932 |
| 35 | -3.72049 | -3.17418 | -2.67138 | -2.25013 | -1.90303 | -1.19917 |
| 36 | -2.54327 | -2.1477 | -1.80095 | -1.51867 | -1.28728 | -0.819471 |
| 37 | -3.61882 | -3.02711 | -2.52891 | -2.12348 | -1.79209 | -1.12676 |
| 38 | -4.20865 | -3.63241 | -3.05493 | -2.5499 | -2.14061 | -1.31215 |
| 39 | -4.90443 | -4.20773 | -3.57925 | -3.01411 | -2.53034 | -1.48365 |
| 40 | -3.73309 | -3.18033 | -2.71881 | -2.29382 | -1.93223 | -1.17007 |
| 41 | -5.77 | -5.10277 | -4.47795 | -3.89628 | -3.26527 | -1.89275 |
| 42 | -5.3177 | -4.61865 | -3.96735 | -3.37853 | -2.86765 | -1.72449 |
| 43 | -4.13241 | -3.59664 | -3.09006 | -2.63419 | -2.24942 | -1.40327 |
| 44 | -2.52325 | -2.19837 | -1.89805 | -1.62864 | -1.37589 | -0.842174 |
| 45 | -2.24366 | -1.94712 | -1.66975 | -1.42578 | -1.20831 | -0.709228 |
| 46 | -4.61182 | -4.14696 | -3.70054 | -3.28821 | -2.9056 | -1.94458 |
| 47 | -3.39869 | -2.91031 | -2.47705 | -2.11082 | -1.78268 | -1.10136 |
| 48 | -3.2142 | -2.82976 | -2.47259 | -2.14617 | -1.84094 | -1.19051 |
| 49 | -3.41815 | -2.93917 | -2.51407 | -2.14422 | -1.81338 | -1.10918 |
| 50 | -2.12028 | -1.85881 | -1.60437 | -1.35753 | -1.12344 | -0.654815 |
| 51 | -0.720326 | -0.634273 | -0.548697 | -0.466242 | -0.390353 | -0.230066 |
| 52 | -2.51307 | -2.23626 | -1.98864 | -1.76255 | -1.56161 | -1.03119 |
| 53 | -2.18072 | -1.98378 | -1.78636 | -1.59481 | -1.41922 | -0.978039 |
| 54 | -1.32999 | -1.16577 | -1.0204 | -0.899037 | -0.78688 | -0.488049 |
| 55 | -2.59051 | -2.29527 | -2.01988 | -1.76408 | -1.54618 | -1.00093 |
| 56 | -2.70104 | -2.3867 | -2.08726 | -1.80522 | -1.55324 | -0.957287 |
| 57 | -4.12713 | -3.58299 | -3.09184 | -2.6712 | -2.33029 | -1.44504 |
| 58 | -1.98217 | -1.80067 | -1.52972 | -1.28255 | -1.07529 | -0.61817 |
| 59 | -0.361768 | -0.346499 | -0.327619 | -0.306743 | -0.285052 | -0.214987 |
| 60 | -1.26652 | -1.1752 | -1.07487 | -0.973311 | -0.874104 | -0.608022 |
| 61 | -3.13776 | -2.81936 | -2.52499 | -2.24165 | -1.9817 | -1.34005 |
| 62 | -3.49871 | -3.12925 | -2.77846 | -2.45078 | -2.16187 | -1.44283 |
| 63 | -3.58783 | -3.17843 | -2.76713 | -2.38261 | -2.04013 | -1.2566 |
| 64 | -2.23316 | -2.01652 | -1.8052 | -1.60076 | -1.41637 | -0.940722 |
| 65 | -0.948373 | -0.865534 | -0.788556 | -0.711908 | -0.637719 | -0.437577 |
| 66 | -2.43679 | -2.22071 | -2.00866 | -1.80302 | -1.6064 | -1.11607 |

| | | | | | | |
|---|---|---|---|---|---|---|
| | | **Beta=0.82** | | | | |
| -0.115811 | -0.0361763 | 1 | -0.207808 | -0.20853 | -0.207944 | -0.206684 |
| -0.215915 | -0.0707336 | 2 | -0.494503 | -0.480429 | -0.467287 | -0.451684 |
| -0.207402 | -0.0681117 | 3 | -0.463462 | -0.439567 | -0.41696 | -0.394236 |
| -0.399554 | -0.110713 | 4 | -0.80366 | -0.780965 | -0.755144 | -0.72759 |
| -0.305113 | -0.103657 | 5 | -0.797662 | -0.759914 | -0.720014 | -0.678139 |
| -0.402628 | -0.135263 | 6 | -1.04775 | -0.980457 | -0.917914 | -0.858735 |
| -0.521402 | -0.124495 | 7 | -1.32159 | -1.26 | -1.19325 | -1.12256 |
| -0.174965 | -0.0563498 | 8 | -0.381997 | -0.373993 | -0.363139 | -0.349631 |
| -0.261749 | -0.0754064 | 9 | -0.970629 | -0.894185 | -0.818585 | -0.744659 |
| -0.313916 | -0.0781522 | 10 | -1.19403 | -1.11686 | -1.04081 | -0.964833 |
| -0.381663 | -0.102494 | 11 | -1.85493 | -1.73574 | -1.62201 | -1.50903 |
| -0.286996 | -0.0926333 | 12 | -0.560111 | -0.546398 | -0.531258 | -0.513123 |
| -0.50526 | -0.17666 | 13 | -1.41484 | -1.32673 | -1.23787 | -1.14811 |
| -0.58667 | -0.207935 | 14 | -1.65864 | -1.54276 | -1.43389 | -1.33168 |
| -0.829364 | -0.264614 | 15 | -2.16983 | -2.03618 | -1.90669 | -1.7805 |
| -0.250811 | -0.0820954 | 16 | -0.603259 | -0.57731 | -0.548593 | -0.519264 |
| -0.955703 | -0.3731 | 17 | -2.17986 | -2.05948 | -1.93347 | -1.81122 |
| -0.252617 | -0.0838716 | 18 | -0.695423 | -0.66233 | -0.6298 | -0.592213 |
| -0.417392 | -0.146669 | 19 | -1.2197 | -1.13527 | -1.06286 | -0.996068 |
| -0.765846 | -0.283152 | 20 | -1.50299 | -1.44755 | -1.38624 | -1.3223 |
| -0.705682 | -0.220621 | 21 | -1.51983 | -1.44753 | -1.37634 | -1.30382 |
| -0.861927 | -0.326499 | 22 | -1.78853 | -1.70304 | -1.61317 | -1.52511 |
| -0.885905 | -0.345557 | 23 | -1.85803 | -1.76756 | -1.67816 | -1.59022 |

| | | | | | | |
|---|---|---|---|---|---|---|
| -0.559419 | -0.110399 | 24 | -5.55724 | -4.82132 | -4.08797 | -3.41331 |
| -0.644907 | -0.129856 | 25 | -5.469 | -4.7982 | -4.14905 | -3.5421 |
| -1.36798 | -0.361623 | 26 | -6.73974 | -6.08198 | -5.42783 | -4.82077 |
| -0.593791 | -0.116894 | 27 | -5.55131 | -4.83214 | -4.14236 | -3.48307 |
| -0.982921 | -0.230046 | 28 | -6.22914 | -5.57546 | -4.92121 | -4.28128 |
| -0.834704 | -0.184951 | 29 | -6.26542 | -5.51601 | -4.79944 | -4.12406 |
| -0.339794 | -0.0685196 | 30 | -2.83932 | -2.48895 | -2.15323 | -1.83492 |
| -0.516735 | -0.118572 | 31 | -3.01489 | -2.70965 | -2.40395 | -2.10679 |
| -0.455238 | -0.106439 | 32 | -2.62843 | -2.3696 | -2.11016 | -1.86041 |
| -0.401058 | -0.0856925 | 33 | -2.77496 | -2.45645 | -2.14923 | -1.87157 |
| -0.89552 | -0.268193 | 34 | -5.04212 | -4.41787 | -3.8627 | -3.34417 |
| -0.56729 | -0.174186 | 35 | -3.57381 | -3.07378 | -2.60446 | -2.20674 |
| -0.396912 | -0.12148 | 36 | -2.47717 | -2.10294 | -1.77187 | -1.49953 |
| -0.54106 | -0.171007 | 37 | -3.49924 | -2.94997 | -2.47958 | -2.09288 |
| -0.607942 | -0.181822 | 38 | -4.06384 | -3.53521 | -2.99182 | -2.51023 |
| -0.651505 | -0.145652 | 39 | -4.69016 | -4.06332 | -3.484 | -2.95445 |
| -0.53443 | -0.138529 | 40 | -3.58796 | -3.08525 | -2.65718 | -2.25512 |
| -0.816973 | -0.199621 | 41 | -5.45506 | -4.86694 | -4.30595 | -3.77407 |
| -0.809504 | -0.210633 | 42 | -5.05616 | -4.43194 | -3.83985 | -3.29524 |
| -0.653185 | -0.17749 | 43 | -3.92798 | -3.44557 | -2.98323 | -2.56086 |
| -0.385272 | -0.10774 | 44 | -2.38356 | -2.0971 | -1.82676 | -1.57925 |
| -0.303428 | -0.0737303 | 45 | -2.10663 | -1.84884 | -1.60185 | -1.38001 |
| -0.910267 | -0.238936 | 46 | -4.33602 | -3.93107 | -3.53544 | -3.16468 |
| -0.474547 | -0.124559 | 47 | -3.2325 | -2.79673 | -2.40208 | -2.06046 |
| -0.543588 | -0.149035 | 48 | -3.0461 | -2.70522 | -2.38304 | -2.0828 |
| -0.479542 | -0.124927 | 49 | -3.24241 | -2.81761 | -2.43226 | -2.0903 |
| -0.278158 | -0.067504 | 50 | -1.98111 | -1.75792 | -1.53386 | -1.31118 |
| -0.0990495 | -0.0249244 | 51 | -0.668767 | -0.596619 | -0.522322 | -0.448649 |
| -0.490944 | -0.142678 | 52 | -2.36705 | -2.12584 | -1.9064 | -1.70205 |
| -0.509376 | -0.139528 | 53 | -2.04939 | -1.87729 | -1.70266 | -1.53053 |
| -0.225116 | -0.0550752 | 54 | -1.23541 | -1.09691 | -0.970669 | -0.862526 |
| -0.469492 | -0.126532 | 55 | -2.43386 | -2.17848 | -1.9354 | -1.70488 |
| -0.417834 | -0.0968157 | 56 | -2.53586 | -2.26231 | -1.9966 | -1.74158 |
| -0.66765 | -0.178966 | 57 | -3.89016 | -3.41144 | -2.97169 | -2.58791 |
| -0.271534 | -0.0838115 | 58 | -1.85867 | -1.69934 | -1.45881 | -1.23398 |
| -0.110929 | -0.0306788 | 59 | -0.323697 | -0.311429 | -0.296512 | -0.280026 |
| -0.30653 | -0.085542 | 60 | -1.15864 | -1.08439 | -1.00106 | -0.914943 |
| -0.628062 | -0.162997 | 61 | -2.96819 | -2.68728 | -2.42362 | -2.16563 |
| -0.730892 | -0.214941 | 62 | -3.29386 | -2.9719 | -2.66045 | -2.3642 |
| -0.544425 | -0.127569 | 63 | -3.36057 | -3.00535 | -2.64166 | -2.29504 |
| -0.418704 | -0.0853274 | 64 | -2.08294 | -1.89836 | -1.71464 | -1.53324 |
| -0.226987 | -0.0708641 | 65 | -0.891963 | -0.816998 | -0.747464 | -0.678104 |
| -0.578826 | -0.170932 | 66 | -2.2834 | -2.09429 | -1.90618 | -1.72193 |

| | | | | | | |
|---|---|---|---|---|---|---|
| | | | **Bet=0.84** | | | |
| -0.203643 | -0.178095 | -0.111508 | -0.0358538 | 1 | -0.185049 | -0.18509 |
| -0.43181 | -0.348549 | -0.209635 | -0.0699996 | 2 | -0.443906 | -0.432446 |
| -0.371698 | -0.309196 | -0.199226 | -0.0673172 | 3 | -0.422677 | -0.400823 |
| -0.697944 | -0.587713 | -0.383026 | -0.110929 | 4 | -0.726108 | -0.707441 |
| -0.635829 | -0.508658 | -0.2997 | -0.103316 | 5 | -0.732117 | -0.699983 |
| -0.801466 | -0.634685 | -0.392606 | -0.134484 | 6 | -0.965342 | -0.906038 |
| -1.05318 | -0.856784 | -0.510582 | -0.124649 | 7 | -1.22039 | -1.16765 |
| -0.335144 | -0.281587 | -0.170414 | -0.0562301 | 8 | -0.343203 | -0.336615 |
| -0.673159 | -0.474267 | -0.258861 | -0.0755257 | 9 | -0.900523 | -0.834564 |
| -0.886588 | -0.657413 | -0.309566 | -0.0781309 | 10 | -1.09129 | -1.02578 |
| -1.39588 | -0.896266 | -0.37957 | -0.102512 | 11 | -1.71533 | -1.61343 |
| -0.490826 | -0.410381 | -0.274653 | -0.0916254 | 12 | -0.502496 | -0.490648 |
| -1.06255 | -0.821133 | -0.49893 | -0.176927 | 13 | -1.31955 | -1.24241 |
| -1.23596 | -0.951694 | -0.577475 | -0.207657 | 14 | -1.54296 | -1.44086 |
| -1.65458 | -1.28608 | -0.817019 | -0.265582 | 15 | -2.03794 | -1.91884 |
| -0.490577 | -0.401099 | -0.246368 | -0.082296 | 16 | -0.554942 | -0.532718 |
| -1.70087 | -1.40281 | -0.931965 | -0.372963 | 17 | -2.0495 | -1.94067 |
| -0.548958 | -0.414092 | -0.247138 | -0.0831915 | 18 | -0.644 | -0.614693 |
| -0.927185 | -0.698998 | -0.411313 | -0.145596 | 19 | -1.14754 | -1.07118 |
| -1.25686 | -1.06143 | -0.737455 | -0.282285 | 20 | -1.38734 | -1.3389 |
| -1.2319 | -1.0181 | -0.682668 | -0.219844 | 21 | -1.40423 | -1.34039 |
| -1.44154 | -1.21048 | -0.832926 | -0.325869 | 22 | -1.66836 | -1.59196 |
| -1.50562 | -1.25746 | -0.857574 | -0.344066 | 23 | -1.73292 | -1.65202 |

| | | | | | | |
|---|---|---|---|---|---|---|
| -2.82799 | -1.57593 | -0.562832 | -0.111287 | 24 | -5.23164 | -4.58566 |
| -2.98285 | -1.7214 | -0.647853 | -0.130644 | 25 | -5.12452 | -4.53967 |
| -4.26656 | -2.85139 | -1.37019 | -0.364838 | 26 | -6.27992 | -5.71382 |
| -2.88974 | -1.64038 | -0.596735 | -0.117615 | 27 | -5.20891 | -4.57995 |
| -3.69616 | -2.30971 | -0.987386 | -0.232115 | 28 | -5.81825 | -5.25471 |
| -3.51044 | -2.06057 | -0.838635 | -0.186519 | 29 | -5.82572 | -5.18379 |
| -1.53916 | -0.866837 | -0.341006 | -0.068927 | 30 | -2.6322 | -2.33234 |
| -1.83083 | -1.14784 | -0.516359 | -0.119357 | 31 | -2.78904 | -2.53081 |
| -1.62365 | -1.02133 | -0.455134 | -0.10708 | 32 | -2.42034 | -2.204 |
| -1.60633 | -0.947231 | -0.40069 | -0.0860837 | 33 | -2.56884 | -2.29728 |
| -2.89315 | -1.87045 | -0.900033 | -0.270101 | 34 | -4.75677 | -4.20586 |
| -1.87522 | -1.19032 | -0.569147 | -0.174894 | 35 | -3.41725 | -2.96362 |
| -1.27455 | -0.814042 | -0.39711 | -0.121846 | 36 | -2.40326 | -2.05251 |
| -1.77285 | -1.11998 | -0.541395 | -0.17053 | 37 | -3.36762 | -2.86248 |
| -2.11605 | -1.30491 | -0.608968 | -0.182187 | 38 | -3.90617 | -3.42383 |
| -2.49442 | -1.47988 | -0.653714 | -0.147126 | 39 | -4.46419 | -3.90404 |
| -1.91026 | -1.16676 | -0.535537 | -0.13931 | 40 | -3.43243 | -2.97899 |
| -3.18779 | -1.87886 | -0.818947 | -0.201166 | 41 | -5.13518 | -4.62073 |
| -2.81437 | -1.71713 | -0.812065 | -0.212555 | 42 | -4.78611 | -4.23371 |
| -2.20005 | -1.3898 | -0.654025 | -0.177778 | 43 | -3.72327 | -3.2908 |
| -1.34264 | -0.833362 | -0.386831 | -0.108407 | 44 | -2.23978 | -1.98986 |
| -1.17838 | -0.70326 | -0.304224 | -0.0740874 | 45 | -1.96786 | -1.74598 |
| -2.81457 | -1.91439 | -0.911416 | -0.240816 | 46 | -4.05754 | -3.70738 |
| -1.75273 | -1.09401 | -0.475802 | -0.125172 | 47 | -3.06301 | -2.67762 |
| -1.79883 | -1.1773 | -0.543255 | -0.149451 | 48 | -2.87621 | -2.57648 |
| -1.77893 | -1.10061 | -0.4802 | -0.125368 | 49 | -3.06277 | -2.68964 |
| -1.09539 | -0.648932 | -0.278091 | -0.0676559 | 50 | -1.84238 | -1.65411 |
| -0.379251 | -0.227579 | -0.0991277 | -0.0249385 | 51 | -0.618044 | -0.558147 |
| -1.51706 | -1.01645 | -0.491035 | -0.143213 | 52 | -2.22063 | -2.01193 |
| -1.37048 | -0.95879 | -0.506592 | -0.140052 | 53 | -1.92044 | -1.77075 |
| -0.760211 | -0.480685 | -0.224604 | -0.0553859 | 54 | -1.14167 | -1.02634 |
| -1.50481 | -0.989807 | -0.470166 | -0.127202 | 55 | -2.27442 | -2.05591 |
| -1.50933 | -0.94503 | -0.417412 | -0.0973044 | 56 | -2.36959 | -2.1337 |
| -2.27168 | -1.43075 | -0.668884 | -0.180127 | 57 | -3.65223 | -3.23373 |
| -1.04258 | -0.608976 | -0.269192 | -0.0818897 | 58 | -1.74062 | -1.60072 |
| -0.262677 | -0.203788 | -0.10889 | -0.0305639 | 59 | -0.290163 | -0.280016 |
| -0.829009 | -0.589116 | -0.303211 | -0.0857095 | 60 | -1.05732 | -0.997244 |
| -1.92643 | -1.32222 | -0.628815 | -0.16402 | 61 | -2.79336 | -2.5477 |
| -2.09889 | -1.42227 | -0.732188 | -0.216102 | 62 | -3.08577 | -2.80761 |
| -1.98086 | -1.24196 | -0.545561 | -0.128867 | 63 | -3.13486 | -2.8289 |
| -1.36626 | -0.92226 | -0.418508 | -0.0858184 | 64 | -1.9333 | -1.77777 |
| -0.610797 | -0.426339 | -0.224842 | -0.0704524 | 65 | -0.839305 | -0.771237 |
| -1.54383 | -1.08972 | -0.574826 | -0.17083 | 66 | -2.13284 | -1.96835 |

| | | | | | | |
|---|---|---|---|---|---|---|
| | | | | | | **Beta=0.86** |
| -0.184408 | -0.183584 | -0.181574 | -0.162508 | -0.106696 | -0.0354771 | 1 |
| -0.422053 | -0.409771 | -0.393938 | -0.325192 | -0.202639 | -0.0692777 | 2 |
| -0.380281 | -0.35994 | -0.340192 | -0.286717 | -0.190633 | -0.0664843 | 3 |
| -0.686154 | -0.663414 | -0.638838 | -0.545801 | -0.365842 | -0.110655 | 4 |
| -0.666127 | -0.630605 | -0.594606 | -0.484218 | -0.293263 | -0.102899 | 5 |
| -0.850904 | -0.798734 | -0.748326 | -0.601287 | -0.381347 | -0.133625 | 6 |
| -1.1101 | -1.04879 | -0.988657 | -0.815769 | -0.498451 | -0.124895 | 7 |
| -0.327926 | -0.317222 | -0.305844 | -0.262568 | -0.165107 | -0.0560114 | 8 |
| -0.768902 | -0.704044 | -0.640704 | -0.460263 | -0.255435 | -0.075585 | 9 |
| -0.961131 | -0.896205 | -0.828797 | -0.626854 | -0.304404 | -0.0780823 | 10 |
| -1.5159 | -1.41814 | -1.31907 | -0.867608 | -0.376628 | -0.102505 | 11 |
| -0.477953 | -0.463033 | -0.444814 | -0.378707 | -0.261672 | -0.0905236 | 12 |
| -1.16443 | -1.08527 | -1.00951 | -0.792133 | -0.49102 | -0.177036 | 13 |
| -1.34469 | -1.25406 | -1.16902 | -0.913228 | -0.566419 | -0.207239 | 14 |
| -1.80283 | -1.68961 | -1.57624 | -1.24111 | -0.80192 | -0.265824 | 15 |
| -0.508213 | -0.483346 | -0.45914 | -0.382307 | -0.241256 | -0.0829992 | 16 |
| -1.82637 | -1.71476 | -1.61321 | -1.33862 | -0.906063 | -0.371687 | 17 |
| -0.585565 | -0.552061 | -0.513742 | -0.393966 | -0.240785 | -0.0820604 | 18 |
| -1.0053 | -0.944438 | -0.881821 | -0.674085 | -0.404881 | -0.145104 | 19 |
| -1.28487 | -1.22827 | -1.17017 | -0.996508 | -0.707584 | -0.280701 | 20 |
| -1.27728 | -1.21289 | -1.1492 | -0.960318 | -0.658131 | -0.218699 | 21 |
| -1.51113 | -1.43136 | -1.35524 | -1.14464 | -0.802853 | -0.324685 | 22 |
| -1.57175 | -1.49247 | -1.4159 | -1.19102 | -0.827797 | -0.341899 | 23 |

| | | | | | | |
|---|---|---|---|---|---|---|
| -3.92696 | -3.30702 | -2.763 | -1.56559 | -0.565758 | -0.112102 | 24 |
| -3.96229 | -3.41285 | -2.89749 | -1.70286 | -0.649347 | -0.130417 | 25 |
| -5.14271 | -4.6044 | -4.1053 | -2.79601 | -1.36977 | -0.367789 | 26 |
| -3.96588 | -3.36523 | -2.81573 | -1.62639 | -0.599279 | -0.118399 | 27 |
| -4.67961 | -4.10653 | -3.57377 | -2.27715 | -0.990124 | -0.233968 | 28 |
| -4.55747 | -3.9548 | -3.39705 | -2.03636 | -0.841344 | -0.187893 | 29 |
| -2.04021 | -1.7568 | -1.48824 | -0.85688 | -0.341797 | -0.0693077 | 30 |
| -2.26664 | -2.00477 | -1.75739 | -1.12553 | -0.515203 | -0.120111 | 31 |
| -1.98248 | -1.76527 | -1.55499 | -1.00101 | -0.454243 | -0.107675 | 32 |
| -2.03041 | -1.78475 | -1.5452 | -0.932099 | -0.400073 | -0.0861288 | 33 |
| -3.70756 | -3.22914 | -2.81195 | -1.84613 | -0.902831 | -0.271926 | 34 |
| -2.52913 | -2.15643 | -1.84241 | -1.17963 | -0.570306 | -0.175456 | 35 |
| -1.73852 | -1.47732 | -1.25973 | -0.808261 | -0.397204 | -0.122282 | 36 |
| -2.42213 | -2.05605 | -1.74913 | -1.11209 | -0.541523 | -0.170218 | 37 |
| -2.92037 | -2.46363 | -2.08673 | -1.29673 | -0.610366 | -0.182916 | 38 |
| -3.37503 | -2.88351 | -2.44983 | -1.47237 | -0.655277 | -0.148194 | 39 |
| -2.58561 | -2.20864 | -1.88223 | -1.16133 | -0.536519 | -0.140151 | 40 |
| -4.12151 | -3.63959 | -3.09971 | -1.86038 | -0.820648 | -0.202947 | 41 |
| -3.70008 | -3.20064 | -2.75169 | -1.70519 | -0.813518 | -0.214063 | 42 |
| -2.8709 | -2.4818 | -2.14536 | -1.37403 | -0.65486 | -0.178779 | 43 |
| -1.74916 | -1.5242 | -1.30472 | -0.822455 | -0.38773 | -0.109037 | 44 |
| -1.52832 | -1.32881 | -1.14381 | -0.695179 | -0.304611 | -0.0744157 | 45 |
| -3.35972 | -3.02952 | -2.71226 | -1.87673 | -0.910253 | -0.242303 | 46 |
| -2.31988 | -2.00499 | -1.71653 | -1.08491 | -0.476784 | -0.125735 | 47 |
| -2.28792 | -2.01463 | -1.75151 | -1.16154 | -0.541771 | -0.149125 | 48 |
| -2.34329 | -2.02994 | -1.73971 | -1.09048 | -0.480751 | -0.125887 | 49 |
| -1.45872 | -1.26051 | -1.06358 | -0.641482 | -0.277856 | -0.067797 | 50 |
| -0.494599 | -0.429599 | -0.366753 | -0.224413 | -0.0990267 | -0.0249211 | 51 |
| -1.81911 | -1.63621 | -1.4677 | -0.999152 | -0.490182 | -0.143706 | 52 |
| -1.6171 | -1.46331 | -1.31839 | -0.936935 | -0.502974 | -0.14052 | 53 |
| -0.918139 | -0.823134 | -0.731084 | -0.471798 | -0.223738 | -0.0556683 | 54 |
| -1.84376 | -1.63836 | -1.45686 | -0.975081 | -0.469787 | -0.127809 | 55 |
| -1.90021 | -1.67202 | -1.46023 | -0.93013 | -0.416542 | -0.0977474 | 56 |
| -2.84301 | -2.49581 | -2.20528 | -1.4126 | -0.6695 | -0.181434 | 57 |
| -1.38768 | -1.18494 | -1.0096 | -0.600303 | -0.268195 | -0.0814255 | 58 |
| -0.268037 | -0.254953 | -0.241131 | -0.192171 | -0.106483 | -0.0304237 | 59 |
| -0.928533 | -0.85615 | -0.782464 | -0.568368 | -0.299245 | -0.0858364 | 60 |
| -2.31391 | -2.08118 | -1.86313 | -1.29918 | -0.628117 | -0.164956 | 61 |
| -2.53366 | -2.26847 | -2.02733 | -1.39649 | -0.731613 | -0.217157 | 62 |
| -2.51003 | -2.20022 | -1.91448 | -1.22313 | -0.545415 | -0.129608 | 63 |
| -1.61991 | -1.46081 | -1.3113 | -0.900834 | -0.417415 | -0.086263 | 64 |
| -0.70803 | -0.645221 | -0.584086 | -0.414557 | -0.222467 | -0.0701704 | 65 |
| -1.80272 | -1.63856 | -1.4781 | -1.06018 | -0.569569 | -0.17059 | 66 |

| | | | | | | |
|---|---|---|---|---|---|---|
| -0.165738 | -0.165092 | -0.164141 | -0.163406 | -0.161933 | -0.147683 | -0.101463 |
| -0.398919 | -0.389417 | -0.381072 | -0.371321 | -0.358664 | -0.302137 | -0.19497 |
| -0.386157 | -0.366194 | -0.34748 | -0.329137 | -0.311632 | -0.265415 | -0.181736 |
| -0.655682 | -0.640323 | -0.622741 | -0.60392 | -0.583486 | -0.505006 | -0.347834 |
| -0.671525 | -0.644062 | -0.615256 | -0.585091 | -0.554487 | -0.459127 | -0.285873 |
| -0.888803 | -0.83639 | -0.787742 | -0.741728 | -0.697334 | -0.567746 | -0.368993 |
| -1.12505 | -1.07998 | -1.03041 | -0.977199 | -0.924961 | -0.773444 | -0.484911 |
| -0.309053 | -0.3034 | -0.296239 | -0.287609 | -0.27861 | -0.243801 | -0.159142 |
| -0.833517 | -0.7766 | -0.719697 | -0.663042 | -0.607241 | -0.444625 | -0.251427 |
| -0.996322 | -0.940607 | -0.885601 | -0.830199 | -0.772305 | -0.595323 | -0.298432 |
| -1.58253 | -1.49566 | -1.41236 | -1.32818 | -1.24194 | -0.836619 | -0.37282 |
| -0.451601 | -0.441182 | -0.430349 | -0.417897 | -0.40285 | -0.348381 | -0.248219 |
| -1.22782 | -1.16044 | -1.09215 | -1.02253 | -0.955672 | -0.761034 | -0.481547 |
| -1.43276 | -1.34288 | -1.25806 | -1.17786 | -1.1025 | -0.873139 | -0.553576 |
| -1.9102 | -1.80433 | -1.70072 | -1.59937 | -1.49753 | -1.194 | -0.785056 |
| -0.510106 | -0.491048 | -0.470368 | -0.449263 | -0.428878 | -0.362674 | -0.235034 |
| -1.92519 | -1.82731 | -1.72397 | -1.62229 | -1.529 | -1.27616 | -0.878889 |
| -0.596721 | -0.570711 | -0.544663 | -0.514721 | -0.48062 | -0.374289 | -0.23439 |
| -1.07898 | -1.01006 | -0.950184 | -0.894727 | -0.837741 | -0.648475 | -0.397395 |
| -1.27841 | -1.23662 | -1.18949 | -1.13976 | -1.08841 | -0.934121 | -0.676679 |
| -1.29652 | -1.24047 | -1.1847 | -1.12755 | -1.07105 | -0.903843 | -0.632397 |
| -1.55411 | -1.48635 | -1.41406 | -1.34213 | -1.27299 | -1.08117 | -0.771646 |
| -1.61473 | -1.5428 | -1.47102 | -1.39974 | -1.33035 | -1.12649 | -0.796794 |

| | | | | | | |
|---|---|---|---|---|---|---|
| -4.90346 | -4.34364 | -3.75652 | -3.19301 | -2.6897 | -1.55173 | -0.568174 |
| -4.78345 | -4.27746 | -3.76793 | -3.27435 | -2.80316 | -1.68092 | -0.651359 |
| -5.8329 | -5.3487 | -4.85323 | -4.37969 | -3.93398 | -2.73239 | -1.36637 |
| -4.86893 | -4.32397 | -3.78101 | -3.23796 | -2.73279 | -1.60885 | -0.600958 |
| -5.41702 | -4.93401 | -4.43184 | -3.92208 | -3.44109 | -2.23766 | -0.991119 |
| -5.39913 | -4.85305 | -4.30924 | -3.77627 | -3.27312 | -2.00531 | -0.842626 |
| -2.43158 | -2.17676 | -1.92409 | -1.67386 | -1.43218 | -0.844235 | -0.342128 |
| -2.57073 | -2.35414 | -2.12783 | -1.89909 | -1.67932 | -1.09947 | -0.513252 |
| -2.22057 | -2.04152 | -1.85415 | -1.66691 | -1.48204 | -0.977331 | -0.452621 |
| -2.37001 | -2.13988 | -1.90956 | -1.69387 | -1.48019 | -0.913915 | -0.398848 |
| -4.46842 | -3.98564 | -3.54185 | -3.1035 | -2.72102 | -1.81626 | -0.903885 |
| -3.25403 | -2.84566 | -2.4464 | -2.0997 | -1.8044 | -1.16728 | -0.571152 |
| -2.32335 | -1.99658 | -1.70079 | -1.45184 | -1.24254 | -0.801857 | -0.397084 |
| -3.2263 | -2.76586 | -2.35677 | -2.0129 | -1.72064 | -1.10267 | -0.541228 |
| -3.73681 | -3.30089 | -2.83789 | -2.40935 | -2.05168 | -1.28661 | -0.610992 |
| -4.22894 | -3.73176 | -3.25646 | -2.80231 | -2.39699 | -1.46153 | -0.656402 |
| -3.26919 | -2.86327 | -2.50491 | -2.15452 | -1.84796 | -1.15346 | -0.537135 |
| -4.8138 | -4.36822 | -3.92799 | -3.49415 | -3.00129 | -1.83651 | -0.82139 |
| -4.51275 | -4.02669 | -3.55025 | -3.09602 | -2.6802 | -1.68874 | -0.814062 |
| -3.51962 | -3.1336 | -2.754 | -2.39723 | -2.08529 | -1.35494 | -0.654849 |
| -2.09473 | -1.87875 | -1.66663 | -1.46426 | -1.26245 | -0.809378 | -0.387969 |
| -1.82995 | -1.6407 | -1.45069 | -1.27313 | -1.10512 | -0.684996 | -0.304647 |
| -3.78178 | -3.48079 | -3.17748 | -2.8859 | -2.601 | -1.83227 | -0.907126 |
| -2.89253 | -2.55201 | -2.23198 | -1.94374 | -1.67618 | -1.07374 | -0.477421 |
| -2.70716 | -2.44516 | -2.18889 | -1.94186 | -1.70039 | -1.14455 | -0.541301 |
| -2.88325 | -2.5571 | -2.24842 | -1.96364 | -1.69531 | -1.0781 | -0.480773 |
| -1.70627 | -1.54908 | -1.38092 | -1.20607 | -1.02818 | -0.632355 | -0.277398 |
| -0.569226 | -0.519904 | -0.465936 | -0.409368 | -0.353041 | -0.220606 | -0.0987924 |
| -2.0761 | -1.89657 | -1.72841 | -1.56613 | -1.41414 | -0.979185 | -0.488419 |
| -1.79519 | -1.66546 | -1.53086 | -1.39416 | -1.26371 | -0.912591 | -0.498449 |
| -1.05026 | -0.955359 | -0.86378 | -0.781448 | -0.699728 | -0.461349 | -0.222485 |
| -2.11393 | -1.93009 | -1.74688 | -1.56584 | -1.4031 | -0.95676 | -0.468381 |
| -2.20391 | -2.00318 | -1.79982 | -1.59764 | -1.40645 | -0.912487 | -0.41513 |
| -3.41714 | -3.05282 | -2.70795 | -2.39623 | -2.13169 | -1.39015 | -0.669108 |
| -1.63053 | -1.5075 | -1.31871 | -1.13625 | -0.976265 | -0.591745 | -0.267943 |
| -0.260722 | -0.252062 | -0.242224 | -0.231724 | -0.220701 | -0.180357 | -0.103741 |
| -0.963003 | -0.914543 | -0.858195 | -0.797821 | -0.735217 | -0.545999 | -0.294572 |
| -2.61702 | -2.4038 | -2.19806 | -1.98991 | -1.79289 | -1.27108 | -0.625888 |
| -2.8783 | -2.63971 | -2.40078 | -2.16554 | -1.94848 | -1.36562 | -0.729118 |
| -2.91376 | -2.65326 | -2.37449 | -2.09977 | -1.84204 | -1.20021 | -0.54439 |
| -1.78699 | -1.65722 | -1.52301 | -1.385 | -1.25258 | -0.876721 | -0.41559 |
| -0.789864 | -0.727889 | -0.67042 | -0.613201 | -0.557674 | -0.401989 | -0.219638 |
| -1.9867 | -1.84454 | -1.69908 | -1.55372 | -1.4101 | -1.02801 | -0.563268 |

| | Beta=0.88 | | | | | |
|---|---|---|---|---|---|---|
| -0.0350407 | 1 | -0.149197 | -0.147964 | -0.146641 | -0.145791 | -0.144578 |
| -0.0685096 | 2 | -0.358959 | -0.350938 | -0.344119 | -0.336284 | -0.3261 |
| -0.065603 | 3 | -0.353284 | -0.335098 | -0.318049 | -0.301438 | -0.285784 |
| -0.109908 | 4 | -0.592279 | -0.579638 | -0.565094 | -0.549523 | -0.532477 |
| -0.102395 | 5 | -0.615745 | -0.592166 | -0.567569 | -0.541893 | -0.515867 |
| -0.132646 | 6 | -0.817793 | -0.771462 | -0.728496 | -0.687891 | -0.648765 |
| -0.124978 | 7 | -1.03608 | -0.997574 | -0.954887 | -0.908774 | -0.86345 |
| -0.0556972 | 8 | -0.278995 | -0.273952 | -0.267858 | -0.260737 | -0.253528 |
| -0.075585 | 9 | -0.769975 | -0.720874 | -0.67162 | -0.622277 | -0.57333 |
| -0.0780036 | 10 | -0.909012 | -0.861462 | -0.814601 | -0.767342 | -0.717707 |
| -0.102474 | 11 | -1.45711 | -1.38318 | -1.31228 | -1.2401 | -1.16542 |
| -0.0892962 | 12 | -0.406613 | -0.397324 | -0.387929 | -0.377379 | -0.364794 |
| -0.176936 | 13 | -1.14013 | -1.08139 | -1.0217 | -0.9606 | -0.901782 |
| -0.206621 | 14 | -1.32835 | -1.24928 | -1.17453 | -1.10368 | -1.03705 |
| -0.266181 | 15 | -1.78716 | -1.69324 | -1.60061 | -1.51005 | -1.41879 |
| -0.0829073 | 16 | -0.468313 | -0.451929 | -0.43395 | -0.41599 | -0.39883 |
| -0.369874 | 17 | -1.80665 | -1.71908 | -1.62602 | -1.53366 | -1.4482 |
| -0.0812903 | 18 | -0.553309 | -0.530399 | -0.507177 | -0.480401 | -0.449956 |
| -0.144523 | 19 | -1.01426 | -0.952223 | -0.897922 | -0.847419 | -0.795522 |
| -0.278391 | 20 | -1.17588 | -1.14031 | -1.09966 | -1.05635 | -1.01125 |
| -0.217189 | 21 | -1.19554 | -1.147 | -1.09797 | -1.04736 | -0.997247 |
| -0.322529 | 22 | -1.44598 | -1.38631 | -1.32207 | -1.25755 | -1.19501 |
| -0.338924 | 23 | -1.503 | -1.4394 | -1.37551 | -1.31163 | -1.24923 |

| | | | | | | |
|---|---|---|---|---|---|---|
| -0.112888 | 24 | -4.58213 | -4.09878 | -3.57909 | -3.07029 | -2.60857 |
| -0.131741 | 25 | -4.45098 | -4.01612 | -3.56947 | -3.12942 | -2.70196 |
| -0.370402 | 26 | -5.40147 | -4.98986 | -4.56253 | -4.1495 | -3.7547 |
| -0.118874 | 27 | -4.53618 | -4.06717 | -3.58997 | -3.10315 | -2.64211 |
| -0.235665 | 28 | -5.02762 | -4.61675 | -4.1815 | -3.73101 | -3.2999 |
| -0.188955 | 29 | -4.99106 | -4.52849 | -4.05973 | -3.59135 | -3.14119 |
| -0.0696672 | 30 | -2.23958 | -2.02414 | -1.80642 | -1.58753 | -1.37184 |
| -0.120964 | 31 | -2.3619 | -2.18166 | -1.98934 | -1.79116 | -1.59757 |
| -0.108341 | 32 | -2.03068 | -1.8839 | -1.72682 | -1.56689 | -1.40595 |
| -0.0863096 | 33 | -2.18032 | -1.98628 | -1.78891 | -1.60118 | -1.4119 |
| -0.273812 | 34 | -4.18151 | -3.76079 | -3.36835 | -2.96897 | -2.62117 |
| -0.176326 | 35 | -3.08663 | -2.72155 | -2.357 | -2.03675 | -1.76102 |
| -0.122699 | 36 | -2.23765 | -1.93558 | -1.65883 | -1.42303 | -1.22285 |
| -0.169912 | 37 | -3.07711 | -2.66092 | -2.28454 | -1.96404 | -1.68778 |
| -0.183375 | 38 | -3.55866 | -3.16885 | -2.7461 | -2.34768 | -2.01088 |
| -0.149227 | 39 | -3.9895 | -3.55294 | -3.12668 | -2.71336 | -2.33619 |
| -0.140929 | 40 | -3.10356 | -2.74017 | -2.41637 | -2.09333 | -1.80765 |
| -0.204698 | 41 | -4.4955 | -4.1123 | -3.72649 | -3.34076 | -2.8937 |
| -0.215477 | 42 | -4.23954 | -3.81522 | -3.39192 | -2.98215 | -2.60044 |
| -0.17975 | 43 | -3.31857 | -2.97525 | -2.63361 | -2.30821 | -2.02048 |
| -0.109692 | 44 | -1.95073 | -1.76563 | -1.58042 | -1.40014 | -1.21612 |
| -0.0748203 | 45 | -1.69481 | -1.53471 | -1.37026 | -1.21377 | -1.06268 |
| -0.243908 | 46 | -3.51263 | -3.25506 | -2.992 | -2.73644 | -2.48263 |
| -0.126272 | 47 | -2.72329 | -2.42441 | -2.13852 | -1.8783 | -1.63095 |
| -0.1501 | 48 | -2.54094 | -2.31244 | -2.08598 | -1.8651 | -1.64492 |
| -0.126157 | 49 | -2.70623 | -2.42261 | -2.14921 | -1.89265 | -1.64643 |
| -0.0679467 | 50 | -1.57432 | -1.44448 | -1.30121 | -1.14859 | -0.989536 |
| -0.0249329 | 51 | -0.522562 | -0.482307 | -0.437013 | -0.388149 | -0.338278 |
| -0.14416 | 52 | -1.93531 | -1.78157 | -1.63583 | -1.49296 | -1.35712 |
| -0.140917 | 53 | -1.67468 | -1.56255 | -1.44506 | -1.32405 | -1.20725 |
| -0.0559215 | 54 | -0.962393 | -0.885153 | -0.808553 | -0.738131 | -0.666498 |
| -0.128355 | 55 | -1.95766 | -1.80335 | -1.6467 | -1.48878 | -1.34449 |
| -0.0981623 | 56 | -2.04353 | -1.87285 | -1.69715 | -1.51963 | -1.34867 |
| -0.182657 | 57 | -3.18781 | -2.87163 | -2.56892 | -2.29093 | -2.05199 |
| -0.0818259 | 58 | -1.5258 | -1.41723 | -1.24996 | -1.08641 | -0.941063 |
| -0.0302823 | 59 | -0.234878 | -0.227261 | -0.218969 | -0.2104 | -0.201555 |
| -0.0858885 | 60 | -0.875829 | -0.836812 | -0.790791 | -0.740751 | -0.687997 |
| -0.165816 | 61 | -2.44187 | -2.25798 | -2.07835 | -1.8936 | -1.71702 |
| -0.218159 | 62 | -2.6745 | -2.47109 | -2.26419 | -2.05723 | -1.86357 |
| -0.130282 | 63 | -2.69985 | -2.47904 | -2.23723 | -1.99538 | -1.76468 |
| -0.0866557 | 64 | -1.64506 | -1.5378 | -1.4249 | -1.30639 | -1.19039 |
| -0.0697092 | 65 | -0.744025 | -0.687659 | -0.63525 | -0.583048 | -0.532457 |
| -0.170608 | 66 | -1.84556 | -1.7234 | -1.59707 | -1.46878 | -1.34089 |

| | | |
|---|---|---|
| -0.133785 | -0.0959145 | -0.0345395 |
| -0.279676 | -0.186736 | -0.0676775 |
| -0.245417 | -0.172643 | -0.0646501 |
| -0.466252 | -0.329736 | -0.109159 |
| -0.433785 | -0.277631 | -0.101799 |
| -0.534527 | -0.355731 | -0.13153 |
| -0.73101 | -0.470154 | -0.124975 |
| -0.225557 | -0.152621 | -0.0552802 |
| -0.42765 | -0.24683 | -0.0755241 |
| -0.563275 | -0.291663 | -0.0778799 |
| -0.803733 | -0.368144 | -0.102417 |
| -0.319683 | -0.234484 | -0.0879229 |
| -0.728348 | -0.470585 | -0.176593 |
| -0.831978 | -0.539052 | -0.205724 |
| -1.14499 | -0.766106 | -0.266121 |
| -0.342141 | -0.227455 | -0.0824149 |
| -1.21571 | -0.850801 | -0.367576 |
| -0.355269 | -0.227731 | -0.0809314 |
| -0.622967 | -0.38942 | -0.144233 |
| -0.874423 | -0.645183 | -0.275371 |
| -0.849049 | -0.605773 | -0.215284 |
| -1.02055 | -0.740143 | -0.319854 |
| -1.06456 | -0.765371 | -0.335556 |

| | | |
|---|---|---|
| -1.53399 | -0.570007 | -0.113634 |
| -1.6547 | -0.652966 | -0.133263 |
| -2.66044 | -1.35961 | -0.372537 |
| -1.58712 | -0.602546 | -0.119881 |
| -2.1914 | -0.990381 | -0.23732 |
| -1.96945 | -0.842392 | -0.189724 |
| -0.828876 | -0.341967 | -0.0700205 |
| -1.06984 | -0.510011 | -0.121518 |
| -0.950093 | -0.449891 | -0.108777 |
| -0.893342 | -0.397709 | -0.0871525 |
| -1.78046 | -0.9027 | -0.275414 |
| -1.15253 | -0.571191 | -0.177074 |
| -0.79466 | -0.396726 | -0.123096 |
| -1.0919 | -0.54088 | -0.170037 |
| -1.27438 | -0.611047 | -0.183713 |
| -1.44708 | -0.656922 | -0.150195 |
| -1.14304 | -0.537321 | -0.141679 |
| -1.80707 | -0.821007 | -0.20623 |
| -1.66756 | -0.813546 | -0.216758 |
| -1.33265 | -0.653625 | -0.180789 |
| -0.79389 | -0.387328 | -0.110202 |
| -0.672503 | -0.304114 | -0.0751263 |
| -1.78123 | -0.901728 | -0.245451 |
| -1.06027 | -0.477638 | -0.126788 |
| -1.125 | -0.540082 | -0.150838 |
| -1.06398 | -0.481003 | -0.127033 |
| -0.621454 | -0.276642 | -0.06809 |
| -0.216148 | -0.098407 | -0.0249386 |
| -0.956505 | -0.485717 | -0.144543 |
| -0.885979 | -0.492968 | -0.141235 |
| -0.449347 | -0.220801 | -0.0561331 |
| -0.934937 | -0.465938 | -0.128827 |
| -0.892076 | -0.413063 | -0.0985302 |
| -1.36338 | -0.667551 | -0.183779 |
| -0.581356 | -0.266627 | -0.0813057 |
| -0.168522 | -0.100666 | -0.0301195 |
| -0.522305 | -0.28918 | -0.0858644 |
| -1.23818 | -0.62204 | -0.166557 |
| -1.32977 | -0.724472 | -0.218944 |
| -1.17337 | -0.542399 | -0.130897 |
| -0.849619 | -0.412481 | -0.0872004 |
| -0.389578 | -0.217134 | -0.0698667 |
| -0.993728 | -0.556012 | -0.170973 |
