# Supplementary material for: Accurate Deep Learning-aided Density-free Strategy for Many-Body Dispersion-corrected Density Functional Theory
Source: arXiv:2203.15739 ancillary file (2022-05-06)
Supplement: Supplementary file 2 [file SI-ML_MBD3.pdf]

# PBE-PCSEG3

| Dimer nr | monomer A | Monomer B |
|---|---|---|
| 1 | -232.038714 | -232.038718 |
| 2 | -232.038724 | -363.519798 |
| 3 | -307.232303 | -307.232303 |
| 4 | -56.5168897 | -56.5168897 |
| 5 | -76.3881841 | -76.3881567 |
| 6 | -232.038705 | -40.4677527 |
| 7 | -189.659476 | -189.659476 |
| 8 | -169.79182 | -169.79182 |
| 9 | -414.561881 | -414.561881 |
| 10 | -323.287393 | -303.41504 |
| 11 | -467.004479 | -453.841366 |
| 12 | -40.4678697 | -40.4678697 |
| 13 | -78.5080738 | -78.5080738 |
| 14 | -232.038707 | -232.038707 |
| 15 | -264.113297 | -264.113299 |
| 16 | -414.562421 | -414.562421 |
| 17 | -232.03875 | -363.519706 |
| 18 | -467.003908 | -453.842007 |
| 19 | -78.5080654 | -77.2584919 |
| 20 | -232.038714 | -76.3881334 |
| 21 | -232.038709 | -56.5167987 |
| 22 | -232.038721 | -93.3541182 |

| Dimer nr | x1 |
|---|---|
| 1 | -4[illegible] |
| 2 | -59[illegible] |
| 3 | -61[illegible] |
| 4 | -1[illegible] |
| 5 | -15[illegible] |
| 6 | -272.506409 |
| 7 | -379.348139 |
| 8 | -339.607366 |
| 9 | -829.153617 |
| 10 | -626.72704 |
| 11 | -920.868925 |
| 12 | -80.9358788 |
| 13 | -157.01664 |
| 14 | -464.074561 |
| 15 | -528.225317 |
| 16 | -829.129657 |
| 17 | -595.554639 |
| 18 | -920.847907 |
| 19 | -155.768443 |
| 20 | -308.43026 |
| 21 | -288.557182 |
| 22 | -325.397363 |

Total PBE PCSEG-3 energies (Hartree) f[illegible] dimes with MBD

Hartree-to-kcalmol
627.5094736

for the
ıout

| Dimer nr | x1 |
|---|---|
| 1 | -0.08250036 |
| 2 | -2.04678863 |
| 3 | -3.68264841 |
| 4 | -2.81836769 |
| 5 | -5.01913227 |
| 6 | 0.030985226 |
| 7 | -18.3153395 |
| 8 | -14.8877757 |
| 9 | -18.7337017 |
| 10 | -15.4413538 |
| 11 | -14.4829426 |
| 12 | -0.08748028 |
| 13 | -0.30907364 |
| 14 | 1.789721966 |
| 15 | 0.803168954 |
| 16 | -3.02165453 |
| 17 | 2.395548979 |
| 18 | -1.24981376 |
| 19 | -1.18311433 |
| 20 | -2.14170445 |
| 21 | -1.05070243 |
| 22 | -2.83896688 |

| Dimer nr | monomer A | Monomer B |
|---|---|---|
| 1 | -232.046551 | -232.046554 |
| 2 | -232.046479 | -363.53295 |
| 3 | -307.24089 | -307.24089 |
| 4 | -56.517379 | -56.517379 |
| 5 | -76.3884381 | -76.3883948 |
| 6 | -232.046524 | -40.46871112 |
| 7 | -189.660656 | -189.660656 |
| 8 | -169.793508 | -169.793508 |
| 9 | -414.570169 | -414.570169 |
| 10 | -323.295393 | -303.423704 |
| 11 | -467.016463 | -453.852507 |
| 12 | -40.4688293 | -40.4688293 |
| 13 | -78.5097023 | -78.5097023 |
| 14 | -232.046527 | -232.046527 |
| 15 | -264.119117 | -264.119192 |
| 16 | -414.570668 | -414.570668 |
| 17 | -232.046453 | -363.532948 |
| 18 | -467.01594 | -453.8531161 |
| 19 | -78.5096606 | -77.2592884 |
| 20 | -232.046559 | -76.3883852 |
| 21 | -232.046587 | -56.5173079 |
| 22 | -232.046562 | -93.3545456 |

| Dimer nr | x1 |
|---|---|
| 1 | [illegible] |
| 2 | [illegible] |
| 3 | [illegible] |
| 4 | [illegible] |
| 5 | [illegible] |
| 6 | -272.51753 |
| 7 | -379.352849 |
| 8 | -339.61328 |
| 9 | -829.173723 |
| 10 | -626.747955 |
| 11 | -920.896832 |
| 12 | -80.9386635 |
| 13 | -157.022096 |
| 14 | -464.096606 |
| 15 | -528.243377 |
| 16 | -829.155214 |
| 17 | -595.584915 |
| 18 | -920.884167 |
| 19 | -155.771909 |
| 20 | -308.440496 |
| 21 | -288.567709 |
| 22 | -325.408291 |

Total PBE PCSEG-3 energies (Hartree) f dimes with MBD

Hartree-to-kcalmol
627.5094736

for the
iout

| Dimer nr | x1 |
|---|---|
| 1 | -2.50029895 |
| 2 | -5.47999003 |
| 3 | -6.88665292 |
| 4 | -3.39812068 |
| 5 | -5.43593887 |
| 6 | -1.43996481 |
| 7 | -19.7898227 |
| 8 | -16.4808712 |
| 9 | -20.9490586 |
| 10 | -18.108888 |
| 11 | -17.4839325 |
| 12 | -0.63059682 |
| 13 | -1.68911118 |
| 14 | -2.22913955 |
| 15 | -3.18058197 |
| 16 | -8.70895926 |
| 17 | -3.45981113 |
| 18 | -9.48242116 |
| 19 | -1.85733392 |
| 20 | -3.48372552 |
| 21 | -2.39354704 |
| 22 | -4.50811591 |

| Dimer nr | monomer A | Monomer B |
|---|---|---|
| 1 | -232.061203 | -232.061195 |
| 2 | -232.061122 | -363.54491 |
| 3 | -307.248965 | -307.248965 |
| 4 | -56.5208046 | -56.5208046 |
| 5 | -76.3873036 | -76.3873423 |
| 6 | -232.061221 | -40.4784208 |
| 7 | -189.651293 | -189.651293 |
| 8 | -169.788817 | -169.788817 |
| 9 | -414.557357 | -414.557357 |
| 10 | -323.29392 | -303.429302 |
| 11 | -467.00704 | -453.84414 |
| 12 | -40.4784349 | -40.4784349 |
| 13 | -78.5186231 | -78.5186231 |
| 14 | -232.061215 | -232.061215 |
| 15 | -264.119163 | -264.11915 |
| 16 | -414.558134 | -414.558134 |
| 17 | -232.061207 | -363.544884 |
| 18 | -467.006471 | -453.845214 |
| 19 | -78.5186126 | -77.261794 |
| 20 | -232.06117 | -76.3872353 |
| 21 | -232.061196 | -56.5207316 |
| 22 | -232.061145 | -93.350105 |

| Dimer nr | x1 |
|---|---|
| 1 | -464.122815 |
| 2 | -595.609871 |
| 3 | -614.504391 |
| 4 | -113.045977 |
| 5 | -152.782621 |
| 6 | -272.539675 |
| 7 | -379.332979 |
| 8 | -339.602245 |
| 9 | -829.14568 |
| 10 | -626.747983 |
| 11 | -920.87463 |
| 12 | -80.9569257 |
| 13 | -157.037788 |
| 14 | -464.119625 |
| 15 | -528.237305 |
| 16 | -829.121903 |
| 17 | -595.602574 |
| 18 | -920.854794 |
| 19 | -155.782309 |
| 20 | -308.452032 |
| 21 | -288.583707 |
| 22 | -325.416485 |

Hartree-to-kcalmol
627.5094736

| Dimer nr | x1 |
|---|---|
| 1 | -0.26222642 |
| 2 | -2.40922429 |
| 3 | -4.05443767 |
| 4 | -2.74088357 |
| 5 | -5.00427855 |
| 6 | -0.020942 |
| 7 | -19.071564 |
| 8 | -15.443059 |
| 9 | -19.4306667 |
| 10 | -15.5378309 |
| 11 | -14.7149931 |
| 12 | -0.03504747 |
| 13 | -0.34001971 |
| 14 | 1.759363183 |
| 15 | 0.632466234 |
| 16 | -3.5357864 |
| 17 | 2.20682494 |
| 18 | -1.95103024 |
| 19 | -1.19372206 |
| 20 | -2.27552725 |
| 21 | -1.11659331 |
| 22 | -3.28509329 |

PBE0-PCSEG3_QCHEMMBD

| Dimer nr | monomer A | Monomer B |
|---|---|---|
| 1 | -232.068115 | -232.068106 |
| 2 | -232.06796 | -363.556636 |
| 3 | -307.256552 | -307.256552 |
| 4 | -56.5212326 | -56.5212326 |
| 5 | -76.3875285 | -76.3875532 |
| 6 | -232.068117 | -40.479247 |
| 7 | -189.652314 | -189.652314 |
| 8 | -169.790286 | -169.790286 |
| 9 | -414.564653 | -414.564653 |
| 10 | -323.300973 | -303.436956 |
| 11 | -467.017679 | -453.854014 |
| 12 | -40.4792619 | -40.4792619 |
| 13 | -78.5200452 | -78.5200452 |
| 14 | -232.068104 | -232.068104 |
| 15 | -264.124266 | -264.124306 |
| 16 | -414.565398 | -414.565398 |
| 17 | -232.068013 | -363.556681 |
| 18 | -467.017145 | -453.855059 |
| 19 | -78.5200089 | -77.2624955 |
| 20 | -232.068077 | -76.3874585 |
| 21 | -232.068129 | -56.52117503 |
| 22 | -232.068059 | -93.3504816 |

| Dimer nr | x1 |
|---|---|
| 1 | -464.140411 |
| 2 | -595.633732 |
| 3 | -614.524428 |
| 4 | -113.047676 |
| 5 | -152.783656 |
| 6 | -272.549671 |
| 7 | -379.337167 |
| 8 | -339.607531 |
| 9 | -829.163638 |
| 10 | -626.766755 |
| 11 | -920.899698 |
| 12 | -80.9594335 |
| 13 | -157.042717 |
| 14 | -464.139722 |
| 15 | -528.253743 |
| 16 | -829.145166 |
| 17 | -595.630315 |
| 18 | -920.888132 |
| 19 | -155.785444 |
| 20 | -308.461211 |
| 21 | -288.593168 |
| 22 | -325.426302 |

Hartree-to-kcalmol
627.5094736

1
2
3
4
5
6
7
8
9
10
11
12
13
14
15
16
17

18
19
20
21
22

| Dimer nr | x1 |
|---|---|
| 1 | -2.62982945 |
| 2 | -5.7328136 |
| 3 | -7.10526467 |
| 4 | -3.27005227 |
| 5 | -5.3803227 |
| 6 | -1.44772083 |
| 7 | -20.4184115 |
| 8 | -16.9171597 |
| 9 | -21.5434984 |
| 10 | -18.0882555 |
| 11 | -17.573453 |
| 12 | -0.57092067 |
| 13 | -1.64815363 |
| 14 | -2.20504946 |
| 15 | -3.24450636 |
| 16 | -9.01764372 |
| 17 | -3.52718055 |
| 18 | -9.995498 |
| 19 | -1.8444386 |
| 20 | -3.56143629 |
| 21 | -2.42461503 |
| 22 | -4.87077873 |

1
2
3
4
5
6
7
8
9
10
11
12

13
14
15
16
17
18
19
20
21
22

REFERENCE CCSD(T) interaction energy

| Dimer nr | kcal/mol |
|---|---|
| 1 | -2.71 |
| 2 | -5.62 |
| 3 | -7.09 |
| 4 | -3.17 |
| 5 | -5.02 |
| 6 | -1.45 |
| 7 | -18.8 |
| 8 | -16.12 |
| 9 | -20.69 |
| 10 | -17 |
| 11 | -16.74 |
| 12 | -0.53 |
| 13 | -1.5 |
| 14 | -2.62 |
| 15 | -4.2 |
| 16 | -9.74 |
| 17 | -4.59 |
| 18 | -11.66 |
| 19 | -1.51 |
| 20 | -3.29 |
| 21 | -2.32 |
| 22 | -4.55 |

| new number | original structure name |
|---|---|
| 1 | 100_BenzenedimerTshaped. |
| 2 | 101_IndolebenzeneTshapec |
| 3 | 102_Phenoldimer.xyz |
| 4 | 81_Ammoniadimer.xyz |
| 5 | 82_Waterdimer.xyz |
| 6 | 83_BenzeneMethanecomple |
| 7 | 84_Formicaciddimer.xyz |
| 8 | 85_Formamidedimer.xyz |
| 9 | 86_Uracildimerhbonded.xyz |
| 10 | 87_2pyridoxine2aminopyridi |
| 11 | 88_AdeninethymineWatsonC |
| 12 | 89_Methanedimer.xyz |
| 13 | 90_Ethenedimer.xyz |
| 14 | 91_Benzenedimerparalleldis |
| 15 | 92_Pyrazinedimer.xyz |
| 16 | 93_Uracildimerstack.xyz |
| 17 | 94_Indolebenzenecomplexst |
| 18 | 95_Adeninethyminecomplex |
| 19 | 96_Etheneethynecomplex.xy |
| 20 | 97_Benzenewatercomplex.x |
| 21 | 98_Benzeneammoniacomple |
| 22 | 99_BenzeneHCNcomplex.xy |

~

.xyz
omplex.xyz

ex.xyz

necomplex.xyz
Crickcomplex.xyz

placed.xyz

tack.xyz
stack.xyz
yz
yz
ex.xyz
yz

| Beta=0.76 | | | |
|---|---|---|---|
| mbd_dimer | Beta=0.76 | mbd monomer A +B | |
| 1 | -16.9263607 | 1 | -14.4786555 |
| 2 | -22.8993651 | 2 | -19.5625873 |
| 3 | -18.7538691 | 3 | -16.062561 |
| 4 | -1.09623511 | 4 | -0.69337355 |
| 5 | -0.68523066 | 5 | -0.37201862 |
| 6 | -9.48988557 | 6 | -8.12157042 |
| 7 | -3.68532796 | 7 | -2.07293427 |
| 8 | -4.09790035 | 8 | -2.48913161 |
| 9 | -16.4155708 | 9 | -14.1186854 |
| 10 | -17.4360219 | 10 | -14.759923 |
| 11 | -23.3656522 | 11 | -20.2979638 |
| 12 | -2.26274337 | 12 | -1.75656447 |
| 13 | -3.85669821 | 13 | -2.62331678 |
| 14 | -19.0270866 | 14 | -14.4822614 |
| 15 | -15.9412982 | 15 | -11.4266054 |
| 16 | -20.3116687 | 16 | -14.0881801 |
| 17 | -26.0837716 | 17 | -19.5708566 |
| 18 | -29.2747017 | 18 | -20.2948723 |
| 19 | -2.62889384 | 19 | -1.98588287 |
| 20 | -8.53367577 | 20 | -7.42831598 |
| 21 | -8.80069702 | 21 | -7.59642665 |
| 22 | -9.45179961 | 22 | -7.63568216 |

| Beta=0.75 | | | |
|---|---|---|---|
| mbd_dimer | Beta=0.75 | mbd monomer A +B | |
| 1 | -18.0560245 | 1 | -15.5922016 |
| 2 | -24.3620473 | 2 | -20.9814959 |
| 3 | -19.9834472 | 3 | -17.2414375 |
| 4 | -1.15052723 | 4 | -0.7237893 |
| 5 | -0.72776258 | 5 | -0.39378604 |
| 6 | -10.107337 | 6 | -8.7175351 |
| 7 | -3.92987861 | 7 | -2.24711682 |
| 8 | -4.35579326 | 8 | -2.67627454 |
| 9 | -17.4624477 | 9 | -15.0970762 |
| 10 | -18.5848179 | 10 | -15.8329162 |
| 11 | -24.8644954 | 11 | -21.7089543 |
| 12 | -2.35494189 | 12 | -1.83458966 |
| 13 | -4.06693371 | 13 | -2.81322744 |
| 14 | -20.1930927 | 14 | -15.5961622 |
| 15 | -16.9056409 | 15 | -12.3254844 |
| 16 | -21.4049974 | 16 | -15.0632308 |
| 17 | -27.5943209 | 17 | -20.9912064 |
| 18 | -30.8592471 | 18 | -21.7006472 |
| 19 | -2.78567298 | 19 | -2.12935946 |
| 20 | -9.12106147 | 20 | -7.99628509 |
| 21 | -9.39410418 | 21 | -8.16891795 |

| | | | |
|---|---|---|---|
| 22 | -10.0725472 | 22 | -8.22110266 |

| | Beta=0.78 | |
|---|---|---|
| Inter energy MBD crrection | mbd_dimer | Beta=0.78 |
| -2.44770522 | 1 | -14.9058268 |
| -3.33677774 | 2 | -20.283342 |
| -2.69130808 | 3 | -16.5386322 |
| -0.40286155 | 4 | -0.99554312 |
| -0.31321204 | 5 | -0.6074779 |
| -1.36831515 | 6 | -8.38962766 |
| -1.61239369 | 7 | -3.24778696 |
| -1.60876874 | 8 | -3.64013794 |
| -2.29688539 | 9 | -14.5344559 |
| -2.67609897 | 10 | -15.3760472 |
| -3.06768841 | 11 | -20.6729064 |
| -0.5061789 | 12 | -2.08582816 |
| -1.23338142 | 13 | -3.47110983 |
| -4.54482512 | 14 | -16.929786 |
| -4.51469281 | 15 | -14.1935674 |
| -6.22348865 | 16 | -18.3119019 |
| -6.51291499 | 17 | -23.3569535 |
| -8.97982942 | 18 | -26.389584 |
| -0.64301097 | 19 | -2.34884225 |
| -1.10535979 | 20 | -7.48775495 |
| -1.20427037 | 21 | -7.73828805 |
| -1.81611746 | 22 | -8.34006362 |

| | Beta=0.77 | |
|---|---|---|
| Inter energy MBD crrection | mbd_dimer | Beta=0.77 |
| -2.46382284 | 1 | -15.8750563 |
| -3.38055137 | 2 | -21.5487959 |
| -2.74200967 | 3 | -17.5977829 |
| -0.42673793 | 4 | -1.04417786 |
| -0.33397654 | 5 | -0.64476803 |
| -1.38980193 | 6 | -8.92394757 |
| -1.68276179 | 7 | -3.45898536 |
| -1.67951872 | 8 | -3.86378925 |
| -2.36537147 | 9 | -15.4445576 |
| -2.7519017 | 10 | -16.3697751 |
| -3.1555411 | 11 | -21.9712373 |
| -0.52035223 | 12 | -2.17273824 |
| -1.25370627 | 13 | -3.65677185 |
| -4.59693047 | 14 | -17.9399559 |
| -4.58015652 | 15 | -15.0287304 |
| -6.34176662 | 16 | -19.2826379 |
| -6.60311451 | 17 | -24.6799388 |
| -9.15859987 | 18 | -27.7925576 |
| -0.65631351 | 19 | -2.48625022 |
| -1.12477638 | 20 | -7.99366988 |
| -1.22518622 | 21 | -8.24973047 |

| | | |
|---|---|---|
| -1.85144457 | 22 | -8.87692893 |

| | mbd monomer A +B | Inter energy M |
|---|---|---|
| 1 | -12.5107259 | -2.39510096 |
| 2 | -17.0411517 | -3.24219039 |
| 3 | -13.9431766 | -2.59545563 |
| 4 | -0.63764113 | -0.35790199 |
| 5 | -0.33221545 | -0.27526244 |
| 6 | -7.06327136 | -1.32635631 |
| 7 | -1.77072063 | -1.47706633 |
| 8 | -2.16273528 | -1.47740265 |
| 9 | -12.3657619 | -2.16869395 |
| 10 | -12.846712 | -2.52933522 |
| 11 | -17.7748624 | -2.89804396 |
| 12 | -1.60856851 | -0.47725965 |
| 13 | -2.28389184 | -1.18721799 |
| 14 | -12.5137604 | -4.41602553 |
| 15 | -9.82977048 | -4.36379688 |
| 16 | -12.3408092 | -5.97109276 |
| 17 | -17.0487254 | -6.30822816 |
| 18 | -17.7711255 | -8.61845846 |
| 19 | -1.7298935 | -0.61894876 |
| 20 | -6.4237686 | -1.06398634 |
| 21 | -6.58347102 | -1.15481703 |
| 22 | -6.60058061 | -1.73948302 |

| | mbd monomer A +B | Inter energy M |
|---|---|---|
| 1 | -13.4590368 | -2.41601953 |
| 2 | -18.2580763 | -3.29071961 |
| 3 | -14.9550534 | -2.64272953 |
| 4 | -0.66479563 | -0.37938223 |
| 5 | -0.35145591 | -0.29331213 |
| 6 | -7.57386502 | -1.35008255 |
| 7 | -1.91613171 | -1.54285365 |
| 8 | -2.32010074 | -1.54368851 |
| 9 | -13.2115504 | -2.23300723 |
| 10 | -13.768108 | -2.60166711 |
| 11 | -18.9885005 | -2.98273677 |
| 12 | -1.68111628 | -0.49162196 |
| 13 | -2.44623342 | -1.21053843 |
| 14 | -13.462338 | -4.47761795 |
| 15 | -10.5906386 | -4.43809181 |
| 16 | -13.1839678 | -6.09867013 |
| 17 | -18.2663691 | -6.41356974 |
| 18 | -18.9815933 | -8.81096432 |
| 19 | -1.85298965 | -0.63326057 |
| 20 | -6.90785348 | -1.0858164 |
| 21 | -7.07175048 | -1.17797998 |

mbd_correction

| | | |
|---|---|---|
| 22 | -7.09924458 | -1.77768435 |

IBD crrection

IBD crrection
